# Supplementary material for: Upper security bounds for coherent-one-way quantum key distribution
Source: arXiv:2006.16891 ancillary file (2021-01-04)
Supplement: Supplementary file 1 [file SM_COW_MC111220.pdf]

# Supplemental Material: Upper security bounds for coherent-one-way quantum key distribution

Javier González-Payo,[1] Róbert Trényi,[1] Weilong Wang,[1, 2, 3] and Marcos Curty[1]

[1]*Escuela de Ingeniería de Telecomunicación, Department of Signal Theory and Communications, University of Vigo, Vigo E-36310, Spain*
[2]*State Key Laboratory of Mathematical Engineering and Advanced Computing, Zhengzhou, Henan, 450001, China*
[3]*Henan Key Laboratory of Network Cryptography Technology, Zhengzhou, Henan, 450001, China*

This Supplemental Material has the following structure. In Section I, we describe Eve's sequential attack in detail including all the parameters that she can tune while applying the attack. Then, in Section II, we define the optimization problem that we solve to obtain Eve's measurement operators. In Sections III, IV and V we derive the analytical formulas for evaluating the gain, the quantum bit error rate (QBER) and the visibilities, respectively, which are achievable with the attack. In Section VI, we describe the technical details of the experiments that we compare to, and we provide the parameters of the attack which deliver the results shown in Fig. 2 in the main text. In Section VII, we compare the attack with the upper bound against collective attacks presented in [1], while in Section VIII we compare it with the upper bound derived in [2] by using quantum filtering operations. Next, in Section IX, we describe how the ultimate upper bound on the secret key rate of the COW protocol, illustrated in Fig. 3 of the main text, has been obtained. And, finally, in Section X we analyze briefly the security of a related protocol—so-called differential-phase-shift QKD—and show how sequential attacks could also be used to derive upper bounds on its secret key rate.

## I. DESCRIPTION OF THE ATTACK

As mentioned in the main text, Eve's attack is a special type of intercept-resend attack, a so-called sequential attack [3–7], where she measures each signal emitted by Alice at a location very close to the sender. When Eve obtains a predetermined number of consecutive conclusive measurement outcomes, she prepares a new sequence of signals, which depends on her measurement outcomes, and she sends it to Bob. Otherwise, Eve just sends vacuum signals to Bob to avoid errors. Upon measuring a signal emitted by Alice, there are two possibilities for Eve: she can obtain a conclusive or an inconclusive result. In the former case, a conclusive outcome can either correctly identify the sent signal or be an error, while in the latter case, an inconclusive result provides Eve no information on the sent signal. Precisely, the attack consists of the following steps:

(i) Eve first measures the signals from Alice one by one and counts the number of consecutive conclusive outcomes, denoted as $S$.

(ii) If $S < M_{\min}$, where $M_{\min}$ is the (predetermined) minimum size of the block that Eve can resend, Eve just resends $S$ vacuum signals to Bob.

(iii) If $S = M_{\min}$, Eve decides with probability $q$ to process the block before resending it (see steps (vi), (vii) and (viii) below), or with probability $1-q$ she resends a block of $S$ vacuum signals to Bob.

(iv) If $M_{\min} < S < M_{\max}$, where $M_{\max}$ is the (predetermined) maximum size of the block that Eve can resend, Eve processes the block before resending it. We note that in principle $M_{\max}$ can be arbitrarily large.

(v) Whenever $S$ reaches $M_{\max}$, Eve does not measure the next signal but automatically replaces it with a vacuum signal. Also, she processes the block before resending it, and she restarts the counting of the conclusive results.

Processing a block consists of the following steps:

(vi) If the first result of the block is the bit 1 signal $|\alpha\rangle|0\rangle$ and the last result is the bit 0 signal $|0\rangle|\alpha\rangle$ (which we shall call the "0...1" structure), Eve resends Bob a block encoded in the same way as the measurement outcomes she obtained but using coherent states with mean photon number $|\beta|^2$.

(vii) If the block does not start with the bit 1 signal and/or does not end with the bit 0 signal, then with probability $q_{\rm p}$ Eve tries to cut it from the left, right or both sides until finding a sub-block starting with the bit 1 signal and ending with the bit 0 signal while keeping the length of the sub-block no smaller than $M_{\min}$, or with probability $1-q_{\rm p}$ she resends it encoded just in the same way as the measurement outcomes she obtained but using coherent states with mean photon number $|\beta|^2$.

(viii) If Eve can successfully cut the block in the previous step, then she resends Bob the sub-block with the "0...1" structure encoded using coherent states with mean photon number $|\beta|^2$ and vacuum signals at the positions where the original signals were cut. Else, Eve resends Bob the block as a sequence of vacuum signals.

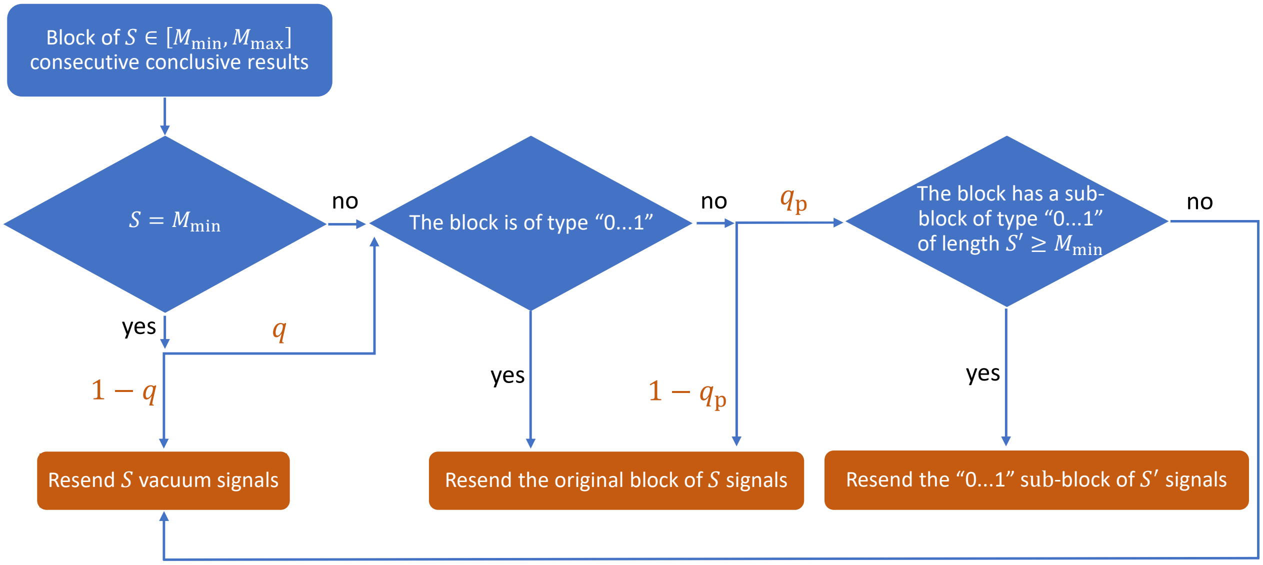


FIG. 1. Flowchart of the attack. The positive integer $S$ is the block size of consecutive conclusive measurement outcomes obtained by Eve. The quantity $M_{\min}$ ($M_{\max}$) is the minimum (maximum) size of a block to be resent to Bob. The probability to resend vacuum signals when $S = M_{\min}$ is $1-q$. The quantity $q_\mathrm{p}$ is the probability to process a block, whose size belongs to the interval $[M_{\min}, M_{\max}]$, and the first result of the block is not the bit 1 signal $|\alpha\rangle\,|0\rangle$ and/or the last result of the block is not the bit 0 signal $|0\rangle\,|\alpha\rangle$. When the first (last) result of the block is the bit 1 (0) signal, we say it has "0...1" structure.

For clarity, the steps of the attack are illustrated by the flowchart in Fig. 1. As a result of the attack, Eve sends Bob blocks of length $S \in [M_{\min}, M_{\max}]$ consisting of signals corresponding to her measurement results, separated by vacuum signals. The parameters over which Eve has control are $M_{\min}$, $M_{\max}$, $q$, $q_\mathrm{p}$ and $\beta$.

## II. EVE'S MEASUREMENT

Eve's measurement is described by a positive-operator-valued measure (POVM) which contains four elements $E_j \geq 0$, with $j = 0, \ldots, 3$, that satisfy $\sum_{j=0}^{3} E_j = \mathbb{1}$, where the symbol $\mathbb{1}$ represents the identity operator.

Let $|\varphi_i\rangle$, with $i = 0, \ldots, 2$, represent each of the three possible signals prepared by Alice in the COW protocol, *i.e.*,

$$\begin{aligned} |\varphi_0\rangle &\equiv |0\rangle\,|\alpha\rangle\,, \\ |\varphi_1\rangle &\equiv |\alpha\rangle\,|0\rangle\,, \\ |\varphi_2\rangle &\equiv |\alpha\rangle\,|\alpha\rangle\,. \end{aligned} \tag{1}$$

The conditional probability of obtaining a measurement result associated with the operator $E_j$, when Eve measures the state $|\varphi_i\rangle$ with the POVM $\{E_j\}_{j=0,\ldots,3}$, is given by

$$p_{j|i} = \langle\varphi_i|\, E_j\, |\varphi_i\rangle\,. \tag{2}$$

In what follows, we shall assume that whenever Eve obtains a measurement result associated with the POVM element $E_i$, she considers that the input state is $|\varphi_i\rangle$. That is, $p_{i|i}$ is the conditional probability that Eve correctly identifies the state $|\varphi_i\rangle$. If Eve obtains a measurement result associated with $E_3$ then she considers it an inconclusive result.

| | Eve's POVM elements | | | |
|---|---|---|---|---|
| Alice's signal | $E_0$ | $E_1$ | $E_2$ | $E_3$ |
| $\vert\varphi_0\rangle$ | $q_\mathrm{s}$ | $q_\mathrm{f}$ | $q_\mathrm{f}$ | $q_\mathrm{inc}$ |
| $\vert\varphi_1\rangle$ | $q_\mathrm{f}$ | $q_\mathrm{s}$ | $q_\mathrm{f}$ | $q_\mathrm{inc}$ |
| $\vert\varphi_2\rangle$ | $q_\mathrm{f}$ | $q_\mathrm{f}$ | $q_\mathrm{s}$ | $q_\mathrm{inc}$ |

TABLE I. Symmetry conditions imposed on the probabilities of Eve's measurement results. Those results associated with the POVM element $E_3$ are considered inconclusive.

For convenience, below we shall impose that the probabilities $p_{j|i}$ of Eve's measurement results satisfy the symmetry conditions shown in Table I. That is, we impose that

$$\begin{aligned} &p_{0|0} = p_{1|1} = p_{2|2} \equiv q_\mathrm{s}, \\ &p_{3|0} = p_{3|1} = p_{3|2} \equiv q_\mathrm{inc}, \\ &p_{1|0} = p_{2|0} = p_{0|1} = p_{2|1} = p_{0|2} = p_{1|2} \equiv q_\mathrm{f}. \end{aligned} \tag{3}$$

The first (second) condition indicates that each state $|\varphi_i\rangle$ has the same probability of being correctly identified by Eve (of producing an inconclusive result). The third condition states that if Eve obtains a conclusive but incorrect result when measuring the state $|\varphi_i\rangle$, with $i = 0, \ldots, 2$, then all states $|\varphi_j\rangle$, with $j \neq i$, are equally likely of being the outcome result of the measurement.

As already mentioned in the main text, the probability of obtaining an inconclusive result, expected gain at

Bob's side. Then, for a given value of $q_{\rm inc}$, Eve selects a POVM, $\{E_j\}_{j=0,\ldots,3}$, that maximizes her probability, $q_{\rm s}$, of correctly discriminating the states $|\varphi_i\rangle$. This can be done by solving the following semidefinite program (SDP) [8, 9]:

$$\begin{aligned} &\text{maximize} \quad p_{0|0} \\ &\text{s. t.} \quad \sum_{j=0}^{3} E_j = \mathbb{1},\ E_j \geq 0 \ \ \forall j=0,\ldots,3, \\ &\qquad p_{0|0} = p_{1|1} = p_{2|2}, \\ &\qquad p_{3|0} = p_{3|1} = p_{3|2} = q_{\rm inc}, \\ &\qquad p_{1|0} = p_{2|0} = p_{0|1} = p_{2|1} = p_{0|2} = p_{1|2}. \end{aligned} \tag{4}$$

Note that in this equation we have used the fact that $p_{0|0} = p_{1|1} = p_{2|2} = q_{\rm s}$ to write the objective function.

SDPs are convex optimization problems that can be solved efficiently in polynomial time, for instance by means of interior-point methods, and they are guaranteed to converge to the global optimum. Any SDP can be rewritten in the following form:

$$\begin{aligned} &\text{maximize} \quad -c^T \mathbf{x} \\ &\text{subject to} \quad F(\mathbf{x}) = F_0 + \sum_i x_i F_i \geq 0, \end{aligned} \tag{5}$$

where the vector $\mathbf{x} = (x_1,\ldots,x_n)^T$ denotes the objective variable, the vector $c$ is fixed by the particular optimization problem, and the matrices $F_0$ and $F_i$ are Hermitian matrices also fixed by the particular optimization problem.

Importantly, as already mentioned in the main text, the solution given by the SDP of Eq. (4) resembles the intermediate measurement strategy introduced in [10, 11]. To be precise, it lies between the MED [12, 13] and the USD regime [14–16]. That is, if $q_{\rm inc} = 0$, the solution to Eq. (4) coincides with the optimal MED result in a scenario where we impose the conditions given by Eq. (3). Also, whenever $q_{\rm inc} \geq q_{\rm usd}$ then $q_{\rm f} = 0$, *i.e.*, the solution to Eq. (4) coincides with the optimal USD solution in a scenario where we impose Eq. (3), where $q_{\rm usd}$ is the failure probability of this latter measurement.

### A. Semidefinite program and searching for $q_{\rm s}$ and $q_{\rm f}$

In this section, we show how to write the SDP given by Eq. (4) in the form given by Eq. (5), which can be easily solved numerically, for instance by using the freely available solvers SDPT3-4.0 [17] and Sedumi [18], together with the input tool YALMIP [19].

For this, we first parametrize the states $|\varphi_i\rangle$, together with the operators $E_j$, in a convenient form. In particular, we express Alice's coherent states $|\varphi_i\rangle$ in some orthonormal basis $\{|b_0\rangle, |b_1\rangle, |b_2\rangle\}$ of a three-dimensional Hilbert space $\mathcal{H}_3$ as follows,

$$\begin{aligned} |\varphi_0\rangle &= |b_0\rangle, \\ |\varphi_1\rangle &= e^{-|\alpha|^2} |b_0\rangle + \sqrt{1-e^{-2|\alpha|^2}}\, |b_1\rangle, \\ |\varphi_2\rangle &= e^{-\frac{|\alpha|^2}{2}} |b_0\rangle + e^{-\frac{|\alpha|^2}{2}} \frac{1-e^{-|\alpha|^2}}{\sqrt{1-e^{-2|\alpha|^2}}} |b_1\rangle \\ &\quad + \frac{1-e^{-|\alpha|^2}}{\sqrt{1-e^{-2|\alpha|^2}}} |b_2\rangle, \end{aligned} \tag{6}$$

with $\langle b_i | b_j\rangle = \delta_{ij}$, where $\delta_{ij}$ represents the Kronecker delta. This implies that we can restrict ourselves to operators $E_j$ that act on $\mathcal{H}_3$.

Next, we rewrite both $\rho_i = |\varphi_i\rangle\langle\varphi_i|$ and $E_j$ acting on $\mathcal{H}_3$ in terms of the Gell-Mann operators, which we shall denote as $\{\sigma_k\}_{k=0}^{8}$. These are Hermitian matrices that form an operator basis in $\mathcal{H}_3$ and satisfy the following two conditions: $\text{Tr}(\sigma_k) = 3\delta_{k0}$ and $\text{Tr}(\sigma_k\sigma_l) = 3\delta_{kl}$, where $\delta_{kl}$ represents again the Kronecker delta. With this representation, we have that $\rho_i$ and $E_j$ can be expressed, respectively, as

$$\begin{aligned} \rho_i &= \sum_{k=0}^{8} \varphi_{ik}\sigma_k, \\ E_j &= \sum_{k=0}^{8} e_{jk}\sigma_k, \end{aligned} \tag{7}$$

for certain *known* real coefficients $\varphi_{ik}$, and for certain *unknown* real coefficients $e_{jk}$. For simplicity, we omit here the explicit value of the coefficients $\varphi_{ik}$; they can be obtained directly from Eq. (6) by using the fact that

$$\varphi_{ik} = \frac{1}{3}\text{Tr}(\rho_i\sigma_k). \tag{8}$$

This means, in particular, that the conditional probabilities $p_{j|i}$ can now be expressed as

$$p_{j|i} = \text{Tr}(E_j\rho_i) = 3\sum_{k=0}^{8} \varphi_{ik} e_{jk}, \tag{9}$$

where we have used Eq. (7) together with the properties of the Gell-Mann operators.

That is, from Eq. (9) we have that the symmetry conditions $p_{0|0} = p_{1|1} = p_{2|2}$ can be rewritten as

$$\begin{aligned} &\sum_{k=0}^{8}(\varphi_{0k}e_{0k} - \varphi_{1k}e_{1k}) \geq 0,\ -\sum_{k=0}^{8}(\varphi_{0k}e_{0k} - \varphi_{1k}e_{1k}) \geq 0, \\ &\sum_{k=0}^{8}(\varphi_{0k}e_{0k} - \varphi_{2k}e_{2k}) \geq 0,\ -\sum_{k=0}^{8}(\varphi_{0k}e_{0k} - \varphi_{2k}e_{2k}) \geq 0. \end{aligned} \tag{10}$$

Similarly, we have that the conditions $p_{3|0} = p_{3|1} =$

$p_{3|2} = q_{\text{inc}}$ have now the form

$$3\sum_{k=0}^{8}\varphi_{0k}e_{3k} - q_{\text{inc}} \geq 0,\ -3\sum_{k=0}^{8}\varphi_{0k}e_{3k} + q_{\text{inc}} \geq 0,$$
$$\sum_{k=0}^{8}(\varphi_{0k}-\varphi_{1k})e_{3k} \geq 0,\ -\sum_{k=0}^{8}(\varphi_{0k}-\varphi_{1k})e_{3k} \geq 0,$$
$$\sum_{k=0}^{8}(\varphi_{0k}-\varphi_{2k})e_{3k} \geq 0,\ -\sum_{k=0}^{8}(\varphi_{0k}-\varphi_{2k})e_{3k} \geq 0, \tag{11}$$

where in the first pair of equations above we impose $p_{3|0} = q_{\text{inc}}$, and in the following two pairs of equations we impose, respectively, $p_{3|1} = p_{3|0}$ and $p_{3|2} = p_{3|0}$.

Also, by using analogous techniques, it is straightforward to rewrite the conditions $p_{1|0} = p_{2|0} = p_{0|1} = p_{2|1} = p_{0|2} = p_{1|2}$ in terms of the real coefficients $\varphi_{ik}$ and $e_{jk}$, which we omit here for simplicity. The constraints $E_j \geq 0$ and $\sum_{j=0}^{3} E_j = \mathbb{1}$ are simply given by,

$$\sum_{k=0}^{8} e_{jk}\sigma_k \geq 0, \tag{12}$$
$$\sum_{k=0}^{8}\sum_{j=0}^{3} e_{jk}\sigma_k - \sigma_0 \geq 0,\ -\sum_{k=0}^{8}\sum_{j=0}^{3} e_{jk}\sigma_k + \sigma_0 \geq 0,$$

since $\sigma_0$ is the identity operator in $\mathcal{H}_3$.

Finally, the objective variable $\mathbf{x}$ (see Eq. (5)) contains the unknown coefficients $e_{jk}$ of the POVM operators $E_j$ for all $j = 0, \ldots, 3$ and $k = 0, \ldots, 8$, *i.e.*, $\mathbf{x} = (e_{00}, \ldots, e_{08}, e_{10}, \ldots, e_{18}, e_{20}, \ldots, e_{28}, e_{30}, \ldots, e_{38})^T$. Similarly, the vector $c^T$ is simply given by $c^T = (-3\varphi_{00}, \ldots, -3\varphi_{08}, 0, \ldots, 0)$ such that $-c^T\mathbf{x} = p_{0|0}$ according to Eq. (9). In doing so, one can express Eq. (4) in the form given by Eq. (5) [20], which can be easily solved numerically [17, 19].

Once we solve Eq. (4) and find the optimal operators $E_j$, the conditional probabilities $p_{j|i}$ can be obtained by simply applying Eq. (9). In particular, we have directly that $q_{\text{s}} = p_{0|0}$. Once $q_{\text{s}}$ is known, we also have from Table I that

$$q_{\text{f}} = \frac{1 - q_{\text{s}} - q_{\text{inc}}}{2}, \tag{13}$$

since $q_{\text{s}} + 2q_{\text{f}} + q_{\text{inc}} = 1$.

## III. GAIN

The gain, which we shall denote by $G$, is defined as the probability that Bob observes a detection click in his data line per signal state sent by Alice. In this context, double clicks (produced by single signals) are counted as single-clicks, as we assume that Bob assigns to them a single bit value which he chooses at random.

The gain can be expressed as $G = N_{\text{clicks}}/N$, where $N_{\text{clicks}}$ refers to the total number of clicks observed by Bob in his data line, and $N$ represents the total number of signal states sent by Alice. In the asymptotic scenario, the quantity $N_{\text{clicks}}$ can be written as $N_{\text{clicks}} = (N/N^{\text{E}})N^{\text{E}}_{\text{clicks}}$, where $N^{\text{E}}$ denotes the average length of the blocks of signals that Eve sends to Bob, and $N^{\text{E}}_{\text{clicks}}$ is the average number of clicks at Bob's data line produced by these blocks of signals. With this notation, we have that the gain can be written as

$$G = \frac{N^{\text{E}}_{\text{clicks}}}{N^{\text{E}}}. \tag{14}$$

Below we calculate the mathematical expressions for the parameters $N^{\text{E}}_{\text{clicks}}$ and $N^{\text{E}}$.

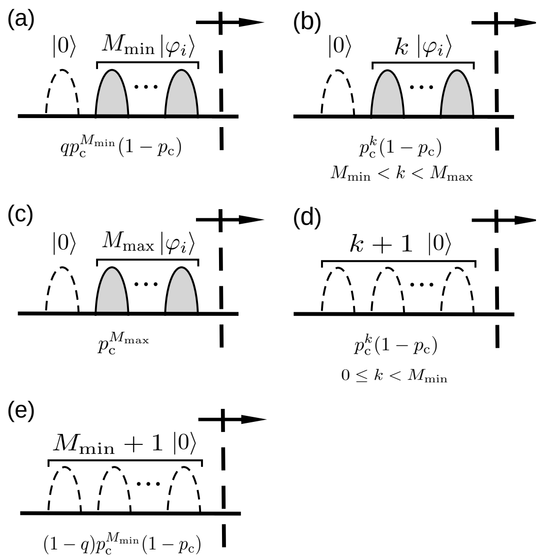


FIG. 2. Blocks of signal states generated by Eve after the first step of her eavesdropping strategy (*i.e.*, before processing the block), together with their *a priori* probabilities. The arrow indicates the transmission direction. For instance, the subfigure (a) indicates that, with probability $qp_{\text{c}}^{M_{\min}}(1-p_{\text{c}})$, Eve generates a block of $M_{\min}+1$ signals, being each of the first $M_{\min}$ signals in a state $|\varphi_i\rangle$ (which, of course, can vary for each signal within the block), while the last one is a vacuum signal $|0\rangle$ (*i.e.*, a vacuum state that lasts two time slots). The signals $|\varphi_i\rangle$ are given by Eq. (1) with $i \in \{0, 1, 2\}$. The other subfigures are interpreted similarly.

### A. Parameter $N^{\text{E}}$

Since we need to determine the average length of the blocks of signals that Eve sends to Bob (independently of how many non-empty pulses they contain), we can consider the blocks of signals generated by Eve after the first step of her eavesdropping strategy (*i.e.*, before she applies the processing), together with their *a priori* probabilities. They are illustrated in Fig. 2.

We remark that, in this context, when we refer to a non-vacuum signal, we shall refer to a signal $|\varphi_i\rangle$, with

$i = 0, \ldots, 2$, given by Eq. (1), even if the signals $|\varphi_i\rangle$ contain vacuum states. In contrast, we shall refer to a vacuum signal as a vacuum state that lasts two time slots, *i.e.*, if we use the notation of Eq. (1), a vacuum signal would be written as $|0\rangle\,|0\rangle$. For simplicity, however, below we will write a vacuum signal as $|0\rangle$ whenever is clear from the context that it refers to a vacuum state that lasts two time slots.

In Fig. 2, the parameter $p_{\rm c}$ denotes the probability that Eve obtains a conclusive result when she measures a signal state sent by Alice. This quantity can be expressed as

$$p_{\rm c} = 1 - \sum_{i=0}^{2} p_{|\varphi_i\rangle} p_{3|i}, \tag{15}$$

where $p_{|\varphi_0\rangle} = p_{|\varphi_1\rangle} = (1-f)/2$ and $p_{|\varphi_2\rangle} = f$, with $f \in (0,1)$, are the probabilities that Alice emits the signal states $|\varphi_i\rangle$, with $i = 0, \ldots, 2$, and the conditional probabilities $p_{3|i}$ have been defined in Section II. From Table I, we have that $p_{3|i} = q_{\rm inc}$ for all $i$, and thus

$$p_{\rm c} = 1 - q_{\rm inc}. \tag{16}$$

This means that the *a priori* probability that Eve prepares a block of $k+1$ signals, being each of the first $k$ signals within the block in a state $|\varphi_i\rangle$ (which, of course, can vary for each signal within the block) and the last signal of the block a vacuum signal (which occupies two time slots), is given by

$$p_{\rm s}(k) = \begin{cases} q p_{\rm c}^{M_{\rm min}}(1-p_{\rm c}) & \text{if } k = M_{\rm min}, \\ p_{\rm c}^{k}(1-p_{\rm c}) & \text{if } M_{\rm min} < k < M_{\rm max}, \\ p_{\rm c}^{M_{\rm max}} & \text{if } k = M_{\rm max}, \\ 0 & \text{otherwise.} \end{cases} \tag{17}$$

Here, the parameter $q$ represents the probability that Eve generates a block of signals like that shown in Fig. 2(a) (instead of that illustrated in Fig. 2(e)) when she obtains $M_{\rm min}$ consecutive conclusive measurement results, followed by one inconclusive result.

Similarly, we have that the probability that Eve generates a block with $k+1$ vacuum signals, is given by

$$p_{\rm v}(k) = \begin{cases} p_{\rm c}^{k}(1-p_{\rm c}) & \text{if } 0 \le k < M_{\rm min}, \\ (1-q) p_{\rm c}^{M_{\rm min}}(1-p_{\rm c}) & \text{if } k = M_{\rm min}, \\ 0 & \text{otherwise.} \end{cases} \tag{18}$$

We find, therefore, that $N^{\rm E}$ can be expressed as

$$N^{\rm E} = \sum_{k=0}^{M_{\rm min}} p_{\rm v}(k)(k+1) + \sum_{k=M_{\rm min}}^{M_{\rm max}} p_{\rm s}(k)(k+1). \tag{19}$$

By substituting Eqs. (17)-(18) into Eq. (19) we finally obtain that $N^{\rm E}$ is given by

$$N^{\rm E} = \frac{1 - p_{\rm c}^{M_{\rm max}+1}}{1 - p_{\rm c}}. \tag{20}$$

### B. Parameter $N^{\rm E}_{\rm clicks}$

Here, we calculate the parameter $N^{\rm E}_{\rm clicks}$. For this, we need to consider only those blocks of signals that Eve sends to Bob containing at least one non-vacuum signal. This is so because we are evaluating the untrusted device scenario, and, thus, as already mentioned in the main text, vacuum signals cannot produce a detection click event at Bob's side.

Consequently, we have that

$$N^{\rm E}_{\rm clicks} = \sum_{k=M_{\rm min}}^{M_{\rm max}} p_{\rm s}(k) p_{\rm click}(k), \tag{21}$$

where the probability $p_{\rm s}(k)$ is given by Eq. (17), and the parameter $p_{\rm click}(k)$ denotes the average number of clicks observed by Bob when Eve sends him a block with $k+1$ signals.

To calculate the probabilities $p_{\rm click}(k)$, we need to take into account the second step of Eve's strategy, *i.e.*, we have to consider the actual blocks of signals that she sends to Bob (after processing) together with their *a priori* probabilities.

Our starting point is a finer-grained characterization of the blocks of signals illustrated in Figs. 2(a)-(b)-(c), *i.e.*, of the blocks that contain at least one non-vacuum signal. Each of these blocks can be of four different types, which we shall denote by "01", "$0 \neq 1$", "$\neq 01$" and "$\neq 0 \neq 1$". They are illustrated in Fig. 3. The blocks of the type "01" are blocks whose first (last non-vacuum) signal is in the state $|\varphi_1\rangle$ ($|\varphi_0\rangle$). The blocks of the type "$0 \neq 1$", on the other hand, are those blocks whose first signal is in a state different from $|\varphi_1\rangle$, while their last non-vacuum signal is in the state $|\varphi_0\rangle$. The other type of blocks are defined analogously.

In doing so, we can express $p_{\rm click}(k)$ as

$$p_{\rm click}(k) = \sum_{\substack{i\in\{0,\neq 0\} \\ j\in\{1,\neq 1\}}} q_{ij}(k) p_{{\rm click}|ij}(k), \tag{22}$$

where $q_{ij}(k)$, with $i \in \{0, \neq 0\}$ and $j \in \{1, \neq 1\}$, denotes the conditional probability that, given a block of the form illustrated in Figs. 2(a)-(b)-(c) of length $k+1$ and containing $k$ non-vacuum signals (obtained by Eve after the first step of her eavesdropping strategy), this block is of the type "$ij$", and $p_{{\rm click}|ij}(k)$ is the average number of clicks observed by Bob when Eve obtains such block (which might still be processed before she sends it to Bob).

To obtain the conditional probabilities $q_{ij}(k)$ with which a given block of length $k+1$ is of the type "$ij$", we need to determine first the conditional probabilities, $p(j|{\rm c})$, with $j = 0, \ldots, 2$, that a given non-vacuum signal within the blocks illustrated in Figs. 2(a)-(b)-(c) is actually in the state $|\varphi_j\rangle$. From Table I, together with the probability that Alice generates the signal $|\varphi_i\rangle$ (which is $(1-f)/2$ if $i = 0, 1$, and $f$ if $i = 2$), we find that $p(j|{\rm c})$

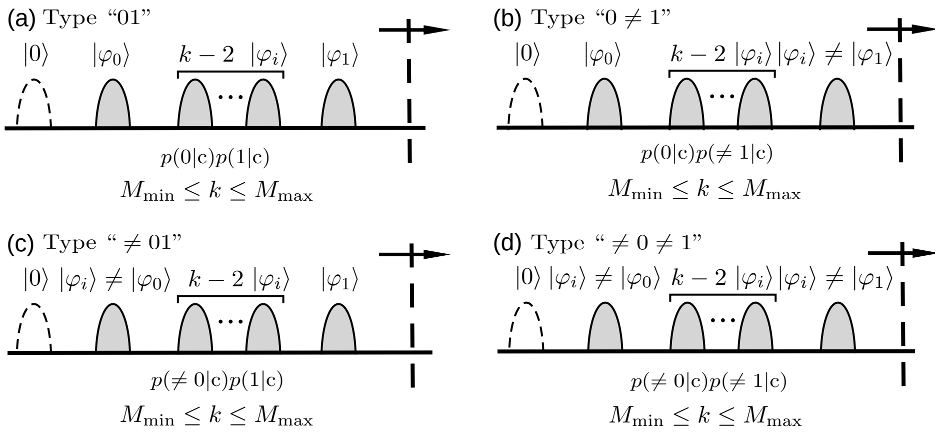


FIG. 3. The four possible types of structures for each of the blocks with $k+1$ signals illustrated in Figs. 2(a)-(b)-(c). We shall denote each of these types by "01", "$0 \neq 1$", "$\neq 01$" and "$\neq 0 \neq 1$". The type "01" refers to those blocks whose first signal is in the state $|\varphi_1\rangle$, while its last non-vacuum signal is in the state $|\varphi_0\rangle$. The description of the other types is analogous. The arrow indicates the transmission direction. Below each type of block we include the conditional probability that Eve generates it, given that she prepares a block of length $k+1$ with $k$ non-vacuum signals.

satisfies

$$\begin{aligned} p(0|\mathrm{c}) &= \frac{1}{2p_{\mathrm{c}}}\left[(1-f)q_{\mathrm{s}} + (1+f)q_{\mathrm{f}}\right], \\ p(1|\mathrm{c}) &= p(0|\mathrm{c}), \\ p(2|\mathrm{c}) &= \frac{1}{p_{\mathrm{c}}}\left[f q_{\mathrm{s}} + (1-f)\, q_{\mathrm{f}}\right]. \end{aligned} \tag{23}$$

Obviously, these probabilities fulfill $\sum_{j=0}^{2} p(j|\mathrm{c}) = 1$.

Similarly, we denote the conditional probability that a given non-vacuum signal within the blocks illustrated in Figs. 2(a)-(b)-(c) is not prepared in the state $|\varphi_j\rangle$ by $p(\neq j|\mathrm{c})$. These probabilities satisfy

$$p(\neq j|\mathrm{c}) = \sum_{\substack{j'=0 \\ j'\neq j}}^{2} p(j'|\mathrm{c}), \tag{24}$$

with $j = 0, \ldots, 2$, and $p(j'|\mathrm{c})$ given by Eq. (23). This means that

$$\begin{aligned} p(\neq 0|\mathrm{c}) &= \frac{1}{2p_{\mathrm{c}}}\left[(1+f)q_{\mathrm{s}} + (3-f)q_{\mathrm{f}}\right], \\ p(\neq 1|\mathrm{c}) &= p(\neq 0|\mathrm{c}), \\ p(\neq 2|\mathrm{c}) &= \frac{1}{p_{\mathrm{c}}}\left[(1-f)q_{\mathrm{s}} + (1+f)q_{\mathrm{f}}\right]. \end{aligned} \tag{25}$$

Obviously, these probabilities satisfy $p(\neq j|\mathrm{c})+p(j|\mathrm{c}) = 1$ for all $j = 0, \ldots, 2$.

We have, therefore, that the conditional probabilities $q_{ij}(k)$ can be written as

$$q_{ij}(k) = p(i|\mathrm{c})p(j|\mathrm{c}), \tag{26}$$

where $p(0|\mathrm{c})$ and $p(1|\mathrm{c})$ are given by Eq. (23), and $p(\neq 0|\mathrm{c})$ and $p(\neq 1|\mathrm{c})$ are given by Eq. (25). We note that these probabilities do not depend on the parameter $k$ for the cases that we are interested.

In the next section, we calculate $p_{\mathrm{click}|ij}(k)$ for $M_{\min} \leq k \leq M_{\max}$.

### 1. *Probability* $p_{\mathrm{click}|ij}(k)$

Let us denote by $\Gamma_{\mathrm{click}}(i, j, L)$ the average number of clicks observed by Bob in his data line when Eve sends him a block of signals of the type "$ij$" containing $L+2$ non-vacuum signals (after the processing of the block). This quantity is provided in Section III B 3 and we will use it in our calculations below.

To obtain $p_{\mathrm{click}|ij}(k)$, we start with the case $k = M_{\min}$, and, moreover, we will suppose for the moment that the block is of the type "01". In this scenario, we have that Eve always sends such block to Bob. This means, in particular, that

$$p_{\mathrm{click}|01}(M_{\min}) = \Gamma_{\mathrm{click}}(0, 1, M_{\min}-2), \tag{27}$$

since the block that Eve sends to Bob in this case contains $M_{\min}$ non-vacuum signals.

On the other hand, if the block is not of the type "01", then Eve sends the block to Bob with probability $1-q_{\mathrm{p}}$, while with probability $q_{\mathrm{p}}$ she tries to process it. In this latter case, when $k = M_{\min}$ this means that she sends him a block with $M_{\min}+1$ vacuum signals, which cannot produce a click at Bob's side. We have, therefore, that

$$p_{\mathrm{click}|ij}(M_{\min}) = (1-q_{\mathrm{p}})\Gamma_{\mathrm{click}}(i, j, M_{\min}-2), \tag{28}$$

with $ij \in \Delta$, where the set $\Delta$ is given by

$$\Delta = \{\text{“}0 \neq 1\text{''}, \text{“} \neq 01\text{''}, \text{“} \neq 0 \neq 1\text{''}\}. \tag{29}$$

Let us now consider $p_{\mathrm{click}|ij}(k)$ with $M_{\min} < k \leq M_{\max}$. Again, if the block is of the type "01", this block is directly sent to Bob. This means that

$$p_{\mathrm{click}|01}(k) = \Gamma_{\mathrm{click}}(0, 1, k-2). \tag{30}$$

On the other hand, if the block is not of the type "01" then Eve sends it to Bob with probability $1-q_{\mathrm{p}}$, and she

tries to process it with probability $q_{\rm p}$. The goal of the processing is to generate a new block of signals with the same length as the original one but which now begins (after, possibly, some vacuum signals) with a signal in the state $|\varphi_1\rangle$ and ends up with a signal prepared in the state $|\varphi_0\rangle$ (followed, possibly, by some vacuum signals). This means that

$$p_{{\rm click}|ij}(k)=(1-q_{\rm p})\Gamma_{\rm click}(i,j,k-2)+q_{\rm p}r^{\rm p}_{{\rm click}|ij}(k), \quad (31)$$

with $ij\in\Delta$, and where $r^{\rm p}_{{\rm click}|ij}(k)$ denotes the average number of clicks observed by Bob in his data line when Eve sends him a processed block of signals of length $k+1$ which originally was of the type "$ij$".

To finish this part, next we calculate $r^{\rm p}_{{\rm click}|ij}(k)$ with $ij\in\Delta$. We start with blocks of the type "$0\neq 1$". In this case, Eve's processing consists of checking whether or not the non-vacuum signals are prepared in the state $|\varphi_1\rangle$. For this, she starts from the first signal of the block (towards its last signal) and replaces all the non-vacuum signals which are not prepared in the state $|\varphi_1\rangle$ with vacuum signals (each of them occupying two time slots) until she finds a signal prepared in the state $|\varphi_1\rangle$, where she stops. Afterwards, in a second step, she checks whether or not the number of remaining non-vacuum signals within the block is still greater or equal than $M_{\rm min}$. If it is, she sends the resulting block to Bob. Otherwise, she sends Bob a block with $k+1$ vacuum signals. This case is illustrated in Fig. 4(a). It is easy to show that in this scenario we have that

$$r^{\rm p}_{{\rm click}|0\neq 1}(k)=p(1|{\rm c})\sum_{l=0}^{k-M_{\rm min}-1}p(\neq 1|{\rm c})^l \times\Gamma_{\rm click}(0,1,k-3-l). \quad (32)$$

The quantity $r^{\rm p}_{{\rm click}|\neq 01}(k)$ can be obtained following the same procedure. All the different cases are illustrated in Fig. 4(b). To be precise, we find that

$$r^{\rm p}_{{\rm click}|\neq 01}(k)=p(0|{\rm c})\sum_{l=0}^{k-M_{\rm min}-1}p(\neq 0|{\rm c})^l \times\Gamma_{\rm click}(0,1,k-3-l). \quad (33)$$

Finally, the calculation of $r^{\rm p}_{{\rm click}|\neq 0\neq 1}(k)$ is analogous, but a bit more tedious. We can decompose it into two steps. First, Eve replaces the first and last non-vacuum signals within the block (which are different from $|\varphi_1\rangle$ and $|\varphi_0\rangle$, respectively) with vacuum signals. Afterwards, she checks the remaining non-vacuum signals of the block, starting from say the last non-vacuum signal (towards its first non-vacuum signal), and she replaces all the non-vacuum signals with vacuum signals until she finds a signal prepared in the state $|\varphi_0\rangle$ where she stops. Then, in a second step, she checks the non-vacuum signals starting from the first non-vacuum signal of the block (towards its last non-vacuum signal), and she replaces all the non-vacuum signals with vacuum signals until she finds a signal equal to $|\varphi_1\rangle$ where she stops. To conclude, she checks if the number of remaining non-vacuum signals within the block is greater or equal than $M_{\rm min}$. If it is, she sends the resulting block to Bob. Otherwise, she sends Bob a block with $k+1$ vacuum signals.

After completing the first step, we have that with probability $p(0|{\rm c})p(\neq 0|{\rm c})^l$, with $l=0,\ldots,k-M_{\rm min}-2$, Eve generates a block of signals which contains (starting from the signal located at the first position of the block) a vacuum signal, followed by $k-l-3$ signals $|\varphi_i\rangle$, followed by the signal $|\varphi_0\rangle$, followed by at least two vacuum signals. This is illustrated in Fig. 4(c), where we illustrate the different possibilities depending on the value of $l$. Next, for each value of $l$, in the second step, we have that with probability $p(1|{\rm c})p(\neq 1|{\rm c})^{l'}$, with $l'=0,\ldots,k-l-M_{\rm min}-2$, Eve finally generates a block of signals which contains (starting again from the signal located at the first position of the block) $l'+1$ vacuum signals, followed by the signal $|\varphi_1\rangle$, followed by $k-l-l'-4$ signals $|\varphi_i\rangle$, followed by the signal $|\varphi_0\rangle$, followed by $l+2$ vacuum signals. This is illustrated in Fig. 4(d), where we show the different possibilities depending on the value of $l'$ given that $l$ is fixed to say $l=0$.

In short, we find that $r^{\rm p}_{{\rm click}|\neq 0\neq 1}(k)$ can be expressed as

$$r^{\rm p}_{{\rm click}|\neq 0\neq 1}(k)=p(0|{\rm c})p(1|{\rm c})\sum_{l=0}^{k-M_{\rm min}-2}\sum_{l'=0}^{k-l-M_{\rm min}-2} \times p(\neq 0|{\rm c})^l p(\neq 1|{\rm c})^{l'} \times\Gamma_{\rm click}(0,1,k-l-l'-4). \quad (34)$$

### 2. *Probability* $p_{\rm click}(k)$

By using Eqs. (22)-(26)-(27)-(28), we find that

$$p_{\rm click}(M_{\rm min})=p(0|{\rm c})p(1|{\rm c})\Gamma_{\rm click}(0,1,M_{\rm min}-2) + (1-q_{\rm p})\sum_{ij\in\Delta}p(i|{\rm c})p(j|{\rm c}) \times\Gamma_{\rm click}(i,j,M_{\rm min}-2). \quad (35)$$

On the other hand, by combining Eqs. (22)-(26)-(30)-(31)-(32)-(33)-(34), we obtain

$$p_{\rm click}(k)=p(0|{\rm c})p(1|{\rm c})\Gamma_{\rm click}(0,1,k-2)+\sum_{ij\in\Delta}p(i|{\rm c})p(j|{\rm c})\Big\{(1-q_{\rm p})\Gamma_{\rm click}(i,j,k-2)+q_{\rm p}r^{\rm p}_{{\rm click}|ij}(k)\Big\}, \quad (36)$$

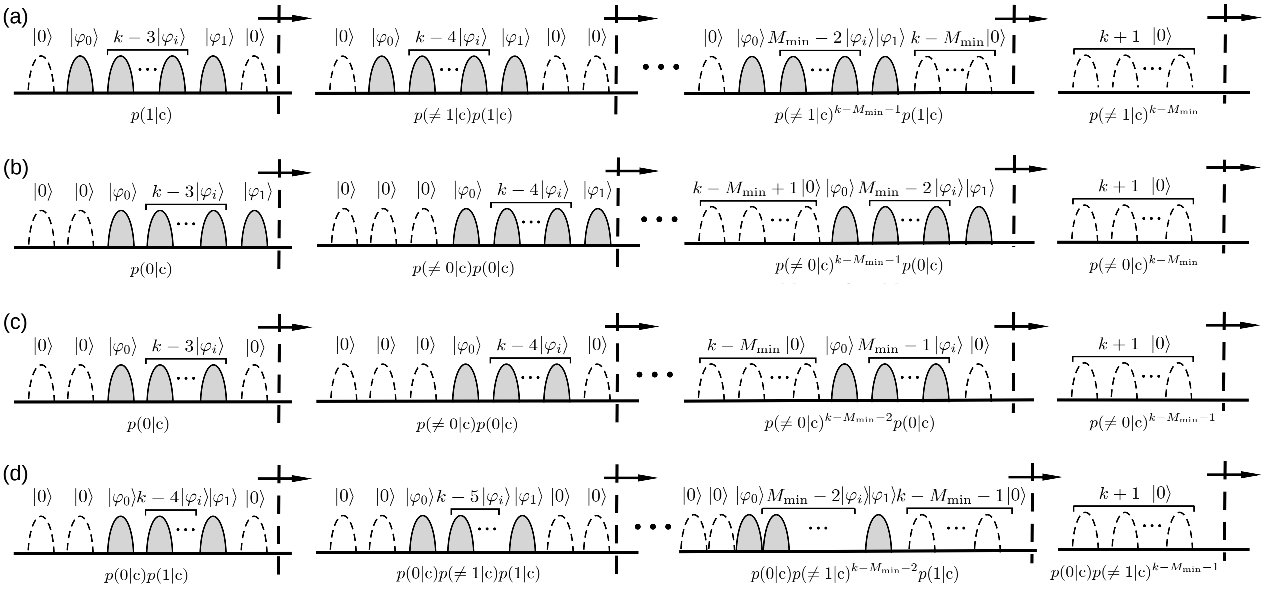

FIG. 4. Structure of the blocks of signal states generated by Eve after processing, together with their conditional probabilities given that in the first step of her eavesdropping strategy Eve obtains a block of length $k+1$ (with $k$ non-vacuum signals) of a certain type from the set $\Delta$ given by Eq. (29). The arrow indicates the transmission direction, being the first signal of the block that which is sent to Bob first. (a) This corresponds to a block of signals of the type "$0 \neq 1$" and, starting from the first signal of the block, Eve replaces all non-vacuum signals with vacuum signals until she finds a signal equal to $|\varphi_1\rangle$ where she stops. If the number of remaining non-vacuum signals within the block is greater or equal than $M_{\rm min}$, then she sends the block to Bob. Otherwise, she sends Bob a block with $k+1$ vacuum signals (which is illustrated in the last subfigure of figure (a)). (b) This corresponds to a block of signals of the type "$\neq 01$" and, starting from the last non-vacuum signal of the block, Eve replaces all non-vacuum signals with vacuum signals until she finds a signal in the state $|\varphi_0\rangle$ where she stops. If the number of remaining non-vacuum signals within the block is greater or equal than $M_{\rm min}$, then she sends the block to Bob. Otherwise, she sends Bob a block with $k+1$ vacuum signals (which is illustrated in the last subfigure of figure (b)). (c) This corresponds to a block of signals of the type "$\neq 0 \neq 1$". In a first step, Eve replaces the first and last non-vacuum signals within the block (which are different from $|\varphi_1\rangle$ and $|\varphi_0\rangle$, respectively) with vacuum signals. Afterwards, she checks the remaining non-vacuum signals starting from the last non-vacuum signal of the block, and she replaces all the non-vacuum signals with vacuum signals until she finds a signal in the state $|\varphi_0\rangle$ where she stops. If the number of remaining non-vacuum signals within the resulting block is smaller than $M_{\rm min}$, then she sends Bob a block with $k+1$ vacuum signals (which is illustrated in the last subfigure of figure (c)). In a second step (which is shown in figure (d) for the case where Eve finds the signal $|\varphi_0\rangle$ in the third last signal of the block), Eve checks the remaining non-vacuum signals starting from the first non-vacuum signal of the block, and she replaces all the non-vacuum signals with vacuum signals until she finds a signal in the state $|\varphi_1\rangle$ where she stops. If the number of non-vacuum signals within the resulting block is greater or equal than $M_{\rm min}$, she sends the resulting block to Bob. Otherwise, she sends Bob a block with $k+1$ vacuum signals (which is illustrated in the last subfigure of figure (d)).

with the set $\Delta$ given by Eq. (29), and where $r^{\rm p}_{{\rm click}|ij}(k)$, with $ij \in \Delta$, is given by Eqs. (32)-(33)-(34), respectively.

Finally, by using Eqs. (17)-(21)-(35)-(36) we obtain the value of $N^{\rm E}_{\rm clicks}$, which can be combined with Eqs. (14)-(20) to find the gain $G$.

### 3. *Average number of clicks* $\Gamma_{\rm click}(i,j,L)$

Here we calculate the average number of clicks, $\Gamma_{\rm click}(i,j,L)$, observed by Bob in his data line when Eve sends him a block of signals of the type "$ij$", with $i \in \{0, \neq 0\}$ and $j \in \{1, \neq 1\}$, containing $L+2$ non-vacuum signals (after processing the block). These blocks of signals are illustrated in Fig. 5. As already mentioned, double clicks (produced by a signal $|\varphi_i\rangle$) are counted as single-clicks, as Bob assigns to them a bit value which he chooses at random.

In the case of a block of signals like that shown in Fig. 5(a) of length $k+1$, *i.e.*, a block whose first (last) non-vacuum signal is $|\varphi_1\rangle$ ($|\varphi_0\rangle$), we have that the average number of clicks observed by Bob is given by

$$\Gamma_{\rm click}(0,1,L) = 2p_{{\rm click}|0}p_{{\rm click}|1} + p_{{\rm click}|0}(1-p_{{\rm click}|1}) + (1-p_{{\rm click}|0})p_{{\rm click}|1} + \sum_{i=1}^{L} i \binom{L}{i} \gamma_{\rm click}^{i}(1-\gamma_{\rm click})^{L-i}, \quad (37)$$

with $L = k - l - l' - 1$. In Eq. (37), $p_{{\rm click}|0}$ ($p_{{\rm click}|1}$) is the conditional probability that Bob observes a detection

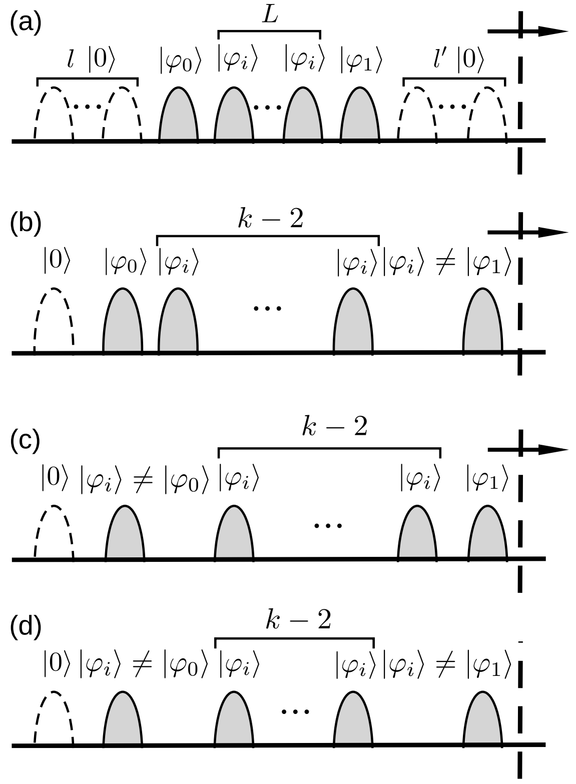


FIG. 5. Generic structure of the blocks of signals of length $k+1$ that Eve sends to Bob after processing the block. (a) The first (last) non-vacuum signal of the block is $|\varphi_1\rangle$ ($|\varphi_0\rangle$). These blocks originate from blocks of the type "01" or from blocks of a type $ij \in \Delta$ which are successfully processed by Eve (*i,e.*, she is able to generate a block whose first and last signals are, respectively, $|\varphi_1\rangle$ and $|\varphi_0\rangle$, and the total number of non-vacuum signals is greater or equal than $M_{\rm min}$). They satisfy $L = k - l - l' - 1$, with $l \geq 1$ and $l' \geq 0$; (b) The first (last) non-vacuum signal of the block is different from $|\varphi_1\rangle$ (equal to $|\varphi_0\rangle$). These blocks correspond to blocks of the type "$0 \neq 1$" which are not processed by Eve; (c) The first (last) non-vacuum signal of the block is $|\varphi_1\rangle$ (different from $|\varphi_0\rangle$). These blocks correspond to blocks of the type "$\neq 01$" which are not processed by Eve; (d) The first (last) non-vacuum signal of the block is not equal to $|\varphi_1\rangle$ ($|\varphi_0\rangle$). These blocks correspond to blocks of the type "$\neq 0 \neq 1$" which are not processed by Eve.

click in his data line given that Eve sends him the signal $|\varphi_0\rangle$ ($|\varphi_1\rangle$), and $\gamma_{\rm click}$ is the probability that each of the $L$ non-vacuum signals (located between the pulses $|\varphi_1\rangle$ and $|\varphi_0\rangle$ in Fig. 5(a)) produces a click at Bob's data line. That is, the first three terms in Eq. (37) represent the average number of clicks observed by Bob due to the two signals $|\varphi_1\rangle$ and $|\varphi_0\rangle$, while the last term represents the average number of clicks observed by Bob due to the $L$ non-vacuum signals located between the two previous pulses.

The conditional probabilities $p_{{\rm click}|j}$, with $j = 0, \ldots, 2$, have the form

$$p_{{\rm click}|0} = p_{{\rm click}|1} = 1 - e^{-t_{\rm B}|\beta|^2},$$
$$p_{{\rm click}|2} = 1 - e^{-2t_{\rm B}|\beta|^2}, \quad (38)$$

where $t_{\rm B}$ is the transmittance of Bob's beamsplitter, and $|\beta|^2$, as already mentioned, is the intensity of the coherent states that Eve sends to Bob.

On the other hand, the quantity $\gamma_{\rm click}$ can be written as

$$\gamma_{\rm click} = \sum_{i=0}^{2} p(i|{\rm c}) p_{{\rm click}|i} = \frac{1}{p_{\rm c}} \left\{ [(1-f)q_{\rm s} + (1+f)q_{\rm f}] \left(1 - e^{-t_{\rm B}|\beta|^2}\right) + [f q_{\rm s} + (1-f)\, q_{\rm f}] \left(1 - e^{-2t_{\rm B}|\beta|^2}\right) \right\}, \quad (39)$$

where we have used Eqs. (23) and (38).

The calculation of the average number of clicks observed by Bob when he receives the blocks of signals illustrated in Figs. 5(b)-(c)-(d) is analogous. To be precise, we have that

$$\Gamma_{\rm click}(i,j,L) = 2 p_{{\rm click}|i} p_{{\rm click}|j} + p_{{\rm click}|i}(1 - p_{{\rm click}|j}) + (1 - p_{{\rm click}|i}) p_{{\rm click}|j} + \sum_{m=1}^{L} m \binom{L}{m} \gamma_{\rm click}^m (1 - \gamma_{\rm click})^{L-m}, \quad (40)$$

with $L = k - 2$, and $ij \in \Delta$ given by Eq. (29).

The conditional probabilities $p_{\text{click}|\neq 0}$ ($p_{\text{click}|\neq 1}$), that Bob observes a detection click in his data line given that Eve sends him a non-vacuum signal different from $|\varphi_0\rangle$ ($|\varphi_1\rangle$), which are required to evaluate Eq. (40), are given by

$$\begin{aligned} p_{\text{click}|\neq 0} &= \frac{1}{p(1|\text{c}) + p(2|\text{c})} \sum_{i=1}^{2} p(i|\text{c}) p_{\text{click}|\text{i}}, \\ p_{\text{click}|\neq 1} &= p_{\text{click}|\neq 0}, \end{aligned} \tag{41}$$

with the probabilities $p(i|\text{c})$ given by Eq. (23). The fact that $p_{\text{click}|\neq 1} = p_{\text{click}|\neq 0}$ is because $p(0|\text{c}) = p(1|\text{c})$.

## IV. QBER

In this Section, we calculate the QBER in Bob's data line. A principal difference between this case and that considered in Section III (besides the obvious fact that both Sections calculate different quantities), is that here we are only interested in those instances where Alice sends Bob a signal state $|\varphi_0\rangle$ or $|\varphi_1\rangle$. This is so because the decoy signals $|\varphi_2\rangle$ are not included in the definition of the QBER.

To be precise, the QBER, which we shall denote by $Q$, is defined as

$$Q = \frac{M_{\text{errors}}}{M_{\text{clicks}}}, \tag{42}$$

where $M_{\text{errors}}$ refers to the average total number of errors obtained by Bob when Alice sends him the signal states $\{|\varphi_0\rangle, |\varphi_1\rangle\}$, and $M_{\text{clicks}}$ (in contrast to the quantity $N_{\text{clicks}}$ introduced in Section III) represents the average total number of clicks at Bob's side when Alice sends him these signal states.

The parameter $M_{\text{clicks}}$ can be written as

$$\frac{M_{\text{clicks}}}{N} = \sum_{i=0}^{1} p_{|\varphi_i\rangle} \sum_{j=0}^{2} p_{j|i} p_{\text{block}|\varphi_j\rangle|j} p_{\text{click}|j}, \tag{43}$$

where $p_{|\varphi_i\rangle}$ is again the probability that Alice emits the signal state $|\varphi_i\rangle$, $p_{j|i}$ is the conditional probability that the output result of Eve's measurement is the state $|\varphi_j\rangle$ given that the input state is $|\varphi_i\rangle$ (this quantity is given by Eq. (3) and Table I), the parameter $p_{\text{block}|\varphi_j\rangle|j}$ is the probability that the signal $|\varphi_j\rangle$ is actually sent to Bob in a block of signals (*i.e.*, it is not replaced by Eve with a vacuum signal), $p_{\text{click}|j}$ is the conditional probability that Bob observes a click given that he receives the signal $|\varphi_j\rangle$ (this quantity is given by Eq. (38)), and $N$ represents the total number of signals sent by Alice.

By substituting the expressions for the different parameters in Eq. (43), and by taking into account that $p_{\text{click}|1} = p_{\text{click}|0}$, $p_{0|0} = p_{1|1} = q_{\text{s}}$, and $p_{0|1} = p_{1|0} = p_{2|0} = p_{2|1} = q_{\text{f}}$, we find that

$$\begin{aligned} \frac{M_{\text{clicks}}}{N} &= \frac{1-f}{2} \bigg[ (q_{\text{s}} + q_{\text{f}}) \left(1 - e^{-t_{\text{B}}|\beta|^2}\right) \sum_{i=0}^{1} p_{\text{block}|\varphi_i\rangle|i} \\ &\quad + 2q_{\text{f}} \left(1 - e^{-2t_{\text{B}}|\beta|^2}\right) p_{\text{block}|\varphi_2\rangle|2} \bigg]. \end{aligned} \tag{44}$$

Similarly, we have that the parameter $M_{\text{errors}}$ can be written as

$$\frac{M_{\text{errors}}}{N} = \sum_{i=0}^{1} p_{|\varphi_i\rangle} \sum_{j=0}^{2} p_{j|i} p_{\text{block}|\varphi_j\rangle|j} p_{\text{error}|ji}, \tag{45}$$

where $p_{\text{error}|ji}$ is the conditional probability that Bob observes a click associated to an error given that he receives the signal $|\varphi_j\rangle$ and the original signal emitted by Alice is $|\varphi_i\rangle$. This latter probability satisfies

$$\begin{aligned} p_{\text{error}|00} &= p_{\text{error}|11} = 0, & p_{\text{error}|10} &= p_{\text{click}|1}, \\ p_{\text{error}|01} &= p_{\text{click}|0}, & p_{\text{error}|20} &= p_{\text{error}|21}, \end{aligned} \tag{46}$$

with

$$\begin{aligned} p_{\text{error}|20} &= e^{-t_{\text{B}}|\beta|^2} \left(1 - e^{-t_{\text{B}}|\beta|^2}\right) + \frac{1}{2} \left(1 - e^{-t_{\text{B}}|\beta|^2}\right)^2 \\ &= \frac{1}{2} \left(1 - e^{-2t_{\text{B}}|\beta|^2}\right). \end{aligned} \tag{47}$$

Note that in Eq. (47) we have taken into account that Bob assigns at random double clicks to single clicks, and thus the error probability associated to these instances is 1/2. By inserting the values of the different parameters in Eq. (45), we obtain

$$\begin{aligned} \frac{M_{\text{errors}}}{N} &= \frac{1-f}{2} \bigg[ q_{\text{f}} \left(1 - e^{-t_{\text{B}}|\beta|^2}\right) \sum_{i=0}^{1} p_{\text{block}|\varphi_i\rangle|i} \\ &\quad + q_{\text{f}} \left(1 - e^{-2t_{\text{B}}|\beta|^2}\right) p_{\text{block}|\varphi_2\rangle|2} \bigg]. \end{aligned} \tag{48}$$

If we now use Eqs. (44)-(48) in Eq. (42), we find that the QBER can be written as

$$Q = \frac{\sum_{i=0}^{1} p_{\text{block}|\varphi_i\rangle|i} + \xi p_{\text{block}|\varphi_2\rangle|2}}{\left(1 + \frac{q_{\text{s}}}{q_{\text{f}}}\right) \sum_{i=0}^{1} p_{\text{block}|\varphi_i\rangle|i} + 2\xi p_{\text{block}|\varphi_2\rangle|2}}, \tag{49}$$

with $\xi = 1 + e^{-t_{\text{B}}|\beta|^2}$.

The probabilities $p_{\text{block}|\varphi_i\rangle|i}$, with $i = 0, \ldots, 2$, are calculated in Section IV A.

### A. Probabilities $p_{\text{block}|\varphi_i\rangle|i}$

These probabilities can be written as

$$p_{\text{block}|\varphi_i\rangle|i} = \sum_{l=M_{\min}+1}^{M_{\max}+1} p_{(l|i)} p_{\text{block}|\varphi_i\rangle|il}, \tag{50}$$

where $p_{(l|i)}$ is the conditional probability that Eve's result is included within a block of length $l$ given that she obtains the outcome $|\varphi_i\rangle$, and $p_{\text{block}|\varphi_i\rangle|il}$ is the conditional probability that Eve sends Bob the signal $|\varphi_i\rangle$ given that her measurement result is $|\varphi_i\rangle$ and this signal is included in a block of length $l$. In Eq. (50), the sum goes from $l = M_{\min}+1,\ldots,M_{\max}+1$ because $p_{\text{block}|\varphi_i\rangle|il} = 0$ whenever $l < M_{\min}+1$ as in that case Eve always sends vacuum signals to Bob.

By taking into account that whenever Eve's measurement result is $|\varphi_i\rangle$, with $i = 0,1,2$, and this signal is included in a block of length $l$, with $M_{\min}+1 \leq l \leq M_{\max}+1$, then Eve always sends Bob either $|\varphi_i\rangle$ or a vacuum signal, we can rewrite $p_{\text{block}|\varphi_i\rangle|il}$ as

$$p_{\text{block}|\varphi_i\rangle|il} = 1 - p_{\text{block}|0\rangle|il}. \tag{51}$$

Here, $p_{\text{block}|0\rangle|il}$ is the conditional probability that Eve sends Bob a vacuum signal given that her measurement result is $|\varphi_i\rangle$ and this instance is included in a block of length $l$.

By combining Eqs. (50)-(51) we have that

$$p_{\text{block}|\varphi_i\rangle|i} = \sum_{l=M_{\min}+1}^{M_{\max}+1} p_{(l|i)} \left[1 - p_{\text{block}|0\rangle|il}\right]. \tag{52}$$

On the other hand, the probabilities $p_{\text{block}|0\rangle|il}$, with $M_{\min}+1 \leq l \leq M_{\max}+1$, can be written as

$$p_{\text{block}|0\rangle|il} = \sum_{j=1}^{l} p_{j|il} p_{\text{block}|0\rangle|ilj}, \tag{53}$$

where $p_{j|il}$ is the conditional probability that the signal prepared by Eve occupies the $j$th position of the block given that Eve's measurement result is $|\varphi_i\rangle$ and the block has length $l$, and $p_{\text{block}|0\rangle|ilj}$ denotes the conditional probability that Eve sends Bob a vacuum signal given that her measurement result is $|\varphi_i\rangle$, and the position of this signal within the block of length $l$ is the $j$th position.

Given that Eve obtains a result $|\varphi_i\rangle$, we have that it is equally likely that this instance corresponds to any position in the block (except for the last position, where Eve's measurement result is always a vacuum signal in the case of $l = M_{\min}+1,\ldots,M_{\max}$ and Eve does not even measure it if $l = M_{\max}+1$). This means that

$$p_{j|il} = \begin{cases} \frac{1}{l-1} & \text{for } j = 1,\ldots,l-1, \\ 0 & \text{for } j = l, \end{cases} \tag{54}$$

for all $l = M_{\min}+1,\ldots,M_{\max}+1$.

### 1. $p_{\text{block}|\varphi_0\rangle|0}$

According to Eq. (52), to obtain $p_{\text{block}|\varphi_0\rangle|0}$ we need to calculate $p_{(l|0)}$ and $p_{\text{block}|0\rangle|0l}$. This is what we do next.

*a. Probability $p_{\text{block}|0\rangle|0M_{\min}+1}$* When the length of the block is $M_{\min}+1$, we have that Eve sends Bob a block of $M_{\min}+1$ vacuum signals with probability $1-q$, while with probability $q$ she tries to process the block further. This means that

$$p_{\text{block}|0\rangle|0M_{\min}+1} = (1-q) + q \sum_{j=1}^{M_{\min}+1} p_{j|0M_{\min}+1} \times p_{\text{block}|0\rangle|0M_{\min}+1j}, \tag{55}$$

where the probabilities $p_{j|0M_{\min}+1}$ (which are given by Eq. (54)) and $p_{\text{block}|0\rangle|0M_{\min}+1j}$ refer to the scenario where Eve decides to process the block further. In this latter case, the only possibility for a signal $|\varphi_0\rangle$ to be replaced by a vacuum signal is that the original block is not of the type "01" (see Section III) and, moreover, Eve decides to change all the non-vacuum signals with vacuum signals, which happens with probability $q_{\text{p}}$.

To be precise, in the case of $j=1$, *i.e.*, if Eve's result corresponds to the first position of the block, we have directly that the resulting block is not of the type "01", and thus

$$p_{\text{block}|0\rangle|0M_{\min}+11} = q_{\text{p}}. \tag{56}$$

Similarly, if Eve's result corresponds to a position in the middle of the block, *i.e.*, $1 < j < M_{\min}$, then the block is not of the type "01" with probability $1 - q_{01}$, where $q_{01}$ is given by Eq. (26). Therefore, we find that

$$p_{\text{block}|0\rangle|0M_{\min}+1j} = (1-q_{01})q_{\text{p}}, \tag{57}$$

when $1 < j < M_{\min}$.

If we now consider the case where Eve's result corresponds to the position $M_{\min}$ of the block, *i.e.*, $j = M_{\min}$, then the only option for the block not being of the type "01" is that its first signal is not equal to $|\varphi_1\rangle$. This happens with probability $p(\neq 1|\text{c})$ given by Eq. (24). This means that,

$$p_{\text{block}|0\rangle|0M_{\min}+1M_{\min}} = p(\neq 1|\text{c})q_{\text{p}}. \tag{58}$$

Finally, we have that Eve cannot obtain the result $|\varphi_0\rangle$ in the position $j = M_{\min}+1$ (*i.e.*, $p_{M_{\min}+1|0M_{\min}+1} = 0$). This is so because if the block is of length $M_{\min}+1$ then in the last signal of the block she obtained an inconclusive result. By substituting Eqs. (54)-(60)-(57)-(58) into Eq. (55), we obtain

$$p_{\text{block}|0\rangle|0M_{\min}+1} = (1-q) + \frac{qq_{\text{p}}}{M_{\min}}\big[1 + (M_{\min}-2) \times (1-q_{01}) + p(\neq 1|\text{c})\big]. \tag{59}$$

*b. Probabilities $p_{\text{block}|0\rangle|0l}$ with $M_{\min}+1 < l \leq M_{\max}+1$* In this scenario, Eve replaces the signal $|\varphi_0\rangle$ with a vacuum signal only if the block is not of the type "01", and, moreover, Eve decides to process it (which happens with probability $q_{\text{p}}$) but she is not able to generate a sub-block of the type "01" of length at least $M_{\min}$ non-vacuum signals which includes the signal $|\varphi_0\rangle$.

In particular, if Eve obtains the measurement result $|\varphi_0\rangle$ in the first position of the block, *i.e.*, when $j=1$, then the block is obviously not of the type "01". This means that if Eve tries to process it, she will always send (even if she is successful with her processing) a vacuum signal in the first position of the block. Therefore, we have that

$$p_{\text{block}|0\rangle|0l1} = q_{\text{p}}. \tag{60}$$

On the other hand, if Eve obtains the measurement result $|\varphi_0\rangle$ in the middle of the block, *i.e.*, $1<j<l-1$, her strategy depends on the type of block $i'j' \in \Delta$ considered (see Section III). There are three different types of block that have to be evaluated: "$0 \neq 1$", "$\neq 01$" and "$\neq 0 \neq 1$", and we can write

$$p_{\text{block}|0\rangle|0lj} = \sum_{i'j' \in \Delta} q_{i'j'} p_{\text{block}|0\rangle|0lji'j'}, \tag{61}$$

where the probabilities $q_{i'j'}$ are given by Eq. (26), and $p_{\text{block}|0\rangle|0lji'j'}$ includes the condition that the block is of the type $i'j'$.

Let us consider first blocks of the type "$0 \neq 1$". If Eve's result corresponds to the second position of the block (*i.e.*, if $j=2$) then she always sends Bob a vacuum signal. This is so because if Eve decides to process the block, then (starting from the first position of the block) she replaces all signals with vacuum signals until she finds a signal in the state $|\varphi_1\rangle$. And, in the scenario considered, the first two signals are different from $|\varphi_1\rangle$. Therefore, we have that $p_{\text{block}|0\rangle|0l20\neq1} = q_{\text{p}}$. Similarly, if $j=3,\ldots,l-2$, we have that Eve sends Bob a vacuum signal (instead of the signal $|\varphi_0\rangle$) if in the previous $j-2$ positions there is no signal $|\varphi_1\rangle$, or if the number of non-vacuum signals within the resulting modified block is strictly less than $M_{\min}$ (*i.e.*, if none of the first $l-M_{\min}$ signals is in the state $|\varphi_1\rangle$, as the last signal of the block is already a vacuum signal).

This is illustrated in Fig. 6. We find, therefore, that

$$p_{\text{block}|0\rangle|0lj0\neq1} = \begin{cases} q_{\text{p}} p(\neq 1|\text{c})^{j-2} & \text{for } j=2,\ldots,l-M_{\min}, \\ q_{\text{p}} p(\neq 1|\text{c})^{l-M_{\min}-1} & \text{for } j=l-M_{\min}+1,\ldots,l-2. \end{cases} \tag{62}$$

Let us now consider the blocks of the type "$\neq 01$". In this scenario, if Eve finds the result $|\varphi_0\rangle$ in a position $j=M_{\min},\ldots,l-2$ of the block, it is clear that she can always generate a sub-block of the type "01" which includes such signal. This means that, in this case, $|\varphi_0\rangle$ is never replaced with a vacuum signal. On the other hand, if she finds the result $|\varphi_0\rangle$ in a position $j=2,\ldots,M_{\min}-1$ this signal would be replaced by a vacuum signal if all her measurement results corresponding to the positions $j=M_{\min},\ldots,l-2$ are simultaneously different from $|\varphi_0\rangle$, as in this case Eve could not generate a sub-block of the type "01" of length at least $M_{\min}$ which contains the signal $|\varphi_0\rangle$. This requires $l-2-M_{\min}+1=l-M_{\min}-1$ simultaneous results different from $|\varphi_0\rangle$. This is illustrated in Fig. 7. Thus we find that

$$p_{\text{block}|0\rangle|0lj\neq01} = \begin{cases} q_{\text{p}} p(\neq 0|\text{c})^{l-M_{\min}-1} & \text{for } j=2,\ldots,M_{\min}-1, \\ 0 & \text{for } j=M_{\min},\ldots,l-2. \end{cases} \tag{63}$$

Finally, we consider the blocks of the type "$\neq 0 \neq 1$". This scenario is a bit more cumbersome and is shown in Fig. 8. Suppose that Eve finds $|\varphi_0\rangle$ in the second position of the block, *i.e.*, $j=2$ (see Fig. 8(a)). In this case, it is clear that this signal will always be replaced with a vacuum signal as it is not possible for Eve to generate a sub-block of the type "01" which contains it. This means that $p_{\text{block}|0\rangle|0l2\neq0\neq1} = q_{\text{p}}$. Suppose now that Eve finds $|\varphi_0\rangle$ in the position $j=3$ of the block (see Fig. 8(b)). Then, there are two options: her result in the position $j-1=2$ is not equal to $|\varphi_1\rangle$, or it is equal to $|\varphi_1\rangle$. In the former case (see upper subfigure of Fig. 8(b)), we find again that the signal $|\varphi_0\rangle$ will always be replaced with a vacuum signal as it is not possible for Eve to generate a sub-block of the type "01" which contains it. This happens with probability $p(\neq 1|\text{c})$. In the latter case (see lower subfigure of Fig. 8(b)), if $M_{\min}=2$ then we have that the signal $|\varphi_0\rangle$ is never replaced with a vacuum signal, as Eve can always generate a sub-block of the type "01" of length at least $M_{\min}$ which contains such signal. On the other hand, if $M_{\min}>2$, Eve replaces $|\varphi_0\rangle$ with a vacuum signal if none of the last $l-M_{\min}-2$ signals (starting to count from the third signal, beginning at the end of the block, towards the beginning of the block) is equal to $|\varphi_0\rangle$. This is the condition required for Eve not being able to generate a sub-block of the type "01" of length at least $M_{\min}$ which contains the signal $|\varphi_0\rangle$. This last scenario happens with probability $p(1|\text{c})p(\neq 0|\text{c})^{\max\{0,l-M_{\min}-2\}}$ given that $M_{\min}>2$. Note that we need to take the maximum of 0 and $l-M_{\min}-2$ since it is possible that $M_{\min}$

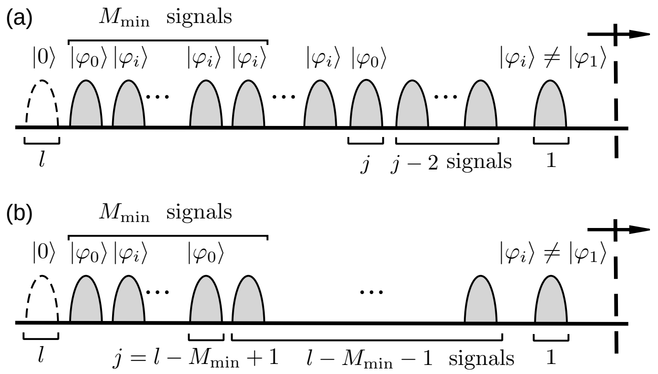


FIG. 6. Possible cases when Eve obtains $|\varphi_0\rangle$ in the $j$th position of the block, with $j = 3, \ldots, l-2$, and the block is of the type "$0 \neq 1$". Here we assume that Eve decides to process the block, which happens with probability $q_{\rm p}$. Case (a): The signal $|\varphi_0\rangle$ is replaced with a vacuum signal by Eve if the previous $j-2$ signals are not equal to $|\varphi_1\rangle$, with $j = 2, \ldots, l - M_{\rm min}$. Case (b): For $j = l - M_{\rm min} + 1, \ldots, l-2$ it is enough that none of the previous $l - M_{\rm min} - 1$ signals is equal to $|\varphi_1\rangle$. This is so because the length of the resulting sub-block (of non-vacuum signals) of the type "01" that Eve would generate is strictly less than $M_{\rm min}$.

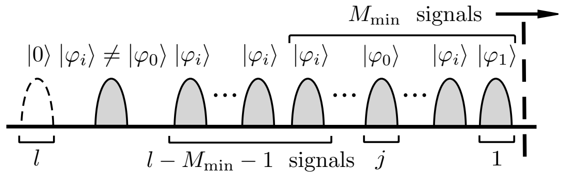


FIG. 7. Possible cases when Eve obtains $|\varphi_0\rangle$ in the $j$th position of the block, with $j = 2, \ldots, l-2$, and the block is of the type "$\neq 01$". Here we assume that Eve decides to process the block, which happens with probability $q_{\rm p}$. Eve only replaces $|\varphi_0\rangle$ with a vacuum signal if $j = 2, \ldots, M_{\rm min} - 1$ and all her measurement results corresponding to the positions $j = M_{\rm min}, \ldots, l - M_{\rm min} - 1$ are simultaneously different from $|\varphi_0\rangle$. This is because in this latter case she could not generate a sub-block of the type "01" of length at least $M_{\rm min}$ which contains the signal $|\varphi_0\rangle$.

is so large (or $l$ is so small) that it is not necessary to have "$\neq 0$" results on the left of the $j$th $|\varphi_0\rangle$ signal to replace it by vacuum, which happens when the bar corresponding to $M_{\rm min}$ on the lower subfigure of Fig. 8(b) contains the $l-1$th signal. In this case the $|\varphi_0\rangle$ signal will be replaced by vacuum irrespective of the signals that come afterwards. We find, therefore, that $p_{{\rm block}|0\rangle|0l3\neq0\neq1} = q_{\rm p} p(\neq 1|{\rm c})$ if $M_{\rm min} = 2$, and $p_{{\rm block}|0\rangle|0l3\neq0\neq1} = q_{\rm p} p(\neq 1|{\rm c}) + q_{\rm p} p(1|{\rm c})\, p(\neq 0|{\rm c})^{\max\{0, l - M_{\rm min} - 2\}}$ if $M_{\rm min} > 2$. In general, it can be shown that for the position $j = 2, \ldots, l-2$, we

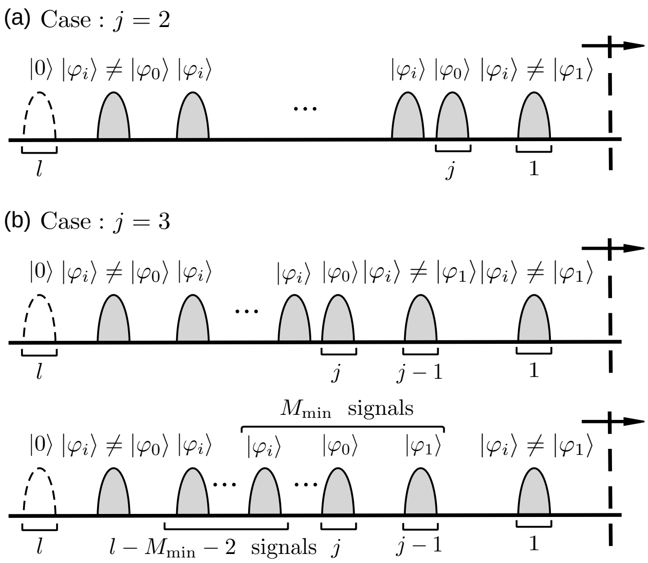


FIG. 8. Possible cases when Eve obtains $|\varphi_0\rangle$ in the $j$th position of the block, with $j = 2$ (Case (a)) and $j = 3$ (Case (b)), and the block is of the type "$\neq 0 \neq 1$". Here we assume that Eve decides to process the block, which happens with probability $q_{\rm p}$. Case (a): Eve always replaces $|\varphi_0\rangle$ with a vacuum signal as she is not able to generate a sub-block of the type "01" of length at least $M_{\rm min}$ which contains the signal $|\varphi_0\rangle$. Case (b) upper subfigure: In this case, Eve's measurement result associated to the signal at the second position of the block is different from $|\varphi_1\rangle$, so, like in the previous scenario, Eve always replaces $|\varphi_0\rangle$ with a vacuum signal. Case (b) lower subfigure: In this case, Eve's result at the second position of the block is $|\varphi_1\rangle$, so, if $M_{\rm min} = 2$, the signal $|\varphi_0\rangle$ is never replaced with a vacuum signal, as Eve can always generate a sub-block of the type "01" of length at least $M_{\rm min}$ which contains such signal. On the other hand, if $M_{\rm min} > 2$, Eve replaces $|\varphi_0\rangle$ with a vacuum signal if none of the last $l - M_{\rm min} - 2$ signals (starting to count from the third signal, beginning at the end of the block, towards the beginning of the block) is equal to $|\varphi_0\rangle$.

have that

$$p_{{\rm block}|0\rangle|0lj\neq0\neq1} = q_{\rm p} p(\neq 1|{\rm c})^{j-2} + q_{\rm p} p(1|{\rm c}) \times \sum_{j'=\max\{2, j - M_{\rm min} + 2\}}^{j-1} p(\neq 1|{\rm c})^{j'-2} \times p(\neq 0|{\rm c})^{\max\{0, l - M_{\rm min} - j'\}}. \quad (64)$$

We note that in the above summation $j'$ represents the position of the first $|\varphi_1\rangle$ signal from the right, preceded by $j'-2$ signals, that are all of type "$\neq 0$". The summation starts at $j' = \max\{2, j - M_{\rm min} + 2\}$ since if the first $|\varphi_1\rangle$ signal from the right is too far away from the $|\varphi_0\rangle$ signal (*i.e.*, $j - (j'-1) \geq M_{\rm min}$) then they form a sub-block of type "01" with length larger or equal than $M_{\rm min}$, therefore the signal is not replaced by vacuum.

To conclude Section IV A 1 b, we need to consider the positions $j = l-1$ and $j = l$ of the block. In the first case, the block can only be of two types: "01" (with probability

$p(1|\mathrm{c})$) or "$0 \neq 1$" (with probability $p(\neq 1|\mathrm{c})$). In the first scenario, the signal $|\varphi_0\rangle$ located in the $l-1$th position of the block is never replaced with a vacuum signal. In the second scenario, the signal $|\varphi_0\rangle$ is replaced with a vacuum signal if and only if Eve decides to process the block (which happens, again, with probability $q_{\mathrm{p}}$) and the first $l - M_{\mathrm{min}} - 1$ positions of the block (starting to count from the second position at the beginning of the block on) are not equal to $|\varphi_1\rangle$. This last condition guarantees that Eve cannot generate a sub-block of the form "01" containing at least $M_{\mathrm{min}}$ non-vacuum signals.

In short, we have that

$$p_{\mathrm{block}|0\rangle|0ll-1} = q_{\mathrm{p}} p(\neq 1|\mathrm{c})^{l-M_{\mathrm{min}}}. \tag{65}$$

Finally, regarding the position $j = l$, we have that Eve cannot obtain the result $|\varphi_0\rangle$ in that position of the block as $p_{l|0l} = 0$.

By combining Eq. (53)-(54)-(60)-(61)-(62)-(63)-(64)-(65), and taking into account that the probability of a block being of the type "$0 \neq 1$", "$\neq 01$" and "$\neq 0 \neq 1$" is given by Eq. (26), we find that for $M_{\mathrm{min}} + 1 < l \leq M_{\mathrm{max}} + 1$ we have that

$$\begin{aligned} p_{\mathrm{block}|0\rangle|0l} = \frac{q_{\mathrm{p}}}{l-1}\Bigg[&1 + q_{0\neq 1}\sum_{j=2}^{l-M_{\mathrm{min}}} p(\neq 1|\mathrm{c})^{j-2} + q_{0\neq 1}\sum_{j=l-M_{\mathrm{min}}+1}^{l-2} p(\neq 1|\mathrm{c})^{l-M_{\mathrm{min}}-1} + q_{\neq 01}\sum_{j=2}^{M_{\mathrm{min}}-1} p(\neq 0|\mathrm{c})^{l-M_{\mathrm{min}}-1} \\ &+ q_{\neq 0\neq 1}\sum_{j=2}^{l-2} p(\neq 1|\mathrm{c})^{j-2} + q_{\neq 0\neq 1} p(1|\mathrm{c})\sum_{j=2}^{l-2}\sum_{j'=\max\{2,j-M_{\mathrm{min}}+2\}}^{j-1} p(\neq 1|\mathrm{c})^{j'-2} p(\neq 0|\mathrm{c})^{\max\{0,l-M_{\mathrm{min}}-j'\}} \\ &+ p(\neq 1|\mathrm{c})^{l-M_{\mathrm{min}}}\Bigg]. \end{aligned} \tag{66}$$

*c. Probabilities $p_{(l|0)}$* To evaluate Eq. (52), we now calculate the probabilities $p_{(l|0)}$ with $M_{\mathrm{min}} + 1 \leq l \leq M_{\mathrm{max}} + 1$. These probabilities can be expressed as

$$p_{(l|0)} = \sum_{j=1}^{l} p_{(j,l|0)}, \tag{67}$$

where $p_{(j,l|0)}$ denotes the conditional probability that, given that Eve obtained the result $|\varphi_0\rangle$, this corresponds to the $j$th position of a block of length $l$.

We start with the case $M_{\mathrm{min}} + 1 \leq l < M_{\mathrm{max}} + 1$. This scenario is illustrated in Fig. 9. Suppose that Eve obtains the measurement result $|\varphi_0\rangle$ at a certain time instance. Then, this signal occupies the first position of a block of length $l$ (see Fig. 9(a)), if and only if: (i) in the time instance corresponding to the previous signal (which is indicated in Fig. 9(a) as time instance "0") Eve sent Bob a vacuum signal (which happens with probability $p_{|0\rangle}$ defined below), and (ii) her next $l-2$ measurement results are all conclusive (which happens with probability $p_{\mathrm{c}}^{l-2}$), and (iii) her $l$th measurement result is inconclusive (which happens with probability $1-p_{\mathrm{c}}$). Putting this together, we have that $p_{(1,l|0)} = (1-p_{\mathrm{c}})p_{\mathrm{c}}^{l-2}p_{|0\rangle}$. Similarly, it is straightforward to show that

$$p_{(j,l|0)} = \begin{cases} (1-p_{\mathrm{c}})p_{\mathrm{c}}^{l-2}p_{|0\rangle} & \text{for } j = 1,\ldots,l-1, \\ 0 & \text{for } j = l. \end{cases} \tag{68}$$

In the asymptotic scenario where Alice sends Bob an infinite number of signals, there are infinite possible events that contribute to the probability $p_{|0\rangle}$. This is illustrated in Fig. 10. For instance, Eve could obtain an inconclusive result in the time instance "0" precisely before the start of the block (see Fig. 10(a)), which happens with probability $1-p_{\mathrm{c}}$. Alternatively, it is possible that Eve does not measure the signal in the time instance "0" but replaces it by vacuum if she has obtained $M_{\mathrm{max}}$ consecutive conclusive results and an inconclusive result in the time instance corresponding to the $M_{\mathrm{max}}+1$th signal (see Fig. 10(b)) preceding the time instance "0". This happens with probability $(1-p_{\mathrm{c}})p_{\mathrm{c}}^{M_{\mathrm{max}}}$. Similarly, it is also possible that Eve does not measure the signal in the time instance "0" but automatically replaces it by vacuum if the time instance "0" is preceded by $M_{\mathrm{max}}$ consecutive conclusive results together with a signal that has also been automatically replaced (not measured) by vacuum in the time instance corresponding to the preceding $M_{\mathrm{max}}+1$th signal, thus preceded by $M_{\mathrm{max}}$ additional consecutive conclusive results, and an inconclusive result in the time instance corresponding to the preceding $2M_{\mathrm{max}}+2$th signal (see Fig. 10(c)); and so on. This latter scenario happens with probability $(1-p_{\mathrm{c}})p_{\mathrm{c}}^{2M_{\mathrm{max}}}$. This means that we can write $p_{|0\rangle}$ as

$$p_{|0\rangle} = (1-p_{\mathrm{c}})\sum_{i=0}^{\infty} p_{\mathrm{c}}^{iM_{\mathrm{max}}} = \frac{1-p_{\mathrm{c}}}{1-p_{\mathrm{c}}^{M_{\mathrm{max}}}}. \tag{69}$$

By combining Eqs. (67)-(68)-(69), this means that

$$p_{(l|0)} = \frac{(l-1)(1-p_{\mathrm{c}})^2 p_{\mathrm{c}}^{l-2}}{1-p_{\mathrm{c}}^{M_{\mathrm{max}}}}, \tag{70}$$

when $M_{\mathrm{min}} + 1 \leq l < M_{\mathrm{max}} + 1$.

The case $p_{(M_{\mathrm{max}}+1|0)}$ is also similar. The only difference is that here Eve does not measure in the $M_{\mathrm{max}}+1$th position of the block as she will automatically replace this

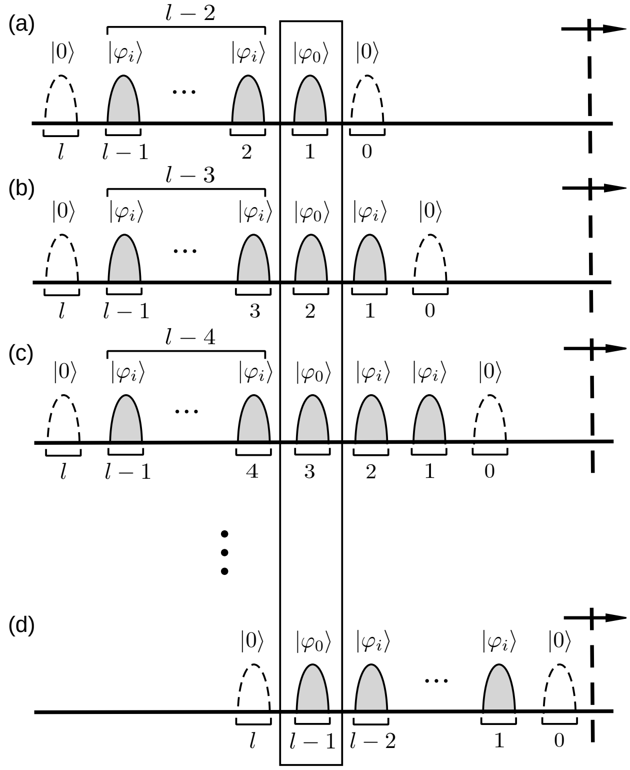


FIG. 9. Illustration of the different cases where Eve's result $|\varphi_0\rangle$ is included in a block of size $l$ (which contains $l-1$ non-vacuum signals), with $M_{\min}+1 \leq l \leq M_{\max}+1$. Case (a): The signal $|\varphi_0\rangle$ occupies the first position of the block if in the previous time instance "0" Eve sent Bob a vacuum signal, in the following $l-2$ time instances (*i.e.*, the time instances that go from "2" till "$l-1$") Eve obtains a conclusive result (indicated in the figure with $|\varphi_i\rangle$, though the actual non-vacuum quantum signal can be different for each time instance), and Eve's $l$th measurement result is inconclusive. Case (b): The signal $|\varphi_0\rangle$ occupies the second position of the block if in the time instance "0" Eve sent Bob a vacuum signal, in the previous time instance "1" and in the following $l-3$ time instances (*i.e.*, the time instances that go from "3" till "$l-1$") Eve obtains a conclusive result, and Eve's $l$th measurement result is inconclusive or when $l = M_{\max}+1$ then this signal is replaced by vacuum without measuring. The other cases are analogous. In total there are $l-1$ cases.

signal with a vacuum signal after obtaining $M_{\max}$ consecutive conclusive results, therefore in this position she cannot get an inconclusive result. To be precise, we have that

$$p_{(j,M_{\max}+1|0)} = \begin{cases} p_{\rm c}^{M_{\max}-1} p_{|0\rangle} & \text{for } j = 1,\ldots,M_{\max} \\ 0 & \text{for } j = M_{\max}+1. \end{cases} \tag{71}$$

This means that

$$p_{(M_{\max}+1|0)} = \frac{(1-p_{\rm c}) M_{\max} p_{\rm c}^{M_{\max}-1}}{1-p_{\rm c}^{M_{\max}}}. \tag{72}$$

Finally, by using Eqs. (52)-(70)-(72) one can directly calculate the probability $p_{{\rm block}|\varphi_0\rangle|0}$,

$$\begin{aligned} p_{{\rm block}|\varphi_0\rangle|0} = \frac{(1-p_{\rm c}) p_{\rm c}^{M_{\min}-1}}{1-p_{\rm c}^{M_{\max}}} \Big\{ & M_{\min}(1-p_{\rm c}) \Big[1 - p_{{\rm block}|0\rangle|0 M_{\min}+1}\Big] + \frac{p_{\rm c}}{1-p_{\rm c}} \left(1 - p_{\rm c}^{M_{\max}-M_{\min}}\right) \\ & + p_{\rm c} \left(M_{\min} - M_{\max} p_{\rm c}^{M_{\max}-M_{\min}-1}\right) - (1-p_{\rm c}) \sum_{l=M_{\min}+2}^{M_{\max}} (l-1) p_{\rm c}^{l-M_{\min}-1} p_{{\rm block}|0\rangle|0l} \\ & + M_{\max} p_{\rm c}^{M_{\max}-M_{\min}} \Big[1 - p_{{\rm block}|0\rangle|0 M_{\max}+1}\Big] \Big\}, \end{aligned} \tag{73}$$

where the probabilities $p_{{\rm block}|0\rangle|0M_{\min}+1}$ and $p_{{\rm block}|0\rangle|0l}$, with $M_{\min}+1 < l \leq M_{\max}+1$ are given, respectively, by Eqs. (59)-(66).

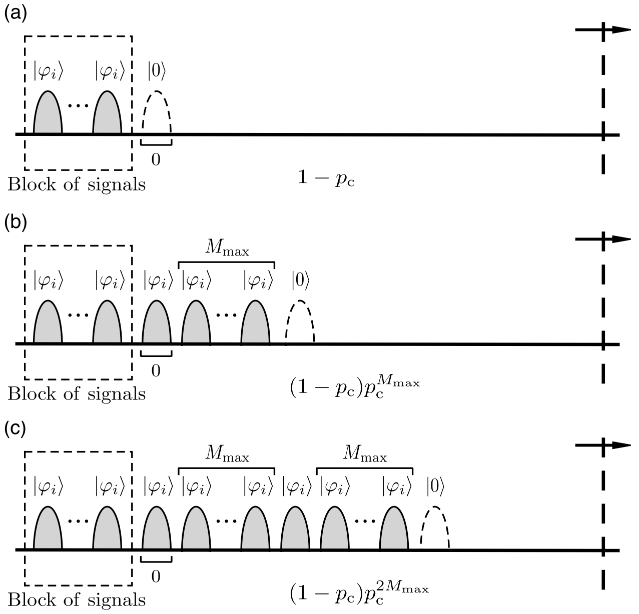

FIG. 10. Illustration of different cases that contribute to the calculation of the probability $p_{|0\rangle}$. (a) Eve could obtain an inconclusive result in the time instance "0", which happens with probability $1-p_{\rm c}$. (b) Alternatively, she could automatically replace the signal in the time instance "0" by vacuum if it is preceded by $M_{\rm max}$ consecutive conclusive results and an inconclusive result in the time instance corresponding to the previous $M_{\rm max}+1$th signal, which happens with probability $(1-p_{\rm c})p_{\rm c}^{M_{\rm max}}$. (c) Also, Eve could automatically replace the signal in the time instance "0" by vacuum if it is preceded by $M_{\rm max}$ consecutive conclusive results and also a signal that has been automatically replaced by vacuum (thus not measured) in the time instance corresponding to the preceding $M_{\rm max}+1$th signal, which is also preceded by $M_{\rm max}$ consecutive conclusive results, and an inconclusive result in the time instance corresponding to the previous $2M_{\rm max}+2$th signal; and so on. This latter scenario happens with probability $(1-p_{\rm c})p_{\rm c}^{2M_{\rm max}}$.

### 2. $p_{{\rm block}|\varphi_1\rangle|1}$

The analysis to determine the probability $p_{{\rm block}|\varphi_1\rangle|1}$ is similar to that of the previous section, and we omit it here for simplicity. Indeed, it can be shown that since all the probabilities associated to the signal $|\varphi_1\rangle$ are equal to those of the signal $|\varphi_0\rangle$, and, moreover, if Eve decides to process the blocks of signals then her goal is to generate blocks of the type "01", we have that

$$p_{{\rm block}|\varphi_1\rangle|1}=p_{{\rm block}|\varphi_0\rangle|0}. \tag{74}$$

### 3. $p_{{\rm block}|\varphi_2\rangle|2}$

Like in the case $p_{{\rm block}|\varphi_0\rangle|0}$, below we calculate the probabilities $p_{{\rm block}|0\rangle|2lj}$ and $p_{(l|2)}$, which are needed to obtain $p_{{\rm block}|\varphi_2\rangle|2}$ by using Eqs. (52)-(53)-(54).

*a. Probability $p_{{\rm block}|0\rangle|2M_{\rm min}+1}$* When the length of the block is $M_{\rm min}+1$, we have that Eve sends Bob a block of $M_{\rm min}+1$ vacuum signals with probability $1-q$, while with probability $q$ she tries to process the block further. Analogously to Eq. (55), this means that

$$p_{{\rm block}|0\rangle|2M_{\rm min}+1}=(1-q)+q\sum_{j=1}^{M_{\rm min}+1}p_{j|2M_{\rm min}+1}\times p_{{\rm block}|0\rangle|2M_{\rm min}+1j}. \tag{75}$$

Let us now consider the probabilities $p_{{\rm block}|0\rangle|2M_{\rm min}+1j}$. If $j=1$, *i.e.*, if Eve's result $|\varphi_2\rangle$ corresponds to the first position of the block, the block is not of the type "01", and thus

$$p_{{\rm block}|0\rangle|2M_{\rm min}+11}=q_{\rm p}. \tag{76}$$

Similarly, if Eve's result corresponds to a position $j=2,\ldots,M_{\rm min}-1$, we have that the block is not of the type "01" with probability $1-q_{01}$, with $q_{01}$ given by Eq. (26). This means that

$$p_{{\rm block}|0\rangle|2M_{\rm min}+1j}=(1-q_{01})q_{\rm p}, \tag{77}$$

when $1<j<M_{\rm min}$.

On the other hand, if $j=M_{\rm min}$, the block is again not of the type "01", and thus

$$p_{{\rm block}|0\rangle|2M_{\rm min}+1M_{\rm min}}=q_{\rm p}. \tag{78}$$

Finally, we have that Eve cannot obtain the result $|\varphi_2\rangle$ in the position $j=M_{\rm min}+1$, because in that position she obtained an inconclusive result.

By substituting Eqs. (54)-(76)-(77)-(78) into Eq. (111), we obtain

$$p_{{\rm block}|0\rangle|2M_{\rm min}+1}=(1-q)+\frac{qq_{\rm p}}{M_{\rm min}}\big[2+(M_{\rm min}-2)\times(1-q_{01})\big]. \tag{79}$$

*b. Probabilities $p_{{\rm block}|0\rangle|2lj}$ with $M_{\rm min}+1<l\leq M_{\rm max}+1$* The analysis is analogous to that of $p_{{\rm block}|0\rangle|0lj}$. In particular, if Eve obtains $|\varphi_2\rangle$ in the first position of the block, the block is obviously not of the type "01". Therefore, if Eve tries to process it (which happens with probability $q_{\rm p}$), she will always send Bob a vacuum signal in the first position of the block, *i.e.*,

$$p_{{\rm block}|0\rangle|2l1}=q_{\rm p}. \tag{80}$$

On the other hand, if Eve obtains $|\varphi_2\rangle$ in a position $j=2,\ldots,l-2$ of the block, her strategy depends on whether the block is of the type "$0\neq1$", "$\neq01$" or "$\neq0\neq1$". Eq. (61) can be rewritten in this scenario as

$$p_{{\rm block}|0\rangle|2lj}=\sum_{i'j'\in\Delta}q_{i'j'}p_{{\rm block}|0\rangle|2lji'j'}. \tag{81}$$

Suppose that the block is of the type "$0\neq1$". Then, if Eve's result corresponds to the second position of the

block and she decides to process the block, she always sends Bob a vacuum signal in that position. That is, we have that $p_{\text{block}|0\rangle|2l20\neq 1} = q_{\text{p}}$.

Similarly, if $j = 3, \ldots, l-2$, Eve sends Bob a vacuum signal (instead of the signal $|\varphi_2\rangle$) if in the previous $j-2$ positions there is no signal $|\varphi_1\rangle$, or if the number of non-vacuum signals within the resulting modified block is strictly less than $M_{\min}$. This means that

$$p_{\text{block}|0\rangle|2lj0\neq 1} = p_{\text{block}|0\rangle|0lj0\neq 1}, \tag{82}$$

with $j = 2, \ldots, l-2$, and $p_{\text{block}|0\rangle|0lj0\neq 1}$ given by Eq. (62).

Suppose now that the block is of the type "$\neq 01$". If Eve finds the result $|\varphi_2\rangle$ in a position $j = 2, \ldots, M_{\min}-1$ of the block, this signal would be replaced by a vacuum signal if all her measurement results corresponding to the positions $j = M_{\min}, \ldots, l-2$ are simultaneously different from $|\varphi_0\rangle$, as in this case Eve could not generate a sub-block of the type "01" of length at least $M_{\min}$ which contains the signal $|\varphi_2\rangle$. On the other hand, if Eve finds the result $|\varphi_2\rangle$ in a position $j = M_{\min}, \ldots, l-2$ of the block, this signal would be replaced by a vacuum signal if all her measurement results corresponding to the positions $j' = j+1, \ldots, l-2$ are simultaneously different from $|\varphi_0\rangle$ for the same reasons as in the previous case. This means $l-2-(j+1)+1 = l-j-2$ simultaneous results different from $|\varphi_0\rangle$. Thus we find that

$$p_{\text{block}|0\rangle|2lj\neq 01} = \begin{cases} q_{\text{p}} p(\neq 0|\text{c})^{l-M_{\min}-1} & \text{for } j = 2, \ldots, M_{\min}-1, \\ q_{\text{p}} p(\neq 0|\text{c})^{l-j-2} & \text{for } j = M_{\min}, \ldots, l-2. \end{cases} \tag{83}$$

Finally, we consider the blocks of the type "$\neq 0 \neq 1$". If Eve finds $|\varphi_2\rangle$ in the second position of the block, then this signal will always be replaced with a vacuum signal because Eve cannot generate a sub-block of the type "01" which contains it. That is, we have that $p_{\text{block}|0\rangle|2l2\neq 0\neq 1} = q_{\text{p}}$. If Eve finds $|\varphi_2\rangle$ in the position $j = 3$ of the block, there are two options: if the signal in the position $j = 2$ is not equal to $|\varphi_1\rangle$, or it is equal to $|\varphi_1\rangle$. In the former case (which happens with probability $p(\neq 1|\text{c})$), the signal $|\varphi_2\rangle$ is replaced with a vacuum signal as it is not possible for Eve to generate a sub-block of the type "01" which contains it. In the latter case, there are again two possibilities depending on the value of $M_{\min}$. If $M_{\min} = 2$, Eve replaces the signal $|\varphi_2\rangle$ with a vacuum signal if none of the remaining $l-5$ signals is in the state $|\varphi_0\rangle$ (which happens with probability $p(\neq 0|\text{c})^{l-5}$). Note that here we have to consider $l-5$ signals because from the $l$ total number of pulses of the block we need to discard the first position (which, by assumption, is not equal to $|\varphi_1\rangle$), the second and third positions of the block (which, by assumption, are in the states $|\varphi_1\rangle$ and $|\varphi_2\rangle$, respectively), and the last two signals of the block (which, by assumption, are in a state different from $|\varphi_0\rangle$ and are a vacuum signal, respectively). If $M_{\min} > 2$, however, Eve replaces the signal $|\varphi_2\rangle$ with a vacuum signal if none of the last $l - M_{\min} - 2$ signals of the block (starting to count from the third signal, beginning at the end of the block, *i.e.*, the signal at the position $l-2$, towards the beginning of the block) is in the state $|\varphi_0\rangle$ (which happens with probability $p(\neq 0|\text{c})^{l-M_{\min}-2}$). This last condition guarantees that Eve cannot generate a sub-block of the type "01" of length at least $M_{\min}$ which contains $|\varphi_2\rangle$. Putting all these conditions together, we find that Eve replaces $|\varphi_2\rangle$ with a vacuum signal with probability given by

$$p_{\text{block}|0\rangle|2l3\neq 0\neq 1} = q_{\text{p}} p(\neq 1|\text{c}) + q_{\text{p}} p(1|\text{c}) \times p(\neq 0|\text{c})^{\max\{0, l-\max\{M_{\min},3\}-2\}}. \tag{84}$$

Similarly to $p_{\text{block}|0\rangle|0l3\neq 0\neq 1}$, given by Eq. (64), we need to take the maximum of 0 and $l - \max\{M_{\min}, 3\} - 2$ since it is possible that $M_{\min}$ is so large (or $l$ is so small) that it is not necessary to have any "$\neq 0$" results on the left of the $j$th (in this case $j = 3$) $|\varphi_2\rangle$ signal to replace it by vacuum, which, similarly to $p_{\text{block}|0\rangle|0l3\neq 0\neq 1}$, happens when the $M_{\min}-1$th signal to the left from the $|\varphi_1\rangle$ signal is at a position $\geq l-1$. In this case the $|\varphi_2\rangle$ signal will be replaced by vacuum irrespective of the signals that come afterwards.

In general, it can be shown that for the position $j = 2, \ldots, l-3$, we have that

$$p_{\text{block}|0\rangle|2lj\neq 0\neq 1} = q_{\text{p}} p(\neq 1|\text{c})^{j-2} + q_{\text{p}} p(1|\text{c}) \times \sum_{j'=2}^{j-1} p(\neq 1|\text{c})^{j'-2} \times p(\neq 0|\text{c})^{\max\{0, l-\max\{M_{\min}, j-j'+2\}-j'\}}. \tag{85}$$

The case $j = l-2$ is equal to the case $j = 2$, as in this situation Eve can never generate a sub-block of the type "01" which contains the signal $|\varphi_2\rangle$. This means, therefore, that

$$p_{\text{block}|0\rangle|2ll-2\neq 0\neq 1} = q_{\text{p}}. \tag{86}$$

To finish Section IV A 3 b, we now study the positions $j = l-1$ and $j = l$ of the block. In the first case, the block cannot be transformed into a block of the form

"01" which contains the signal $|\varphi_2\rangle$. We have, therefore, that

$$p_{\text{block}|0\rangle|2ll-1} = q_{\text{p}}. \tag{87}$$

In the second case, note that Eve cannot find $|\varphi_2\rangle$ in that position of the block because $p_{l|2l} = 0$.

By combining Eq. (53)-(54)-(80)-(82)-(83)-(85)-(86), and taking into account that the probability of a block being of the type "$0 \neq 1$", "$\neq 01$" and "$\neq 0 \neq 1$" is given by Eq. (26), we find that for $M_{\min} + 1 < l \leq M_{\max} + 1$ we have that

$$p_{\text{block}|0\rangle|2l} = \frac{q_{\text{p}}}{l-1}\Bigg[2 + q_{0\neq 1}\sum_{j=2}^{l-M_{\min}} p(\neq 1|\text{c})^{j-2} + q_{0\neq 1}\sum_{j=l-M_{\min}+1}^{l-2} p(\neq 1|\text{c})^{l-M_{\min}-1} + q_{\neq 01}\sum_{j=2}^{M_{\min}-1} p(\neq 0|\text{c})^{l-M_{\min}-1}$$
$$+ q_{\neq 01}\sum_{j=M_{\min}}^{l-2} p(\neq 0|\text{c})^{l-j-2} + q_{\neq 0\neq 1}\sum_{j=2}^{l-3} p(\neq 1|\text{c})^{j-2} + q_{\neq 0\neq 1}p(1|\text{c})\sum_{j=2}^{l-3}\sum_{j'=2}^{j-1} p(\neq 1|\text{c})^{j'-2}$$
$$\times p(\neq 0|\text{c})^{\max\{0,l-\max\{M_{\min},j-j'+2\}-j'\}} + q_{\neq 0\neq 1}\Bigg]. \tag{88}$$

*c. Probability $p_{(l|2)}$ with $M_{\min} + 1 \leq l \leq M_{\max} + 1$* The analysis is exactly the same as that used to determine $p_{(l|0)}$, being straightforward to show that

$$p_{(l|2)} = p_{(l|0)}, \tag{89}$$

with $M_{\min} + 1 \leq l \leq M_{\max} + 1$, and where $p_{(l|0)}$ is given by Eqs. (70)-(72) for $M_{\min} + 1 \leq l < M_{\max} + 1$ and $l = M_{\max} + 1$, respectively.

By using Eqs. (52)-(70)-(72) we obtain, therefore that $p_{\text{block}|\varphi_2\rangle|2}$ can be expressed as

$$p_{\text{block}|\varphi_2\rangle|2} = \frac{(1-p_{\text{c}})p_{\text{c}}^{M_{\min}-1}}{1-p_{\text{c}}^{M_{\max}}}\Bigg\{M_{\min}(1-p_{\text{c}})\Big[1-p_{\text{block}|0\rangle|2M_{\min}+1}\Big] + \frac{p_{\text{c}}}{1-p_{\text{c}}}\left(1-p_{\text{c}}^{M_{\max}-M_{\min}}\right)$$
$$+ p_{\text{c}}\left(M_{\min} - M_{\max}p_{\text{c}}^{M_{\max}-M_{\min}-1}\right) - (1-p_{\text{c}})\sum_{l=M_{\min}+2}^{M_{\max}}(l-1)p_{\text{c}}^{l-M_{\min}-1}p_{\text{block}|0\rangle|2l}$$
$$+ M_{\max}p_{\text{c}}^{M_{\max}-M_{\min}}\Big[1-p_{\text{block}|0\rangle|2M_{\max}+1}\Big]\Bigg\}, \tag{90}$$

where the probabilities $p_{\text{block}|0\rangle|2M_{\min}+1}$ and $p_{\text{block}|0\rangle|2l}$, with $M_{\min} + 1 < l \leq M_{\max} + 1$ are given, respectively, by Eqs. (79)-(88).

## V. VISIBILITIES

In this Section we introduce the calculations to determine the value of the visibilities $V_d$ and $V_{01}$. The visibilities $V_{0d}$, $V_{d1}$ and $V_{dd}$ can be obtained following exactly the same procedure used to determine $V_{01}$, and we omit the explicit calculations here for simplicity.

As introduced already in the main text, in general the visibility is defined as

$$V_s = \frac{p_{\text{click}}(\text{D}_{\text{M1}}|s) - p_{\text{click}}(\text{D}_{\text{M2}}|s)}{p_{\text{click}}(\text{D}_{\text{M1}}|s) + p_{\text{click}}(\text{D}_{\text{M2}}|s)}, \tag{91}$$

with $s \in \{$"$d$", "01", "0$d$", "$d$1", "$dd$"$\}$, and where $p_{\text{click}}(\text{D}_{\text{M}i}|s)$, with $i = 1, 2$, denotes the the conditional probability that the detector $\text{D}_{\text{M}i}$ within Bob's monitor line observes a click in the time instance where the interference occurs given that Alice sends Bob the signal (or combination of signals) indicated by $s$.

### A. Visibility $V_d$

This case corresponds to the scenario where Alice sends Bob a decoy signal, *i.e.*, she sends him the signal $|\varphi_2\rangle \equiv |\alpha\rangle|\alpha\rangle$ (see Eq. (1)). The goal of this visibility is to evaluate the interference between the two coherent pulses $|\alpha\rangle$ that form the signal $|\varphi_2\rangle$. In the ideal noiseless scenario, we have that the Mach-Zehnder interferometer at Bob's monitoring line is designed such that the detector $\text{D}_{\text{M2}}$ never clicks when interfering two coherent pulses $|\alpha\rangle$ (and, thus, $V_d = 1$).

Below we calculate $V_d$ in the presence of Eve's attack. For this, we first note that the probabilities $p_{\text{click}}(\text{D}_{\text{M}i}|d)$,

which are required to calculate $V_d$, can be written as

$$p_{\rm click}({\rm D}_{{\rm M}i}|d)=\sum_{j=0}^{2}p_{j|2}p_{{\rm block}|\varphi_j\rangle|j}p_{\rm click}({\rm D}_{{\rm M}i}|\,|\varphi_j\rangle),\quad (92)$$

where $p_{j|2}$ denotes the conditional probability that Eve's measurement result is the state $|\varphi_j\rangle$ given that Alice sent Bob the state $|\varphi_2\rangle$ (these probabilities are given by Eq. (3) and Table I), $p_{{\rm block}|\varphi_j\rangle|j}$ is the probability that Eve actually sends the signal $|\varphi_j\rangle$ to Bob in a block of signals, *i.e.*, without replacing it with a vacuum signal (see Section IV A), and $p_{\rm click}({\rm D}_{{\rm M}i}|\,|\varphi_j\rangle)$ is the conditional probability that detector $\rm D_{Mi}$ clicks in the time instance corresponding to interference given that Eve sent Bob the signal $|\varphi_j\rangle$. Note that if Eve's measurement result is $|\varphi_j\rangle$, with $j=0,1,2$, she always sends Bob either this signal or a vacuum signal, *i.e.*, we have that $p_{{\rm block}|\varphi_{j'}\rangle|j}=0$ for all $j'\neq j$. This is the reason why these cases are not included in Eq. (92).

This means that to evaluate Eq. (92) we only need to calculate the probabilities $p_{\rm click}({\rm D}_{{\rm M}i}|\,|\varphi_j\rangle)$, as all the other parameters have already been calculated in Sections II and IV A. This is what we do next. In particular, we have that

$$\begin{aligned}
&p_{\rm click}({\rm D}_{\rm M1}|\,|\varphi_0\rangle)=\gamma,\\
&p_{\rm click}({\rm D}_{\rm M2}|\,|\varphi_0\rangle)=p_{\rm click}({\rm D}_{\rm M1}|\,|\varphi_0\rangle),\\
&p_{\rm click}({\rm D}_{\rm M1}|\,|\varphi_1\rangle)=p_{\rm click}({\rm D}_{\rm M1}|\,|\varphi_0\rangle),\\
&p_{\rm click}({\rm D}_{\rm M2}|\,|\varphi_1\rangle)=p_{\rm click}({\rm D}_{\rm M1}|\,|\varphi_0\rangle),\\
&p_{\rm click}({\rm D}_{\rm M1}|\,|\varphi_2\rangle)=\lambda,\\
&p_{\rm click}({\rm D}_{\rm M2}|\,|\varphi_2\rangle)=0,
\end{aligned}\qquad (93)$$

where the parameters $\gamma$ and $\lambda$ are given by

$$\begin{aligned}
\gamma&=\frac{1}{2}\Big[1-e^{-\frac{1}{2}(1-t_{\rm B})\eta_{\rm DM}|\beta|^2}\Big],\\
\lambda&=1-e^{-(1-t_{\rm B})\eta_{\rm DM}|\beta|^2}.
\end{aligned}\qquad (94)$$

Here, $|\beta|^2$ is again the intensity of Eve's sending coherent states and $\eta_{\rm DM}$ is a parameter that takes into account the fact that the detection efficiency of the detector in the data line and those in the monitoring line at Bob's side might be different. To be precise, if the detection efficiency of Bob's detector in the data (monitoring) line is $\eta_{\rm D}$ ($\eta_{\rm M}$), with say $\eta_{\rm D}\geq\eta_{\rm M}$, then the parameter $\eta_{\rm DM}$ is defined as

$$\eta_{\rm DM}=\frac{\eta_{\rm M}}{\eta_{\rm D}}.\qquad (95)$$

This definition is motivated by the fact that in the untrusted device scenario one typically assumes that Eve might control the detection efficiency of Bob's measurement unit and make this efficiency equal to one if she wishes so. However, if Bob's detectors in the monitoring and data lines have different detection efficiencies, it might happen that Eve can control only partially the detection efficiency of that detector which has the lowest detection efficiency (say, for example, that in the monitoring line as assumed above). Note that a detector in the data/monitoring line with finite detection efficiency can always be modeled with a beamsplitter (with transmittance equal to its detection efficiency) followed by a unit detection efficiency detector. With this model, and in a second step, the beamsplitter of the detector in the data line (which by assumption has the higher detection efficiency) can be placed outside Bob's measuring unit (*i.e.*, it now affects all detectors) and then give its control to Eve, while the beamsplitter that models the loss in the detector in the monitoring line must have now transmittance $\eta_{\rm DM}$, such that the overall transmittance of the monitoring line is indeed $\eta_{\rm M}$.

Also, note that in Eq. (93) we assigned double clicks in detectors $\rm D_{M1}$ and $\rm D_{M2}$ to single clicks at random.

By combining Eqs. (92)-(93) as well as Table I, and by taking into account that $p_{{\rm block}|\varphi_1\rangle|1}=p_{{\rm block}|\varphi_0\rangle|0}$, we find that

$$\begin{aligned}
&p_{\rm click}({\rm D}_{\rm M1}|d)=2q_{\rm f}p_{{\rm block}|\varphi_0\rangle|0}\gamma+q_{\rm s}p_{{\rm block}|\varphi_2\rangle|2}\lambda,\\
&p_{\rm click}({\rm D}_{\rm M2}|d)=2q_{\rm f}p_{{\rm block}|\varphi_0\rangle|0}\gamma.
\end{aligned}\qquad (96)$$

By substituting these values in Eq. (91), with $s=d$, we finally obtain

$$V_d=\frac{q_{\rm s}p_{{\rm block}|\varphi_2\rangle|2}\lambda}{4q_{\rm f}p_{{\rm block}|\varphi_0\rangle|0}\gamma+q_{\rm s}p_{{\rm block}|\varphi_2\rangle|2}\lambda},\qquad (97)$$

where, as already mentioned, the probabilities $p_{{\rm block}|\varphi_j\rangle|j}$ have been calculated in Section IV A.

### B. Visibility $V_{01}$

The calculations to obtain this visibility are more cumbersome than those of $V_d$ because here we have to take into account two consecutive signals sent by Alice (instead of only one, as is the case in $V_d$).

Let us start by introducing some notation first. In particular, we will distinguish between three different types of blocks of signals that Eve sends to Bob (and which contain non-vacuum signals). The first type, which we will denote as "b1", refers to those blocks of signals which are directly of the type "01" without performing any processing on them. Whenever Eve obtains one of these blocks of signals she always sends it to Bob. The second type, which we will denote as "b2", refers to those blocks of signals which are not of the type "01" (without performing any processing on them) but Eve sends them to Bob anyway, which happens with probability $1-q_{\rm p}$. Finally, the third type, which we will denote as "b3", refers to those blocks of signals which are of the type "01" but only after performing some processing on them.

In addition, we will consider five posible positions (with respect to the blocks of signals generated by Eve) for the combination of signals $|\varphi_0\rangle\otimes|\varphi_1\rangle$ prepared by Alice. These positions are illustrated in Fig. 11. For example, the first position (which is shown in Fig. 11(a))

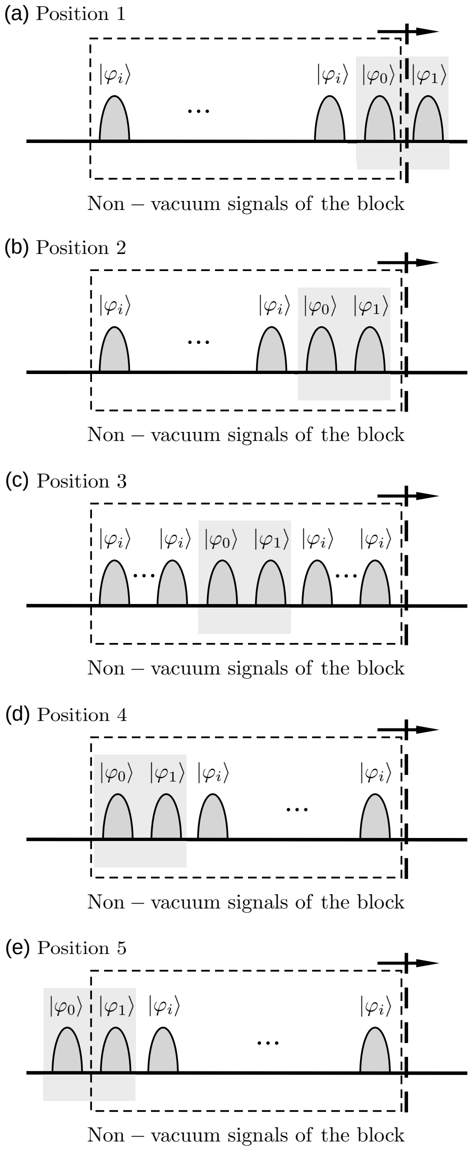


FIG. 11. Possible positions that the combination of signals $|\varphi_0\rangle \otimes |\varphi_1\rangle$ prepared by Alice can occupy with respect to the blocks of signals generated by Eve. For instance, subfigure (a) shows the scenario where $|\varphi_1\rangle$ occupies the last position of a block of signals generated by Eve (and, thus, $|\varphi_1\rangle$ will be necessarily replaced by Eve with a vacuum signal before she sends it to Bob), while the signal $|\varphi_0\rangle$ occupies the first position of the next block of signals. Note that depending on Eve's measurement result, $|\varphi_0\rangle$ might also be replaced by Eve with other signal before she sends it to Bob. Subfigure (b), on the other hand, refers to the situation where the signal $|\varphi_1\rangle$ ($|\varphi_0\rangle$) occupies the first (second) position of a block of signals generated by Eve. Again, both signals might be replaced with other signals before Eve sends them to Bob depending on her measurement results. The description of the other subfigures is analogous and we omit it here for simplicity.

describes the scenario where the signal $|\varphi_1\rangle$ ends up as the last signal of a block generated by Eve (and, thus, $|\varphi_1\rangle$ will be necessarily replaced with a vacuum signal before she sends it to Bob), while the signal $|\varphi_0\rangle$ is the first signal of the next block generated by Eve. Of course, depending on Eve's measurement result, the signal $|\varphi_0\rangle$ might also be replaced by Eve with other signal before she sends it to Bob. The second position (which is shown in Fig. 11(b)) refers to the situation where the signal $|\varphi_1\rangle$ ($|\varphi_0\rangle$) occupies the first (second) position of the block of signals generated by Eve. Again, depending on Eve's measurement results when measuring these two signals, they could be replaced by other signals before she sends them to Bob. The description of the other cases illustrated in Fig. 11 is analogous and can be inferred from the figure.

With the definitions above, we have that the probability $p_{\text{click}}(\text{D}_{\text{M}i}|01)$ can be expressed as

$$p_{\text{click}}(\text{D}_{\text{M}i}|01) = \sum_{j\in\Omega}\sum_{k=1}^{5} p_{(j,k|01)} p_{\text{click}}(\text{D}_{\text{M}i}|01, j, k), \quad (98)$$

where the set $\Omega = \{\text{b1}, \text{b2}, \text{b3}\}$ indicates the type of block considered, $p_{(j,k|01)}$ is the conditional probability that the signals emitted by Alice occupy the $k$th position in a block of signals of the type $j \in \Omega$ given that she sent the signals $|\varphi_0\rangle \otimes |\varphi_1\rangle$, and $p_{\text{click}}(\text{D}_{\text{M}i}|01, j, k)$ is the conditional probability that detector $\text{D}_{\text{M}i}$ clicks given that Alice emitted $|\varphi_0\rangle \otimes |\varphi_1\rangle$ and these signals occupy the $k$th position in a block of signals of the type $j \in \Omega$.

### 1. *Blocks of the type "b1"*

Let us first consider blocks of the type "b1", *i.e.*, those blocks which are directly of the form "01" without performing any processing on them. We will consider the different positions (see Fig. 11) in which the signals $|\varphi_0\rangle \otimes |\varphi_1\rangle$ can be located with respect to the block.

*Positions 1 and 5:* In particular, if these signals are located in position 1, this means that Eve has replaced the signal $|\varphi_0\rangle$ with a signal $|\varphi_1\rangle$ and, in addition, she has replaced the signal $|\varphi_1\rangle$ with a vacuum signal. This is illustrated in Fig. 12(a). That is, this implies that at the time instance corresponding to the interference between the signals $|\varphi_0\rangle$ and $|\varphi_1\rangle$, actually at Bob's side interfere the signal $|\varphi_1\rangle$ and the vacuum signal $|0\rangle$. Since the signal $|\varphi_1\rangle = |\alpha\rangle\,|0\rangle$, we have that at such time instance the detectors $\text{D}_{\text{M1}}$ and $\text{D}_{\text{M2}}$ observe the interference of two vacuum signals. As a result, we have that

$$p_{\text{click}}(\text{D}_{\text{M}i}|01, \text{b1}, 1) = 0, \quad (99)$$

for $i = 1, 2$.

Similarly, if the signals $|\varphi_0\rangle \otimes |\varphi_1\rangle$ are located in position 5, this means that Eve has replaced the signal $|\varphi_0\rangle$ with a vacuum signal and, in addition, she has replaced

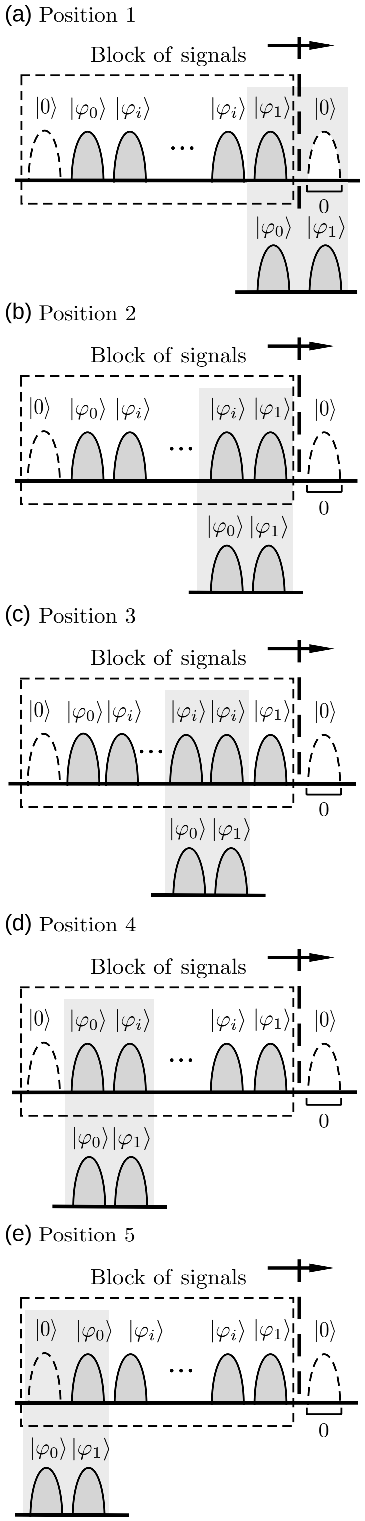


FIG. 12. Illustration of the signals that Eve sends to Bob replacing Alice's signals $|\varphi_0\rangle \otimes |\varphi_1\rangle$. This is shown for the case of blocks of the type "b1" as a function of the position that the signals $|\varphi_0\rangle \otimes |\varphi_1\rangle$ occupy with respect to the block.

the signal $|\varphi_1\rangle$ with a signal $|\varphi_0\rangle$. This is illustrated in Fig. 12(e). That is, this implies that at the time instance corresponding to the interference between $|\varphi_0\rangle$ and $|\varphi_1\rangle$, at Bob's side actually interfere $|0\rangle$ and $|\varphi_0\rangle$. Since the signal $|\varphi_0\rangle = |0\rangle |\alpha\rangle$, we have that at such time instance the detectors $\mathrm{D_{M1}}$ and $\mathrm{D_{M2}}$ observe again the interference of two vacuum signals. That is,

$$p_{\mathrm{click}}(\mathrm{D}_{\mathrm{M}i}|01, \mathrm{b1}, 5) = 0, \tag{100}$$

for $i = 1, 2$.

*Position 2:* Let us now consider the scenario where the signals $|\varphi_0\rangle \otimes |\varphi_1\rangle$ are located in position 2. This implies that the signal $|\varphi_1\rangle$ is correctly identified by Eve and, moreover, the signal $|\varphi_0\rangle$ provides Eve a conclusive result. This is illustrated in Fig. 12(b). To evaluate this case, we rewrite the terms $p_{(\mathrm{b1},2|01)} p_{\mathrm{click}}(\mathrm{D}_{\mathrm{M}i}|01, \mathrm{b1}, 2)$ in Eq. (98) as follows

$$p_{(\mathrm{b1},2|01)} p_{\mathrm{click}}(\mathrm{D}_{\mathrm{M}i}|01, \mathrm{b1}, 2) = \sum_{l=M_{\mathrm{min}}+1}^{M_{\mathrm{max}}+1} p_{(\mathrm{b1},2,l|01)} \times p_{\mathrm{click}}(\mathrm{D}_{\mathrm{M}i}|01, \mathrm{b1}, 2, l), \tag{101}$$

where we have included an additional condition related to the length, $l$, of the block of signals generated by Eve. That is, $p_{(\mathrm{b1},2,l|01)}$ denotes the conditional probability that the signals emitted by Alice occupy the position 2 in a block of signals of the type "b1" and of length $l$ given that she sent Bob the signals $|\varphi_0\rangle \otimes |\varphi_1\rangle$, and $p_{\mathrm{click}}(\mathrm{D}_{\mathrm{M}i}|01, \mathrm{b1}, 2, l)$ is defined analogously.

Now, suppose that $l = M_{\mathrm{min}}+1$ with $M_{\mathrm{min}} = 2$. In this scenario, the probability $p_{(\mathrm{b1},2,M_{\mathrm{min}}+1|01)}$ means that: in the time instance corresponding to the signal sent before $|\varphi_1\rangle$ (which is indicated in Fig. 12 as time instance "0") Eve sends Bob a vacuum state (which happens with probability $p_{|0\rangle}$ given by Eq. (69)), Eve successfully identifies both signals $|\varphi_0\rangle$ and $|\varphi_1\rangle$ emitted by Alice (which happens with probability $q_{\mathrm{s}}^2$, see Table I), Eve obtains an inconclusive result in the following signal (which happens with probability $1 - p_{\mathrm{c}}$), and, moreover, Eve decides to send a block containing non-vacuum signals (which happens with probability $q$ when $l = M_{\mathrm{min}} + 1$). That is, we find that

$$p_{(\mathrm{b1},2,M_{\mathrm{min}}+1|01)} = p_{|0\rangle} q_{\mathrm{s}}^2 (1 - p_{\mathrm{c}}) q. \tag{102}$$

if $M_{\mathrm{min}} = 2$. This means that at the time instance corresponding to the interference between the signals $|\varphi_0\rangle = |0\rangle |\alpha\rangle$ and $|\varphi_1\rangle = |\alpha\rangle |0\rangle$, Bob observes the interference of two coherent states $|\alpha\rangle$. Therefore, we have that

$$\begin{aligned} p_{\mathrm{click}}(\mathrm{D_{M1}}|01, \mathrm{b1}, 2, M_{\mathrm{min}} + 1) &= \lambda, \\ p_{\mathrm{click}}(\mathrm{D_{M2}}|01, \mathrm{b1}, 2, M_{\mathrm{min}} + 1) &= 0 \end{aligned} \tag{103}$$

with the parameter $\lambda$ given by Eq. (94).

On the other hand, if $M_{\mathrm{min}} > 2$, we have that the probability $p_{(\mathrm{b1},2,M_{\mathrm{min}}+1|01)}$ implies that: in the time instance

"0" Eve sends Bob a vacuum state (which happens again with probability $p_{|0\rangle}$), Eve successfully identifies the signal $|\varphi_1\rangle$ emitted by Alice (which happens with probability $q_{\rm s}$), Eve obtains a conclusive result when she measures the signal $|\varphi_0\rangle$ (which happens with probability $p_{\rm c}$), Eve obtains $M_{\rm min}-3$ further conclusive results when she measures the following $M_{\rm min}-3$ signals (which happens with probability $p_{\rm c}^{M_{\rm min}-3}$), Eve finds the result $|\varphi_0\rangle$ when measuring the next signal (which happens with probability $p_{\rm c}p(0|{\rm c})$, with $p(0|{\rm c})$ given by Eq. (23)), Eve obtains an inconclusive result in the following signal (which happens with probability $1-p_{\rm c}$), and, moreover, Eve decides to send a block containing non-vacuum signals (which happens with probability $q$ when $l=M_{\rm min}+1$). That is, we find that

$$p_{({\rm b1},2,M_{\rm min}+1|01)}=p_{|0\rangle}q_{\rm s}p_{\rm c}^{M_{\rm min}-1}p(0|{\rm c})(1-p_{\rm c})q, \quad (104)$$

if $M_{\rm min}>2$.

To calculate $p_{\rm click}({\rm D_{M\mathit{i}}}|01,{\rm b1},2,M_{\rm min}+1)$, we need to take into account the signal that Eve sends to Bob instead of the original $|\varphi_0\rangle$ emitted by Alice. In particular, let $r_{(i|0)}$ denote the conditional probability that Eve sends Bob the signal $|\varphi_i\rangle$ instead of the signal $|\varphi_0\rangle$. These probabilities are given by

$$r_{(0|0)}=\frac{q_{\rm s}}{p_{\rm c}}, \qquad r_{(1|0)}=\frac{q_{\rm f}}{p_{\rm c}}, \qquad r_{(2|0)}=r_{(1|0)}, \quad (105)$$

where $q_{\rm f}$ is given in Table I. To be precise, if Eve sends Bob say $|\varphi_0\rangle$ (or the signal $|\varphi_d\rangle=|\alpha\rangle|\alpha\rangle$) after $|\varphi_1\rangle$, we have that in the time instance corresponding to the interference between the original signals, $|\varphi_0\rangle$ and $|\varphi_1\rangle$, Bob observes the interference between two coherent states $|\alpha\rangle$. Therefore, $p_{\rm click}({\rm D_{M\mathit{i}}}|01,{\rm b1},2,M_{\rm min}+1)$ is given by Eq. (103). But, if Eve sends Bob say a signal $|\varphi_1\rangle$ after $|\varphi_1\rangle$, then Bob observes instead the interference between a vacuum signal and a coherent state. Therefore, in this last case, we have that $p_{\rm click}({\rm D_{M1}}|01,{\rm b1},2,M_{\rm min}+1)=p_{\rm click}({\rm D_{M2}}|01,{\rm b1},2,M_{\rm min}+1)=\gamma$, with the parameter $\gamma$ given by Eq. (94). That is, we find that

$$\begin{aligned}p_{\rm click}({\rm D_{M1}}|01,{\rm b1},2,M_{\rm min}+1)&=\frac{q_{\rm s}+q_{\rm f}}{p_{\rm c}}\lambda+\frac{q_{\rm f}}{p_{\rm c}}\gamma,\\ p_{\rm click}({\rm D_{M2}}|01,{\rm b1},2,M_{\rm min}+1)&=\frac{q_{\rm f}}{p_{\rm c}}\gamma. \quad (106)\end{aligned}$$

This means, that, in general, we find that

$$p_{({\rm b1},2,M_{\rm min}+1|01)}p_{\rm click}({\rm D_{M1}}|01,{\rm b1},2,M_{\rm min}+1)=\begin{cases}p_{|0\rangle}q_{\rm s}^2(1-p_{\rm c})q\lambda & \text{if } M_{\rm min}=2,\\ p_{|0\rangle}q_{\rm s}p_{\rm c}^{M_{\rm min}-2}p(0|{\rm c})(1-p_{\rm c})q\Theta & \text{if } M_{\rm min}>2,\end{cases} \quad (107)$$

and

$$p_{({\rm b1},2,M_{\rm min}+1|01)}p_{\rm click}({\rm D_{M2}}|01,{\rm b1},2,M_{\rm min}+1)=\begin{cases}0 & \text{if } M_{\rm min}=2,\\ p_{|0\rangle}q_{\rm s}q_{\rm f}p_{\rm c}^{M_{\rm min}-2}p(0|{\rm c})(1-p_{\rm c})q\gamma & \text{if } M_{\rm min}>2,\end{cases} \quad (108)$$

where the parameter $\Theta$ is defined as

$$\Theta=(q_{\rm s}+q_{\rm f})\lambda+q_{\rm f}\gamma. \quad (109)$$

Let us now consider the situation where $M_{\rm min}+1<l<M_{\rm max}+1$. The analysis is similar to above. In particular, the probability $p_{({\rm b1},2,l|01)}$ implies that: in the time instance "0" Eve sends Bob a vacuum state, Eve successfully identifies the signal $|\varphi_1\rangle$ emitted by Alice, Eve obtains a conclusive result when she measures the signal $|\varphi_0\rangle$, Eve obtains $l-4$ further conclusive results when she measures the following $l-4$ signals, Eve finds the result $|\varphi_0\rangle$ when measuring the next signal (which corresponds to the signal located in the position $l-1$ of the block), and Eve obtains an inconclusive result in the following signal (which corresponds to the signal located in the position $l$ of the block). That is, we find that

$$p_{({\rm b1},2,l|01)}=p_{|0\rangle}q_{\rm s}p_{\rm c}^{l-2}p(0|{\rm c})(1-p_{\rm c}). \quad (110)$$

On the other hand, the calculation of the probability $p_{\rm click}({\rm D_{M\mathit{i}}}|01,{\rm b1},2,l)$, with $M_{\rm min}+1<l<M_{\rm max}+1$, is exactly the same like in the case of $p_{\rm click}({\rm D_{M\mathit{i}}}|01,{\rm b1},2,M_{\rm min}+1)$ with $M_{\rm min}>2$, and the results coincide with those given by Eqs. (103)-(106). We find, therefore that

$$\begin{aligned}p_{({\rm b1},2,l|01)}p_{\rm click}({\rm D_{M1}}|01,{\rm b1},2,l)&=p_{|0\rangle}q_{\rm s}p_{\rm c}^{l-3}p(0|{\rm c})\\&\quad\times(1-p_{\rm c})\Theta,\\ p_{({\rm b1},2,l|01)}p_{\rm click}({\rm D_{M2}}|01,{\rm b1},2,l)&=p_{|0\rangle}q_{\rm s}q_{\rm f}p_{\rm c}^{l-3}p(0|{\rm c})\\&\quad\times(1-p_{\rm c})\gamma, \quad (111)\end{aligned}$$

if $M_{\rm min}+1<l<M_{\rm max}+1$.

Finally, let us now consider the case $l=M_{\rm max}+1$. This situation is exactly the same as that of $M_{\rm min}+1<l<M_{\rm max}+1$ except for one point: now it is not necessary that Eve obtains an inconclusive result in the signal located in the last position of the block, *i.e.*, in the position $M_{\rm max}+1$. This is so because if Eve obtains

$M_{\max}$ consecutive conclusive results, she sends the block to Bob independently of her measurement result in the position $M_{\max}+1$ of the block, where she will send Bob a vacuum signal anyway. This means that

$$
\begin{aligned}
p_{(\mathrm{b1},2,M_{\max}+1|01)}p_{\mathrm{click}}(\mathrm{D_{M1}}|01,\mathrm{b1},2,M_{\max}+1) &= p_{|0\rangle}q_{\mathrm{s}}p_{\mathrm{c}}^{M_{\max}-2}p(0|\mathrm{c})\Theta,\\
p_{(\mathrm{b1},2,M_{\max}+1|01)}p_{\mathrm{click}}(\mathrm{D_{M2}}|01,\mathrm{b1},2,M_{\max}+1) &= p_{|0\rangle}q_{\mathrm{s}}q_{\mathrm{f}}p_{\mathrm{c}}^{M_{\max}-2}p(0|\mathrm{c})\gamma,
\end{aligned}
\tag{112}
$$

By combining Eqs. (101)-(107)-(108)-(111)-(112) we obtain

$$
\begin{aligned}
p_{(\mathrm{b1},2|01)}p_{\mathrm{click}}(\mathrm{D_{M1}}|01,\mathrm{b1},2) &= \begin{cases} p_{|0\rangle}q_{\mathrm{s}}\Big\{q_{\mathrm{s}}(1-p_{\mathrm{c}})q\lambda+p(0|\mathrm{c})p_{\mathrm{c}}\Theta\Big\} & \text{if } M_{\min}=2,\\ p_{|0\rangle}q_{\mathrm{s}}p(0|\mathrm{c})p_{\mathrm{c}}^{M_{\min}-2}\big[p_{\mathrm{c}}+(1-p_{\mathrm{c}})q\big]\Theta & \text{if } M_{\min}>2,\end{cases}\\
p_{(\mathrm{b1},2|01)}p_{\mathrm{click}}(\mathrm{D_{M2}}|01,\mathrm{b1},2) &= \begin{cases} p_{|0\rangle}q_{\mathrm{s}}q_{\mathrm{f}}p(0|\mathrm{c})\gamma p_{\mathrm{c}} & \text{if } M_{\min}=2,\\ p_{|0\rangle}q_{\mathrm{s}}q_{\mathrm{f}}p(0|\mathrm{c})\gamma p_{\mathrm{c}}^{M_{\min}-2}\big[p_{\mathrm{c}}+(1-p_{\mathrm{c}})q\big] & \text{if } M_{\min}>2.\end{cases}
\end{aligned}
\tag{113}
$$

*Position 3:* We now evaluate the case where the signals $|\varphi_0\rangle\otimes|\varphi_1\rangle$ are located in position 3 (see Fig. 12(c)). Similar to Eq. (101), we rewrite the terms $p_{(\mathrm{b1},3|01)}p_{\mathrm{click}}(\mathrm{D_{M}}_i|01,\mathrm{b1},3)$ in Eq. (98) as follows

$$
p_{(\mathrm{b1},3|01)}p_{\mathrm{click}}(\mathrm{D_{M}}_i|01,\mathrm{b1},3) = \sum_{l=M_{\min}+1}^{M_{\max}+1} p_{(\mathrm{b1},3,l|01)} \times p_{\mathrm{click}}(\mathrm{D_{M}}_i|01,\mathrm{b1},3,l),
\tag{114}
$$

where we include the condition related to the length, $l$, of the block of signals generated by Eve.

The pair of signals $|\varphi_0\rangle\otimes|\varphi_1\rangle$ can only occupy the position 3 of a block of signals if $l\geq 5$. This is illustrated in Fig. 13. Let us consider first the case $l=M_{\min}+1$ with $M_{\min}\geq 4$. There are $l-4$ different alternatives in which the signals $|\varphi_0\rangle\otimes|\varphi_1\rangle$ can occupy position 3 (see Fig. 13). In all of them, the probability $p_{(\mathrm{b1},3,M_{\min}+1|01)}$ means that: in the time instance "0" Eve sends Bob a vacuum state (which happens with probability $p_{|0\rangle}$), Eve's measurement result corresponding to the next signal is $|\varphi_1\rangle$ (which happens with probability $p_{\mathrm{c}}p(1|\mathrm{c})$), Eve obtains $M_{\min}-2$ consecutive conclusive measurement results when measuring the next $M_{\min}-2$ signals, Eve's measurement result corresponding to the next signal is $|\varphi_0\rangle$ (which happens with probability $p_{\mathrm{c}}p(0|\mathrm{c})$), Eve obtains an inconclusive result in the following signal (which happens with probability $1-p_{\mathrm{c}}$), and, moreover, Eve decides to send a block containing non-vacuum signals (which happens with probability $q$ when $l=M_{\min}+1$). That is, we find that

$$
p_{(\mathrm{b1},3,M_{\min}+1|01)} = (M_{\min}-3)p_{|0\rangle}p(0|\mathrm{c})p(1|\mathrm{c})(1-p_{\mathrm{c}}) \times p_{\mathrm{c}}^{M_{\min}}q,
\tag{115}
$$

if $M_{\min}\geq 4$.

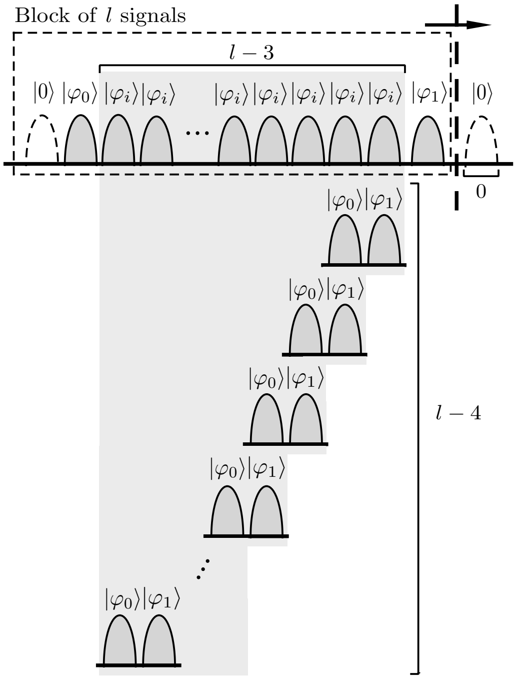


FIG. 13. Illustration of the $l-4$ possible ways in which the pair of signals $|\varphi_0\rangle\otimes|\varphi_1\rangle$ prepared by Alice can occupy the position 3 of a block of the type "b1" (with non-vacuum signals) generated by Eve.

To calculate $p_{\mathrm{click}}(\mathrm{D_{M}}_i|01,\mathrm{b1},3,M_{\min}+1)$, we need to consider the signals that Eve sends to Bob instead of the original $|\varphi_0\rangle$ and $|\varphi_1\rangle$ emitted by Alice. In particular, let $r_{(i|1)}$ denote the conditional probability that Eve sends Bob the signal $|\varphi_i\rangle$ instead of the signal $|\varphi_1\rangle$ prepared by Alice (note that the probabilities $r_{(i|0)}$ have been already

defined in Eq. (105)). These probabilities are given by

$$r_{(0|1)} = \frac{q_{\rm f}}{p_{\rm c}}, \qquad r_{(1|1)} = \frac{q_{\rm s}}{p_{\rm c}}, \qquad r_{(2|1)} = r_{(0|1)}, \quad (116)$$

There are in total nine possible combinations of signals that Eve can send to Bob, each of them happening with probability $r_{(i|0)}r_{(j|1)}$ with $i,j \in \{0,1,2\}$. For instance, with probability $r_{(0|0)}r_{(0|1)} = q_{\rm s}q_{\rm f}/p_{\rm c}^2$ Eve sends Bob the signals $|\varphi_0\rangle \otimes |\varphi_0\rangle$ (instead of the signals $|\varphi_0\rangle \otimes |\varphi_1\rangle$). This means that in the time instance corresponding to the interference between the original signals, Bob actually observes the interference between a coherent state $|\alpha\rangle$ (from the signal $|\varphi_0\rangle$) and a vacuum signal (from the other signal $|\varphi_0\rangle$). Therefore, we have that in this case both detectors $\rm D_{M1}$ and $\rm D_{M2}$ click with probability $\gamma$. Similarly, with probability $r_{(0|0)}r_{(2|1)} = q_{\rm s}q_{\rm f}/p_{\rm c}^2$ Eve sends Bob the signals $|\varphi_0\rangle \otimes |\varphi_2\rangle$ (instead of the signals $|\varphi_0\rangle \otimes |\varphi_1\rangle$). That is, in the time instance corresponding to the interference between the original signals, Bob observes the interference between two coherent states $|\alpha\rangle$. Therefore, we have that in this case detector $\rm D_{M1}$ clicks with probability $\lambda$ and detector $\rm D_{M2}$ never clicks. The remaining cases are similar and we omit them here for simplicity. We obtain

$$\begin{aligned} p_{\rm click}({\rm D_{M1}}|01,{\rm b1},3,M_{\rm min}+1) &= \frac{(q_{\rm s}+q_{\rm f})^2}{p_{\rm c}^2}\lambda \\ &\quad + \frac{2q_{\rm f}(q_{\rm s}+q_{\rm f})}{p_{\rm c}^2}\gamma, \\ p_{\rm click}({\rm D_{M2}}|01,{\rm b1},3,M_{\rm min}+1) &= \frac{2q_{\rm f}(q_{\rm s}+q_{\rm f})}{p_{\rm c}^2}\gamma. \quad (117) \end{aligned}$$

This means, that, in general, we find that

$$\begin{aligned} p_{({\rm b1},3,M_{\rm min}+1|01)}p_{\rm click}({\rm D_{M1}}|01,{\rm b1},3,M_{\rm min}+1) &= (M_{\rm min}-3)p_{|0\rangle}p(0|{\rm c})p(1|{\rm c})(1-p_{\rm c})p_{\rm c}^{M_{\rm min}-2}q\xi \\ p_{({\rm b1},3,M_{\rm min}+1|01)}p_{\rm click}({\rm D_{M2}}|01,{\rm b1},3,M_{\rm min}+1) &= 2(M_{\rm min}-3)p_{|0\rangle}p(0|{\rm c})p(1|{\rm c})(1-p_{\rm c})p_{\rm c}^{M_{\rm min}-2}qq_{\rm f}(q_{\rm s}+q_{\rm f})\gamma, \quad (118) \end{aligned}$$

if $M_{\rm min} \geq 4$, and zero otherwise, where the parameter $\xi$ is defined as

$$\xi = (q_{\rm s}+q_{\rm f})^2\lambda + 2q_{\rm f}(q_{\rm s}+q_{\rm f})\gamma. \quad (119)$$

The scenario $M_{\rm min}+1 < l < M_{\rm max}+1$ is analogous to the case $l = M_{\rm min}+1$. The only difference is that now Eve always sends the block to Bob (instead of sending it with probability $q$). We have, therefore, that

$$p_{({\rm b1},3,l|01)} = (l-4)p_{|0\rangle}p(0|{\rm c})p(1|{\rm c})(1-p_{\rm c})p_{\rm c}^{l-1}, \quad (120)$$

if $l > \max[M_{\rm min}+1,4]$. On the other hand, the expression for the probabilities $p_{\rm click}({\rm D_{M1}}|01,{\rm b1},3,M_{\rm min}+1)$ and $p_{\rm click}({\rm D_{M2}}|01,{\rm b1},3,M_{\rm min}+1)$ coincides with that given in Eq. (117). Putting all together, we obtain

$$\begin{aligned} p_{({\rm b1},3,l|01)}p_{\rm click}({\rm D_{M1}}|01,{\rm b1},3,l) &= (l-4)p_{|0\rangle}p(0|{\rm c})p(1|{\rm c})(1-p_{\rm c})p_{\rm c}^{l-3}\xi, \\ p_{({\rm b1},3,l|01)}p_{\rm click}({\rm D_{M2}}|01,{\rm b1},3,l) &= 2(l-4)p_{|0\rangle}p(0|{\rm c})p(1|{\rm c})(1-p_{\rm c})p_{\rm c}^{l-3}q_{\rm f}(q_{\rm s}+q_{\rm f})\gamma, \quad (121) \end{aligned}$$

if $l > \max[M_{\rm min}+1,4]$, and zero otherwise.

Finally, we consider the case $l = M_{\rm max}+1$. Again, the only difference with respect to the previous case (where $M_{\rm min}+1 < l < M_{\rm max}+1$) is that here it is not necessary that Eve observes an inconclusive result in the signal located in the last position of the block. Then, by removing the multiplicative term $1-p_{\rm c}$ from the expressions in Eq. (121) and by imposing $l = M_{\rm max}+1$, we obtain

$$\begin{aligned} p_{({\rm b1},3,M_{\rm max}+1|01)}p_{\rm click}({\rm D_{M1}}|01,{\rm b1},3,M_{\rm max}+1) &= (M_{\rm max}-3)p_{|0\rangle}p(0|{\rm c})p(1|{\rm c})p_{\rm c}^{M_{\rm max}-2}\xi, \\ p_{({\rm b1},3,M_{\rm max}+1|01)}p_{\rm click}({\rm D_{M2}}|01,{\rm b1},3,M_{\rm max}+1) &= 2(M_{\rm max}-3)p_{|0\rangle}p(0|{\rm c})p(1|{\rm c})p_{\rm c}^{M_{\rm max}-2}q_{\rm f}(q_{\rm s}+q_{\rm f})\gamma, \quad (122) \end{aligned}$$

if $M_{\rm max} \geq 4$.

By combining Eqs. (114)-(118)-(121)-(122) we find that

$$p_{(\mathrm{b1},3|01)}p_{\mathrm{click}}(\mathrm{D_{M1}}|01,\mathrm{b1},3)=\begin{cases}p_{|0\rangle}p(0|\mathrm{c})p(1|\mathrm{c})\xi\frac{p_{\mathrm{c}}^{2}(1-p_{\mathrm{c}}^{M_{\max}-3})}{1-p_{\mathrm{c}}} & \text{if } M_{\min}<4 \text{ and } M_{\max}\geq 4,\\ p_{|0\rangle}p(0|\mathrm{c})p(1|\mathrm{c})p_{\mathrm{c}}^{M_{\min}-2}\xi\sigma & \text{if } M_{\min}\geq 4 \text{ and } M_{\max}\geq M_{\min}+1,\end{cases}$$

$$p_{(\mathrm{b1},3|01)}p_{\mathrm{click}}(\mathrm{D_{M2}}|01,\mathrm{b1},3)=\begin{cases}2p_{|0\rangle}p(0|\mathrm{c})p(1|\mathrm{c})q_{\mathrm{f}}(q_{\mathrm{s}}+q_{\mathrm{f}})\gamma\frac{p_{\mathrm{c}}^{2}(1-p_{\mathrm{c}}^{M_{\max}-3})}{1-p_{\mathrm{c}}} & \text{if } M_{\min}<4 \text{ and } M_{\max}\geq 4,\\ 2p_{|0\rangle}p(0|\mathrm{c})p(1|\mathrm{c})p_{\mathrm{c}}^{M_{\min}-2}q_{\mathrm{f}}(q_{\mathrm{s}}+q_{\mathrm{f}})\gamma\sigma & \text{if } M_{\min}\geq 4 \text{ and } M_{\max}\geq M_{\min}+1,\end{cases} \tag{123}$$

where the parameter $\sigma$ is given by

$$\sigma=(M_{\min}-3)(1-p_{\mathrm{c}})q+\frac{p_{\mathrm{c}}}{1-p_{\mathrm{c}}}\big[(3p_{\mathrm{c}}+M_{\min}(1-p_{\mathrm{c}})-2)-p_{\mathrm{c}}^{M_{\max}-M_{\min}}\big]. \tag{124}$$

*Position 4:* To conclude this part, we now evaluate the scenario where the signals $|\varphi_0\rangle\otimes|\varphi_1\rangle$ are located in position 4. This case is very similar to that where the signals occupy the position 2. In particular, here we have that the signal $|\varphi_0\rangle$ is correctly identified by Eve and, in addition, the signal $|\varphi_1\rangle$ provides Eve a conclusive result (see Fig. 12(d)). Like in the previous two cases, we rewrite the terms $p_{(\mathrm{b1},4|01)}p_{\mathrm{click}}(\mathrm{D}_{\mathrm{M}i}|01,\mathrm{b1},4)$ in Eq. (98) as follows

$$p_{(\mathrm{b1},4|01)}p_{\mathrm{click}}(\mathrm{D}_{\mathrm{M}i}|01,\mathrm{b1},4)=\sum_{l=M_{\min}+1}^{M_{\max}+1}p_{(\mathrm{b1},4,l|01)}\times p_{\mathrm{click}}(\mathrm{D}_{\mathrm{M}i}|01,\mathrm{b1},4,l), \tag{125}$$

by conditioning on the length, $l$, of the block of signals generated by Eve.

If $l=M_{\min}+1$ with $M_{\min}=2$, this case coincides precisely with that evaluated when considering the position 2. So, to avoid counting this event twice, we set

$$p_{(\mathrm{b1},4,M_{\min}+1|01)}=0, \tag{126}$$

if $M_{\min}=2$. On the other hand, if $M_{\min}>2$, the probability $p_{(\mathrm{b1},4,M_{\min}+1|01)}$ implies that: in the time instance "0" Eve sends Bob a vacuum state, in the next time instance Eve's measurement result is $|\varphi_1\rangle$, then Eve obtains $M_{\min}-3$ further conclusive results when she measures the following $M_{\min}-3$ signals, Eve obtains a conclusive result when she measures the signal $|\varphi_1\rangle$, Eve successfully identifies the signal $|\varphi_0\rangle$ emitted by Alice, Eve obtains an inconclusive result in the following signal, and, moreover, Eve decides to send a block of signals containing non-vacuum signals. That is, we find that

$$p_{(\mathrm{b1},4,M_{\min}+1|01)}=p_{|0\rangle}q_{\mathrm{s}}p_{\mathrm{c}}^{M_{\min}-1}p(1|\mathrm{c})(1-p_{\mathrm{c}})q, \tag{127}$$

if $M_{\min}>2$.

To determine $p_{\mathrm{click}}(\mathrm{D}_{\mathrm{M}i}|01,\mathrm{b1},4,M_{\min}+1)$, we take into account the probability $r(i|1)$, given by Eq. (116), that Eve sends Bob the signal $|\varphi_i\rangle$ instead of the original $|\varphi_1\rangle$ emitted by Alice. In particular, if Eve sends Bob say $|\varphi_1\rangle$ (or the signal $|\varphi_d\rangle$) before $|\varphi_0\rangle$, then in the time instance corresponding to the interference between the original signals, $|\varphi_0\rangle$ and $|\varphi_1\rangle$, Bob observes the interference between two coherent states, and thus $p_{\mathrm{click}}(\mathrm{D_{M1}}|01,\mathrm{b1},4,M_{\min}+1)=\lambda$ and $p_{\mathrm{click}}(\mathrm{D_{M2}}|01,\mathrm{b1},4,M_{\min}+1)=0$. But if Eve sends Bob $|\varphi_0\rangle$ before $|\varphi_0\rangle$, then in the time instance corresponding to the interference between the two signals, Bob observes the interference between a coherent state and a vacuum state, and thus $p_{\mathrm{click}}(\mathrm{D_{M1}}|01,\mathrm{b1},4,M_{\min}+1)=p_{\mathrm{click}}(\mathrm{D_{M2}}|01,\mathrm{b1},4,M_{\min}+1)=\gamma$. That is, we have that $p_{\mathrm{click}}(\mathrm{D}_{\mathrm{M}i}|01,\mathrm{b1},4,M_{\min}+1)=p_{\mathrm{click}}(\mathrm{D}_{\mathrm{M}i}|01,\mathrm{b1},2,M_{\min}+1)$, with $i=1,2$, and $p_{\mathrm{click}}(\mathrm{D}_{\mathrm{M}i}|01,\mathrm{b1},2,M_{\min}+1)$ given by Eqs. (103)-(106).

This means, that, in general, we obtain that

$$p_{(\mathrm{b1},4,M_{\min}+1|01)}p_{\mathrm{click}}(\mathrm{D_{M1}}|01,\mathrm{b1},4,M_{\min}+1)=\begin{cases}0 & \text{if } M_{\min}=2,\\ p_{|0\rangle}q_{\mathrm{s}}p_{\mathrm{c}}^{M_{\min}-2}p(1|\mathrm{c})(1-p_{\mathrm{c}})q\Theta & \text{if } M_{\min}>2,\end{cases} \tag{128}$$

$$p_{(\mathrm{b1},4,M_{\min}+1|01)}p_{\mathrm{click}}(\mathrm{D_{M2}}|01,\mathrm{b1},4,M_{\min}+1)=\begin{cases}0 & \text{if } M_{\min}=2,\\ p_{|0\rangle}q_{\mathrm{s}}q_{\mathrm{f}}p_{\mathrm{c}}^{M_{\min}-2}p(1|\mathrm{c})(1-p_{\mathrm{c}})q\gamma & \text{if } M_{\min}>2,\end{cases} \tag{129}$$

where the parameter $\Theta$ is given by Eq. (109).

Next we consider the situation where $M_{\min}+1<l<M_{\max}+1$. It is easy to show that in this case the probability $p_{(\mathrm{b1},4,l|01)}$ is given by

$$p_{(\mathrm{b1},4,l|01)}=p_{|0\rangle}q_{\mathrm{s}}p_{\mathrm{c}}^{l-2}p(1|\mathrm{c})(1-p_{\mathrm{c}}). \tag{130}$$

Similarly, we have that $p_{\mathrm{click}}(\mathrm{D}_{\mathrm{M}i}|01,\mathrm{b1},4,l)=$

$p_{\rm click}({\rm D}_{{\rm M}i}|01,{\rm b1},4,M_{\rm min}+1)$ with $M_{\rm min}>2$, and thus we have

$$p_{({\rm b1},4,l|01)}p_{\rm click}({\rm D}_{\rm M1}|01,{\rm b1},4,l) = p_{|0\rangle}q_{\rm s}p_{\rm c}^{l-3}p(1|{\rm c}) \times (1-p_{\rm c})\Theta,$$
$$p_{({\rm b1},4,l|01)}p_{\rm click}({\rm D}_{\rm M2}|01,{\rm b1},4,l) = p_{|0\rangle}q_{\rm s}q_{\rm f}p_{\rm c}^{l-3}p(1|{\rm c}) \times (1-p_{\rm c})\gamma. \quad (131)$$

Finally, we evaluate the scenario $l=M_{\rm max}+1$. Again, the situation is equal to that of $M_{\rm min}+1<l<M_{\rm max}+1$ except that now it is not necessary that Eve obtains an inconclusive result in the signal located in the last position of the block. This means that

$$p_{({\rm b1},4,M_{\rm max}+1|01)}p_{\rm click}({\rm D}_{\rm M1}|01,{\rm b1},4,M_{\rm max}+1) = p_{|0\rangle}q_{\rm s}p_{\rm c}^{M_{\rm max}-2}p(1|{\rm c})\Theta,$$
$$p_{({\rm b1},4,M_{\rm max}+1|01)}p_{\rm click}({\rm D}_{\rm M2}|01,{\rm b1},4,M_{\rm max}+1) = p_{|0\rangle}q_{\rm s}q_{\rm f}p_{\rm c}^{M_{\rm max}-2}p(1|{\rm c})\gamma. \quad (132)$$

By combining Eqs. (125)-(128)-(129)-(131)-(132) we obtain

$$p_{({\rm b1},4|01)}p_{\rm click}({\rm D}_{\rm M1}|01,{\rm b1},4) = \begin{cases} p_{|0\rangle}q_{\rm s}p(1|{\rm c})p_{\rm c}\Theta & \text{if } M_{\rm min}=2,\\ p_{|0\rangle}q_{\rm s}p(1|{\rm c})p_{\rm c}^{M_{\rm min}-2}\left[p_{\rm c}+(1-p_{\rm c})q\right]\Theta & \text{if } M_{\rm min}>2,\end{cases}$$
$$p_{({\rm b1},4|01)}p_{\rm click}({\rm D}_{\rm M2}|01,{\rm b1},4) = \begin{cases} p_{|0\rangle}q_{\rm s}q_{\rm f}p(1|{\rm c})\gamma p_{\rm c} & \text{if } M_{\rm min}=2,\\ p_{|0\rangle}q_{\rm s}q_{\rm f}p(1|{\rm c})\gamma p_{\rm c}^{M_{\rm min}-2}\left[p_{\rm c}+(1-p_{\rm c})q\right] & \text{if } M_{\rm min}>2,\end{cases} \quad (133)$$

Note that these probabilities coincide with the probabilities $p_{({\rm b1},2|01)}p_{\rm click}({\rm D}_{{\rm M}i}|01,{\rm b1},2)$ given by Eq. (113), except from the fact that in Eq. (113) appears $p(0|{\rm c})$ (instead of $p(1|{\rm c})$) and, in addition, Eq. (113) includes the contribution of a block of length $l=M_{\rm min}+1$ when $M_{\rm min}=2$, while Eq. (133) does not include such term; otherwise we would count such event twice.

### 2. *Blocks of the type "b2"*

Next we consider blocks of the type "b2", *i.e.*, those blocks which are not of the form "01" but Eve sends them to Bob anyway with probability $1-q_{\rm p}$.

The first signal (last non-vacuum signal, *i.e.*, the signal which occupies the position $l-1$) of the block can be $|\varphi_m\rangle$, with $m=0,1,2$, ($|\varphi_n\rangle$, with $n=0,1,2$), expect for the combination $m=1$ and $n=0$, since this case corresponds to a block of the type "b1". For simplicity, we shall consider each of the eight possible combinations $(m,n)$ for the first and last non-vacuum signal of the block individually. That is, we write

$$\sum_{k=1}^{5} p_{({\rm b2},k|01)}p_{\rm click}({\rm D}_{{\rm M}i}|01,{\rm b2},k) = \sum_{\substack{m,n=0\\(m,n)\neq(1,0)}}^{2}\sum_{k=1}^{5} p^{(m,n)}_{({\rm b2},k|01)}p^{(m,n)}_{\rm click}({\rm D}_{{\rm M}i}|01,{\rm b2},k), \quad (134)$$

where $p^{(m,n)}_{({\rm b2},k|01)}$ and $p^{(m,n)}_{\rm click}({\rm D}_{{\rm M}i}|01,{\rm b2},k)$ refer to the probabilities $p_{({\rm b2},k|01)}$ and $p_{\rm click}({\rm D}_{{\rm M}i}|01,{\rm b2},k)$ when the first (last non-vacuum) signal of the block is $|\varphi_m\rangle$ ($|\varphi_n\rangle$).

In addition, like above, for each position $k=1,\ldots,5$ (see Fig. 11), in which the original signals, $|\varphi_0\rangle\otimes|\varphi_1\rangle$, prepared by Alice can be located with respect to the block, we will write

$$p^{(m,n)}_{({\rm b2},k|01)}p^{(m,n)}_{\rm click}({\rm D}_{{\rm M}i}|01,{\rm b2},k) = \sum_{l=M_{\rm min}+1}^{M_{\rm max}+1} p^{(m,n)}_{({\rm b2},k,l|01)} \times p^{(m,n)}_{\rm click}({\rm D}_{{\rm M}i}|01,{\rm b2},k,l), \quad (135)$$

where $l$ indicates again the length of the block.

As an illustration, below we focus on the case $m=n=0$. That is, this is a block whose first and last non-vacuum signals are both in the state $|\varphi_0\rangle$.

*Position 1:* Let us begin with the case $l = M_{\min}+1$. The probability $p^{(0,0)}_{(\mathrm{b}2,1,M_{\min}+1|01)}$ implies that: in the time instance "0" (corresponding to the signal $|\varphi_1\rangle$) Eve sends Bob a vacuum state (which happens with probability $p_{|0\rangle}$), in the next signal Eve successfully identifies $|\varphi_0\rangle$ (which happens with probability $q_{\mathrm{s}}$), then Eve obtains $M_{\min}-2$ consecutive conclusive results in the following $M_{\min}-2$ signals (which happens with probability $p_{\mathrm{c}}^{M_{\min}-2}$), Eve finds the result $|\varphi_0\rangle$ in the signal located in the position $M_{\min}$ of the block (which happens with probability $p_c p(0|\mathrm{c})$), Eve obtains an inconclusive result in the following signal (which happens with probability $1-p_{\mathrm{c}}$), Eve decides to check if the block is of the type "01" (which happens with probability $q$ when $l = M_{\min}+1$), and, moreover, Eve decides to send a block containing non-vacuum signals to Bob even if the block is not of the type '01" (which happens with probability $1-q_{\mathrm{p}}$). That is, we obtain

$$p^{(0,0)}_{(\mathrm{b}2,1,M_{\min}+1|01)} = p_{|0\rangle} q_{\mathrm{s}} p_{\mathrm{c}}^{M_{\min}-1} p(0|\mathrm{c})(1-p_{\mathrm{c}})q(1-q_{\mathrm{p}}). \tag{136}$$

To calculate $p^{(0,0)}_{\mathrm{click}}(\mathrm{D}_{\mathrm{M}i}|01,\mathrm{b}2,1,M_{\min}+1)$, note that in the time instance corresponding to the interference between the original signals, $|\varphi_0\rangle$ and $|\varphi_1\rangle$, Bob observes the interference between a coherent state $|\alpha\rangle$ (from $|\varphi_0\rangle$) and a vacuum signal (as $|\varphi_1\rangle$ is replaced by Eve with vacuum). This means that

$$p^{(0,0)}_{\mathrm{click}}(\mathrm{D}_{\mathrm{M}i}|01,\mathrm{b}2,1,M_{\min}+1) = \gamma, \tag{137}$$

with $\gamma$ given by Eq. (94)

That is, we obtain

$$p^{(0,0)}_{(\mathrm{b}2,1,M_{\min}+1|01)} p^{(0,0)}_{\mathrm{click}}(\mathrm{D}_{\mathrm{M}i}|01,\mathrm{b}2,1,M_{\min}+1) = p_{|0\rangle} \times q_{\mathrm{s}} p_{\mathrm{c}}^{M_{\min}-1} p(0|\mathrm{c})(1-p_{\mathrm{c}})q(1-q_{\mathrm{p}})\gamma. \tag{138}$$

Let us now study the case where $M_{\min}+1 < l < M_{\max}+1$. The probability $p^{(0,0)}_{(\mathrm{b}2,1,l|01)}$ now implies that: in the time instance "0" Eve sends Bob a vacuum state, in the next signal Eve successfully identifies $|\varphi_0\rangle$, then Eve obtains $l-3$ consecutive conclusive results in the following $l-3$ signals, Eve finds the result $|\varphi_0\rangle$ in the signal located in the position $l-1$ of the block, Eve obtains an inconclusive result in the following signal, and, in addition, Eve decides to send a block containing non-vacuum signals to Bob even if the block is not of the type '01". We find, therefore, that

$$p^{(0,0)}_{(\mathrm{b}2,1,l|01)} = p_{|0\rangle} q_{\mathrm{s}} p_{\mathrm{c}}^{l-2} p(0|\mathrm{c})(1-p_{\mathrm{c}})(1-q_{\mathrm{p}}). \tag{139}$$

On the other hand, it is straightforward to show that in this scenario $p^{(0,0)}_{\mathrm{click}}(\mathrm{D}_{\mathrm{M}i}|01,\mathrm{b}2,1,l)$ is also given by Eq. (137). That is, we obtain

$$p^{(0,0)}_{(\mathrm{b}2,1,l|01)} p^{(0,0)}_{\mathrm{click}}(\mathrm{D}_{\mathrm{M}i}|01,\mathrm{b}2,1,l) = p_{|0\rangle} q_{\mathrm{s}} p_{\mathrm{c}}^{l-2} p(0|\mathrm{c}) \times(1-p_{\mathrm{c}})(1-q_{\mathrm{p}})\gamma. \tag{140}$$

To conclude this part, we now consider the case $l = M_{\max}+1$. Like above, the only difference with respect to the previous case is that here it is not necessary that Eve obtains an inconclusive result in the signal located in the last position of the block. This means that

$$p^{(0,0)}_{(\mathrm{b}2,1,M_{\max}+1|01)} p^{(0,0)}_{\mathrm{click}}(\mathrm{D}_{\mathrm{M}1}|01,\mathrm{b}2,1,M_{\max}+1) = p_{|0\rangle} \times q_{\mathrm{s}} p_{\mathrm{c}}^{M_{\max}-1} p(0|\mathrm{c})(1-q_{\mathrm{p}})\gamma. \tag{141}$$

By combining Eqs. (158)-(138)-(140)-(141) we obtain

$$p^{(0,0)}_{(\mathrm{b}2,1|01)} p^{(0,0)}_{\mathrm{click}}(\mathrm{D}_{\mathrm{M}i}|01,\mathrm{b}2,1) = p_{|0\rangle} q_{\mathrm{s}} p(0|\mathrm{c})(1-q_{\mathrm{p}}) \times \gamma p_{\mathrm{c}}^{M_{\min}-1}\big[p_{\mathrm{c}} + (1-p_{\mathrm{c}})q\big]. \tag{142}$$

Considering the remaining $(m,n)$ cases and performing the summation in Eq. (134) we have that

$$p_{(\mathrm{b}2,1|01)} p_{\mathrm{click}}(\mathrm{D}_{\mathrm{M}i}|01,\mathrm{b}2,1) = p_{|0\rangle}(1-q_{\mathrm{p}}) \times \gamma p_{\mathrm{c}}^{M_{\min}-1}(q_s+q_f)\big[p_{\mathrm{c}} + (1-p_{\mathrm{c}})q\big], \tag{143}$$

for $i = 1,2$.

*Position 2:* We now consider the case where the signals $|\varphi_0\rangle \otimes |\varphi_1\rangle$ are located in position 2.

Suppose that $l = M_{\min}+1$ with $M_{\min} = 2$. In this scenario, $p^{(0,0)}_{(\mathrm{b}2,2,M_{\min}+1|01)}$ means that: in the time instance "0" (which now corresponds to the signal sent before $|\varphi_1\rangle$) Eve sends Bob a vacuum state, in the next signal Eve obtains the result $|\varphi_0\rangle$ (instead of the signal $|\varphi_0\rangle$ sent by Alice), which happens with probability $q_{\mathrm{f}}$, Eve successfully identifies both the signal $|\varphi_0\rangle$ emitted by Alice, Eve obtains an inconclusive result in the following signal, Eve decides to check if the block is of the type "01", and, moreover, Eve decides to send a block containing non-vacuum signals to Bob even if the block is not of the type "01". That is, we find that

$$p^{(0,0)}_{(\mathrm{b}2,2,M_{\min}+1|01)} = p_{|0\rangle} q_{\mathrm{f}} q_{\mathrm{s}} (1-p_{\mathrm{c}})q(1-q_{\mathrm{p}}). \tag{144}$$

if $M_{\min} = 2$. This means that at the time instance corresponding to the interference between the original signals $|\varphi_0\rangle$ and $|\varphi_1\rangle$ emitted by Alice, Bob observes the interference of a coherent state $|\alpha\rangle$ (from one $|\varphi_0\rangle$ sent by Eve) and a vacuum signal (from the other $|\varphi_0\rangle$ sent by Eve). That is, we have that $p^{(0,0)}_{\mathrm{click}}(\mathrm{D}_{\mathrm{M}i}|01,\mathrm{b}2,2,M_{\min}+1) = \gamma$.

On the other hand, if $M_{\min} > 2$, the probability $p^{(0,0)}_{(\mathrm{b}2,2,M_{\min}+1|01)}$ implies that: in the time instance "0" Eve sends Bob a vacuum signal, in the next signal Eve obtains the result $|\varphi_0\rangle$, Eve obtains a conclusive result when measuring the signal $|\varphi_0\rangle$ emitted by Alice, Eve obtains $M_{\min}-3$ further conclusive results when measuring the next $M_{\min}-3$ signals, Eve finds the result $|\varphi_0\rangle$ in the signal located in the position $M_{\min}$ of the block, Eve obtains an inconclusive result in the following signal, Eve decides to check if the block is of the type

"01", and, moreover, Eve decides to send a block containing non-vacuum signals to Bob even if the block is not of the type "01". We find, therefore, that

$$p^{(0,0)}_{(\mathrm{b}2,2,M_{\min}+1|01)} = p_{|0\rangle} q_{\mathrm{f}} p_{\mathrm{c}}^{M_{\min}-1} p(0|\mathrm{c})(1-p_{\mathrm{c}})q(1-q_{\mathrm{p}}). \tag{145}$$

if $M_{\min} > 2$.

To calculate $p^{(0,0)}_{\mathrm{click}}(\mathrm{D}_{\mathrm{M}i}|01,\mathrm{b}2,2,M_{\min}+1)$, we take into account the signal that Eve sends to Bob instead of the original $|\varphi_0\rangle$ emitted by Alice. If Eve sends Bob the signal $|\varphi_1\rangle$ (which happens with probability $r_{(1|0)}$ given by Eq. (105)) then in the time instance corresponding to the interference between the original signals, $|\varphi_0\rangle$ and $|\varphi_1\rangle$, Bob observes the interference between two vacuum states. This means that $p^{(0,0)}_{\mathrm{click}}(\mathrm{D}_{\mathrm{M}i}|01,\mathrm{b}2,2,M_{\min}+1) = 0$. If Eve sends Bob the signal $|\varphi_0\rangle$ or the signal $|\varphi_2\rangle$ (which happens with probability $r_{(0|0)} + r_{(2|0)}$) then in the time instance corresponding to the interference between the original signals, Bob observes the interference between one coherent state $|\alpha\rangle$ and one vacuum state. This means that $p^{(0,0)}_{\mathrm{click}}(\mathrm{D}_{\mathrm{M}i}|01,\mathrm{b}2,2,M_{\min}+1) = (q_{\mathrm{s}}+q_{\mathrm{f}})\gamma/p_{\mathrm{c}}$.

This means, that, in general, we find that

$$p^{(0,0)}_{(\mathrm{b}2,2,M_{\min}+1|01)} p^{(0,0)}_{\mathrm{click}}(\mathrm{D}_{\mathrm{M}i}|01,\mathrm{b}2,2,M_{\min}+1) = \begin{cases} p_{|0\rangle} q_{\mathrm{f}} q_{\mathrm{s}}(1-p_{\mathrm{c}})q(1-q_{\mathrm{p}})\gamma & \text{if } M_{\min}=2, \\ p_{|0\rangle} q_{\mathrm{f}} p_{\mathrm{c}}^{M_{\min}-2} p(0|\mathrm{c})(1-p_{\mathrm{c}})q(1-q_{\mathrm{p}})(q_{\mathrm{s}}+q_{\mathrm{f}})\gamma & \text{if } M_{\min}>2, \end{cases} \tag{146}$$

with $i = 1, 2$.

The situation where $M_{\min}+1 < l < M_{\max}+1$ is again analogous, being the main difference that now the probability $q$ is not included in $p^{(0,0)}_{(\mathrm{b}2,2,l|01)}$ as this probability is only relevant when $l = M_{\min}+1$. In particular, it is easy to show that in this case,

$$p^{(0,0)}_{(\mathrm{b}2,2,l|01)} = p_{|0\rangle} q_{\mathrm{f}} p_{\mathrm{c}}^{l-2} p(0|\mathrm{c})(1-p_{\mathrm{c}})(1-q_{\mathrm{p}}), \tag{147}$$

and the probability $p^{(0,0)}_{\mathrm{click}}(\mathrm{D}_{\mathrm{M}i}|01,\mathrm{b}2,2,l) = (q_{\mathrm{s}}+q_{\mathrm{f}})\gamma/p_{\mathrm{c}}$. That is, we obtain

$$p^{(0,0)}_{(\mathrm{b}2,2,l|01)} p^{(0,0)}_{\mathrm{click}}(\mathrm{D}_{\mathrm{M}i}|01,\mathrm{b}2,2,l) = p_{|0\rangle} q_{\mathrm{f}} p_{\mathrm{c}}^{l-3} p(0|\mathrm{c}) \times(1-p_{\mathrm{c}})(1-q_{\mathrm{p}})(q_{\mathrm{s}}+q_{\mathrm{f}})\gamma. \tag{148}$$

The result for the case $l = M_{\max}+1$ can be obtained directly from that of the case $M_{\min}+1 < l < M_{\max}+1$ by simply removing from the probability $p^{(0,0)}_{(\mathrm{b}2,2,l|01)}$ the term $1-p_{\mathrm{c}}$, as in this latter scenario is not necessary that Eve obtains an inconclusive result in the signal located in the last position of the block. This means that

$$p^{(0,0)}_{(\mathrm{b}2,2,M_{\max}+1|01)} p^{(0,0)}_{\mathrm{click}}(\mathrm{D}_{\mathrm{M}i}|01,\mathrm{b}2,2,M_{\max}+1) = p_{|0\rangle} q_{\mathrm{f}} \times p_{\mathrm{c}}^{M_{\max}-2} p(0|\mathrm{c})(1-q_{\mathrm{p}})(q_{\mathrm{s}}+q_{\mathrm{f}})\gamma. \tag{149}$$

By combining Eqs. (158)-(146)-(148)-(149) we obtain

$$p^{(0,0)}_{(\mathrm{b}2,2|01)} p^{(0,0)}_{\mathrm{click}}(\mathrm{D}_{\mathrm{M}i}|01,\mathrm{b}2,2) = \begin{cases} p_{|0\rangle} q_{\mathrm{f}}(1-q_{\mathrm{p}})\gamma\big[q_{\mathrm{s}}(1-p_{\mathrm{c}})q + p(0|\mathrm{c})(q_{\mathrm{s}}+q_{\mathrm{f}})p_{\mathrm{c}}\big] & \text{if } M_{\min}=2, \\ p_{|0\rangle} q_{\mathrm{f}} p(0|\mathrm{c})(1-q_{\mathrm{p}})(q_{\mathrm{s}}+q_{\mathrm{f}})\gamma p_{\mathrm{c}}^{M_{\min}-2}\big[p_{\mathrm{c}} + (1-p_{\mathrm{c}})q\big] & \text{if } M_{\min}>2, \end{cases} \tag{150}$$

with $i = 1, 2$. The remaining $(m, n)$ cases can be treated similarly and we omit the detailed calculations here for simplicity. The summation in Eq. (134) gives

$$\begin{aligned} p_{(\mathrm{b}2,2|01)} p_{\mathrm{click}}(\mathrm{D}_{\mathrm{M}1}|01,\mathrm{b}2,2) &= \begin{cases} p_{|0\rangle}(1-q_{\mathrm{p}})\Big[p_{\mathrm{c}}\Big(q_{\mathrm{f}}(q_{\mathrm{f}}+q_{\mathrm{s}})\gamma + \big(q_{\mathrm{f}} + \big[p(1|\mathrm{c})+p(2|\mathrm{c})\big]q_{\mathrm{s}}\big)\Theta\Big) + \\ +(1-p_{\mathrm{c}})qq_{\mathrm{f}}\Big(2q_{\mathrm{s}}(\gamma+\lambda) + q_{\mathrm{f}}(2\gamma+\lambda)\Big)\Big] & \text{if } M_{\min}=2, \\ p_{|0\rangle}(1-q_{\mathrm{p}})p_{\mathrm{c}}^{M_{\min}-2}\Big[p_{\mathrm{c}} + (1-p_{\mathrm{c}})q\Big]\Big[q_{\mathrm{f}}(q_{\mathrm{f}}+q_{\mathrm{s}})\gamma + \\ +\Big(q_{\mathrm{f}} + \big[p(1|\mathrm{c})+p(2|\mathrm{c})\big]q_{\mathrm{s}}\Big)\Theta\Big] & \text{if } M_{\min}>2, \end{cases} \\ p_{(\mathrm{b}2,2|01)} p_{\mathrm{click}}(\mathrm{D}_{\mathrm{M}2}|01,\mathrm{b}2,2) &= \begin{cases} p_{|0\rangle}(1-q_{\mathrm{p}})q_{\mathrm{f}}\gamma\Big[2p_{\mathrm{c}}(1-q)q_{\mathrm{f}} + p_{\mathrm{c}}\Big(1+p(1|\mathrm{c})+p(2|\mathrm{c})-2q\Big)q_{\mathrm{s}} + \\ +2q(q_{\mathrm{f}}+q_{\mathrm{s}})\Big] & \text{if } M_{\min}=2, \\ p_{|0\rangle}(1-q_{\mathrm{p}})p_{\mathrm{c}}^{M_{\min}-2}q_{\mathrm{f}}\gamma\Big[p_{\mathrm{c}} + (1-p_{\mathrm{c}})q\Big]\Big[2q_{\mathrm{f}} + \\ +\big[1+p(1|\mathrm{c})+p(2|\mathrm{c})\big]q_{\mathrm{s}}\Big] & \text{if } M_{\min}>2. \end{cases} \end{aligned} \tag{151}$$

*Position 3:* This case is totally analogous to that corresponding to position 3 in blocks of the type "b1". There are only two differences. First, in Eq. (123) we need to replace the probability $p(1|\mathrm{c})$ with $p(0|\mathrm{c})$. This is so because in the example we are considering the first signal of the block is actually in the state $|\varphi_0\rangle$ (instead of being in the state $|\varphi_1\rangle$). The second difference is that here we need to include the term $1-q_{\mathrm{p}}$ that Eve decides to send a block with non-vacuum signals to Bob even if the block is not of the type "01". By making these changes in Eq. (123), we obtain

$$p_{(\mathrm{b2},3|01)}^{(0,0)} p_{\mathrm{click}}^{(0,0)}(\mathrm{D_{M1}}|01,\mathrm{b2},3) = \begin{cases} p_{|0\rangle} p(0|\mathrm{c})^2 (1-q_{\mathrm{p}}) \xi \frac{p_{\mathrm{c}}^2 (1-p_{\mathrm{c}}^{M_{\max}-3})}{1-p_{\mathrm{c}}} & \text{if } M_{\min} < 4 \text{ and } M_{\max} \geq 4, \\ p_{|0\rangle} p(0|\mathrm{c})^2 (1-q_{\mathrm{p}}) p_{\mathrm{c}}^{M_{\min}-2} \xi \sigma & \text{if } M_{\min} \geq 4 \text{ and } M_{\max} \geq M_{\min}+1, \end{cases}$$
$$p_{(\mathrm{b2},3|01)}^{(0,0)} p_{\mathrm{click}}^{(0,0)}(\mathrm{D_{M2}}|01,\mathrm{b2},3) = \begin{cases} 2p_{|0\rangle} p(0|\mathrm{c})^2 (1-q_{\mathrm{p}}) q_{\mathrm{f}} (q_{\mathrm{s}}+q_{\mathrm{f}}) \gamma \frac{p_{\mathrm{c}}^2 (1-p_{\mathrm{c}}^{M_{\max}-3})}{1-p_{\mathrm{c}}} & \text{if } M_{\min} < 4 \text{ and } M_{\max} \geq 4, \\ 2p_{|0\rangle} p(0|\mathrm{c})^2 (1-q_{\mathrm{p}}) p_{\mathrm{c}}^{M_{\min}-2} q_{\mathrm{f}} (q_{\mathrm{s}}+q_{\mathrm{f}}) \gamma \sigma & \text{if } M_{\min} \geq 4 \text{ and } M_{\max} \geq M_{\min}+1, \end{cases} \tag{152}$$

where the parameters $\xi$ and $\sigma$ are given, respectively by Eqs. (119) and (124). Performing the summation over $(m,n)$ in Eq. (134) we have that

$$p_{(\mathrm{b2},3|01)} p_{\mathrm{click}}(\mathrm{D_{M1}}|01,\mathrm{b2},3) = \begin{cases} p_{|0\rangle} \left[1-q_{01}\right] (1-q_{\mathrm{p}}) \xi \frac{p_{\mathrm{c}}^2 (1-p_{\mathrm{c}}^{M_{\max}-3})}{1-p_{\mathrm{c}}} & \text{if } M_{\min} < 4 \text{ and } M_{\max} \geq 4, \\ p_{|0\rangle} \left[1-q_{01}\right] (1-q_{\mathrm{p}}) p_{\mathrm{c}}^{M_{\min}-2} \xi \sigma & \text{if } M_{\min} \geq 4 \text{ and } M_{\max} \geq M_{\min}+1, \end{cases}$$
$$p_{(\mathrm{b2},3|01)} p_{\mathrm{click}}(\mathrm{D_{M2}}|01,\mathrm{b2},3) = \begin{cases} 2p_{|0\rangle} \left[1-q_{01}\right] (1-q_{\mathrm{p}}) q_{\mathrm{f}} (q_{\mathrm{s}}+q_{\mathrm{f}}) \gamma \frac{p_{\mathrm{c}}^2 (1-p_{\mathrm{c}}^{M_{\max}-3})}{1-p_{\mathrm{c}}} & \text{if } M_{\min} < 4 \text{ and } M_{\max} \geq 4, \\ 2p_{|0\rangle} \left[1-q_{01}\right] (1-q_{\mathrm{p}}) p_{\mathrm{c}}^{M_{\min}-2} q_{\mathrm{f}} (q_{\mathrm{s}}+q_{\mathrm{f}}) \gamma \sigma & \text{if } M_{\min} \geq 4 \text{ and } M_{\max} \geq M_{\min}+1, \end{cases} \tag{153}$$

where $q_{01}$ is given by Eq. (26) and we have introduced the term $1-q_{01}$ since $(1,0)$ is the only case which is not included in the summation over $(m,n)$.

*Position 4:* This case is also totally analogous to that corresponding to position 4 in blocks of the type "b1", being the only differences those already mentioned in the previous paragraph. That is, in Eq. (133) we have to replace $p(1|\mathrm{c})$ with $p(0|\mathrm{c})$ and, moreover, we need to include the term $1-q_{\mathrm{p}}$. By performing these two changes in Eq. (133), we obtain

$$p_{(\mathrm{b2},4|01)}^{(0,0)} p_{\mathrm{click}}^{(0,0)}(\mathrm{D_{M1}}|01,\mathrm{b2},4) = \begin{cases} p_{|0\rangle} q_{\mathrm{s}} p(0|\mathrm{c})(1-q_{\mathrm{p}}) p_{\mathrm{c}} \Theta & \text{if } M_{\min} = 2, \\ p_{|0\rangle} q_{\mathrm{s}} p(0|\mathrm{c})(1-q_{\mathrm{p}}) p_{\mathrm{c}}^{M_{\min}-2} \big[p_{\mathrm{c}} + (1-p_{\mathrm{c}}) q\big] \Theta & \text{if } M_{\min} > 2, \end{cases}$$
$$p_{(\mathrm{b2},4|01)}^{(0,0)} p_{\mathrm{click}}^{(0,0)}(\mathrm{D_{M2}}|01,\mathrm{b2},4) = \begin{cases} p_{|0\rangle} q_{\mathrm{s}} q_{\mathrm{f}} p(0|\mathrm{c})(1-q_{\mathrm{p}}) \gamma p_{\mathrm{c}} & \text{if } M_{\min} = 2, \\ p_{|0\rangle} q_{\mathrm{s}} q_{\mathrm{f}} p(0|\mathrm{c})(1-q_{\mathrm{p}}) \gamma p_{\mathrm{c}}^{M_{\min}-2} \big[p_{\mathrm{c}} + (1-p_{\mathrm{c}}) q\big] & \text{if } M_{\min} > 2. \end{cases} \tag{154}$$

The remaining $(m,n)$ cases can be obtained easily by taking into account that Position 4 is very similar to Position 2. As for the case of "b1" type blocks, one has to omit the case of $l = M_{\min}+1$ with $M_{\min}=2$ since these have already been counted when considering Position 2. Also note that one can obtain the terms for $(m,n)$ from the corresponding results for Position 2 since a "0"("1") signal on the left in Position 4 is equivalent to a "1"("0") signal on the right in Position 2 when considering the interference between the two signals sent by Alice. Thus the summation in $(m,n)$ in Eq. (134) gives

$$p_{(\mathrm{b2},4|01)}p_{\mathrm{click}}(\mathrm{D_{M1}}|01,\mathrm{b2},4)=\begin{cases}p_{|0\rangle}(1-q_{\mathrm{p}})p_{\mathrm{c}}\Big[q_{\mathrm{f}}(q_{\mathrm{f}}+q_{\mathrm{s}})\gamma+\Big(q_{\mathrm{f}}+\big[1-p(1|\mathrm{c})\big]q_{\mathrm{s}}\Big)\Theta\Big] & \text{if } M_{\min}=2,\\ p_{|0\rangle}(1-q_{\mathrm{p}})p_{\mathrm{c}}^{M_{\min}-2}\Big[p_{\mathrm{c}}+(1-p_{\mathrm{c}})q\Big]\Big[q_{\mathrm{f}}(q_{\mathrm{f}}+q_{\mathrm{s}})\gamma+ & \\ +\Big(q_{\mathrm{f}}+\big[1-p(1|\mathrm{c})\big]q_{\mathrm{s}}\Big)\Theta\Big] & \text{if } M_{\min}>2,\end{cases}$$

$$p_{(\mathrm{b2},4|01)}p_{\mathrm{click}}(\mathrm{D_{M2}}|01,\mathrm{b2},4)=\begin{cases}p_{|0\rangle}(1-q_{\mathrm{p}})q_{\mathrm{f}}p_{\mathrm{c}}\gamma\Big[2q_{\mathrm{f}}+\Big(2-p(1|\mathrm{c})\Big)q_{\mathrm{s}}\Big] & \text{if } M_{\min}=2,\\ p_{|0\rangle}(1-q_{\mathrm{p}})p_{\mathrm{c}}^{M_{\min}-2}q_{\mathrm{f}}\gamma\Big[p_{\mathrm{c}}+(1-p_{\mathrm{c}})q\Big]\Big[2q_{\mathrm{f}}+\Big(2-p(1|\mathrm{c})\Big)q_{\mathrm{s}}\Big] & \text{if } M_{\min}>2.\end{cases} \quad (155)$$

*Position 5:* In this case, the signal $|\varphi_0\rangle$ is replaced by Eve with a vacuum signal, while the signal $|\varphi_1\rangle$ is replaced by Eve with a signal $|\varphi_0\rangle$. This means that in the time instance corresponding to the interference between the original signals $|\varphi_0\rangle\otimes|\varphi_1\rangle$ emitted by Alice, Bob actually observes the interference between two vacuum signals. This means that $p_{\mathrm{click}}^{(0,0)}(\mathrm{D}_{\mathrm{M}i}|01,\mathrm{b2},5)=0$, and thus

$$p_{(\mathrm{b2},5|01)}^{(0,0)}p_{\mathrm{click}}^{(0,0)}(\mathrm{D}_{\mathrm{M}i}|01,\mathrm{b2},5)=0, \quad (156)$$

with $i=1,2$. The remaining $(m,n)$ cases can be obtained similarly and the summation over $(m,n)$ in Eq. (134) gives

$$p_{(\mathrm{b2},5|01)}p_{\mathrm{click}}(\mathrm{D}_{\mathrm{M}i}|01,\mathrm{b2},5)=p_{|0\rangle}(1-q_{\mathrm{p}})\gamma p_{\mathrm{c}}^{M_{\min}-1}\times(q_s+q_f)\big[p_{\mathrm{c}}+(1-p_{\mathrm{c}})q\big], \quad (157)$$

for $i=1,2$, which, as expected, coincides with the result obtained for Position 1 in Eq. (143).

### 3. Blocks of the type "b3"

Finally, here we study blocks of the type "b3". These are blocks which originally are not of the form "01" but Eve decides to process them (which happens with probability $q_{\mathrm{p}}$) and she successfully transforms them in blocks of the form "01".

Like above, for each possible position $k=1,\ldots,5$ (see Fig. 11), in which the original signals, $|\varphi_0\rangle\otimes|\varphi_1\rangle$, generated by Alice can be located with respect to the block, we will write

$$p_{(\mathrm{b3},k|01)}p_{\mathrm{click}}(\mathrm{D}_{\mathrm{M}i}|01,\mathrm{b3},k)=\sum_{l=M_{\min}+2}^{M_{\max}+1}p_{(\mathrm{b3},k,l|01)}\times p_{\mathrm{click}}(\mathrm{D}_{\mathrm{M}i}|01,\mathrm{b3},k,l), \quad (158)$$

where $l$ indicates once again the length of the block. Note, however, that in contrast to previous cases, now the minimum length of the block is $M_{\min}+2$ (instead of $M_{\min}+1$). This is so because in the blocks of the type "b3" Eve always replaces at least one non-vacuum signal with a vacuum signal, and it is necessary that the remaining total number of non-vacuum signals (within the block) is at least $M_{\min}$. Otherwise, Eve would send Bob a block with only vacuum states.

*Positions 1 and 5:* For the same reason like in the case of blocks of the type "b1" we have that

$$p_{\mathrm{click}}(\mathrm{D}_{\mathrm{M}i}|01,\mathrm{b3},1)=p_{\mathrm{click}}(\mathrm{D}_{\mathrm{M}i}|01,\mathrm{b3},5)=0, \quad (159)$$

for $i=1,2$. Note that position 1 (position 5) implies that Eve has replaced the signal $|\varphi_0\rangle$ with $|\varphi_1\rangle$ (a vacuum signal) and the signal $|\varphi_1\rangle$ with a vacuum signal ($|\varphi_0\rangle$). That is, in both cases we have that at the time instance corresponding to the interference between the original signals $|\varphi_0\rangle$ and $|\varphi_1\rangle$ prepared by Alice, Bob observes the interference between two vacuum states and, thus, there is no click in his detectors.

*Position 2:* Let us start with the case $l=M_{\min}+2$ with $M_{\min}=2$. In this scenario, $p_{(\mathrm{b3},2,M_{\min}+2|01)}$ means that any of the two situations illustrated in Figs. 14(a) and (b) happens. The first one (see Fig. 14(a)) implies that: in the time instance "0" Eve sends Bob a vacuum state (which happens with probability $p_{|0\rangle}$), then Eve correctly identifies the signals $|\varphi_0\rangle\otimes|\varphi_1\rangle$ emitted by Alice (which happens with probability $q_{\mathrm{s}}^2$), Eve's measurement result on the next signal is not equal to $|\varphi_0\rangle$ (which happens with probability $p_{\mathrm{c}}p(\neq 0|\mathrm{c})$, with $p(\neq j|\mathrm{c})$ given by Eq. (24)), Eve obtains an inconclusive result in the following signal (which happens with probability $1-p_{\mathrm{c}}$), and with probability $q_{\mathrm{p}}$ Eve decides to process the block (as it is not of the form "01").

The second possible situation (see Fig. 14(b)) implies that: in the time instance "0" Eve sends Bob a vacuum state (which happens with probability $p_{|0\rangle}$), then Eve's measurement result on the next signal is not equal to $|\varphi_1\rangle$ (which happens with probability $p_{\mathrm{c}}p(\neq 1|\mathrm{c})$), Eve correctly identifies the signals $|\varphi_0\rangle\otimes|\varphi_1\rangle$ emitted by Alice (which happens again with probability $q_{\mathrm{s}}^2$), Eve obtains an inconclusive result in the following signal (which happens with probability $1-p_{\mathrm{c}}$), and with probability $q_{\mathrm{p}}$ Eve decides to process the block (as it is not of the form "01").

This means that

$$\begin{aligned}p_{(\mathrm{b3},2,M_{\min}+2|01)}&=p_{|0\rangle}q_{\mathrm{s}}^2p_{\mathrm{c}}(1-p_{\mathrm{c}})q_{\mathrm{p}}\\&\times[p(\neq 0|\mathrm{c})+p(\neq 1|\mathrm{c})]\\&=2p_{|0\rangle}q_{\mathrm{s}}^2p_{\mathrm{c}}(1-p_{\mathrm{c}})q_{\mathrm{p}}p(\neq 0|\mathrm{c}),\end{aligned} \quad (160)$$

if $M_{\min}=2$. Note that in the second equality we have used the fact that $p(\neq 0|\mathrm{c})=p(\neq 1|\mathrm{c})$. In both scenar-

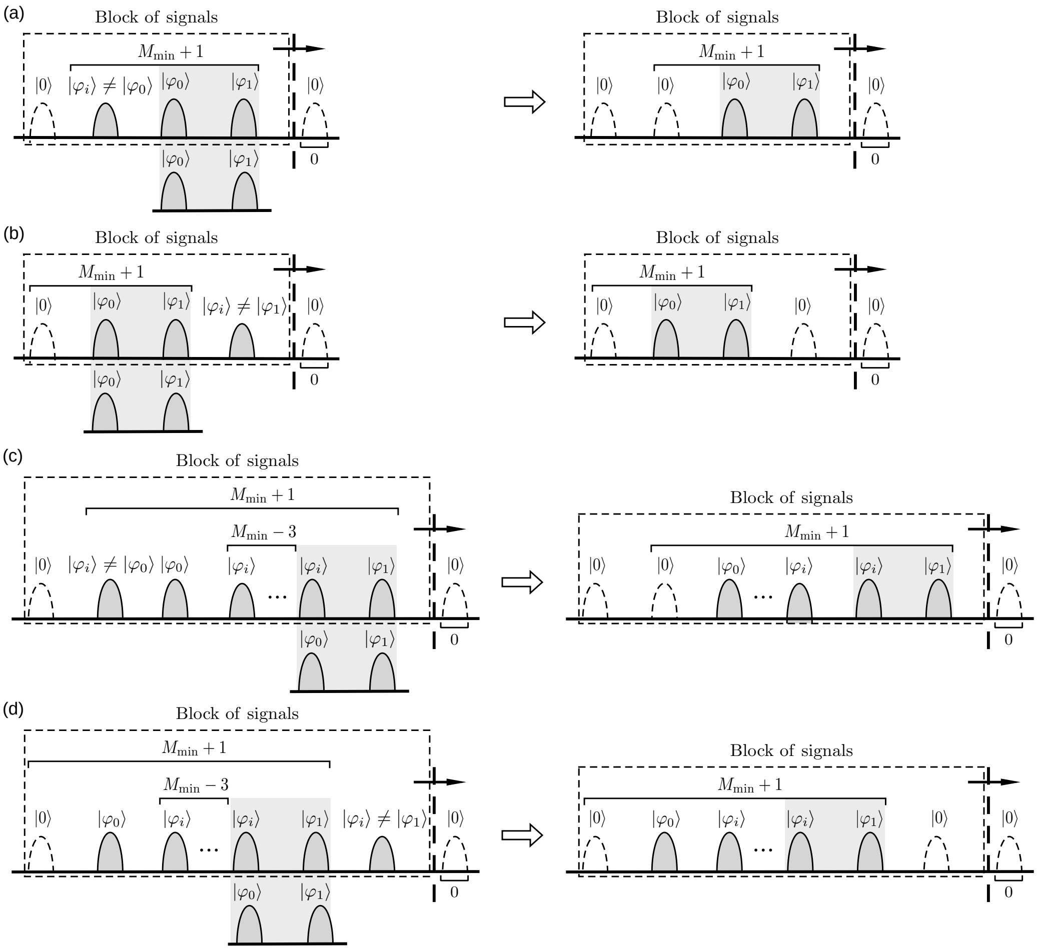


FIG. 14. Illustration of the possible scenarios when the original signals $|\varphi_0\rangle \otimes |\varphi_1\rangle$ emitted by Alice occupy the position 2 in a block of the type "b3" of length $l = M_{\min} + 2$. Subfigures (a) and (b) represent the case $M_{\min} = 2$, while subfigures (c) and (d) show the case $M_{\min} > 2$. For example, on the left hand side of subfigure (a) we illustrate the measurement results obtained by Eve (including also the vacuum signal in the time instance "0" that precedes the block) together with the location of the original signals emitted by Alice. On the right hand side of that subfigure we illustrate the block of signals that Eve finally sends to Bob. The explanation of the other subfigures is analogous.

ios, at the time instance corresponding to the interference between the original signals $|\varphi_0\rangle$ and $|\varphi_1\rangle$ emitted by Alice, Bob observes the interference between two coherent states and, thus,

$$p_{\text{click}}(\text{D}_{\text{M1}}|01, \text{b3}, 2, M_{\min} + 2) = \lambda$$
$$p_{\text{click}}(\text{D}_{\text{M2}}|01, \text{b3}, 2, M_{\min} + 2) = 0. \qquad (161)$$

On the other hand, if $l = M_{\min} + 2$ with $M_{\min} > 2$ there are also two possibilities. They are illustrated in Figs. 14(c) and (d). The first one implies that (see Fig. 14(c)): in the time instance "0" Eve sends Bob a vacuum state, next Eve correctly identifies the signal $|\varphi_1\rangle$ emitted by Alice, also Eve obtains a conclusive result when measuring the signal $|\varphi_0\rangle$, then Eve obtains $M_{\min} - 3$ further conclusive results when measuring the next $M_{\min} - 3$ signals, next Eve obtains the result $|\varphi_0\rangle$ in the following signal, also she obtains a conclusive result different from $|\varphi_0\rangle$ when she measures the signal located in position $M_{\min} + 1$, Eve obtains an inconclusive result in the following signal (located in the position $M_{\min} + 2$), and with probability $q_{\text{p}}$ Eve decides to process the block.

The second possibility (see Fig. 14(d)) is as follows: in the time instance "0" Eve sends Bob a vacuum state, next Eve obtains a conclusive result different from $|\varphi_1\rangle$ when she measures the signal located in the first position of the block, next Eve correctly identifies the signal $|\varphi_1\rangle$ emitted by Alice, also Eve obtains a conclusive result when measuring the signal $|\varphi_0\rangle$, then Eve obtains $M_{\min} - 3$ further conclusive results when measuring the next $M_{\min} - 3$ signals, next Eve obtains the result $|\varphi_0\rangle$ in the following signal (located in the position $M_{\min} + 1$), Eve obtains an inconclusive result in the following signal (located in the position $M_{\min} + 2$), and with probability $q_{\text{p}}$ Eve decides to process the block.

This means that

$$
\begin{aligned}
p_{(\mathrm{b3},2,M_{\min}+2|01)} &= p_{|0\rangle} q_{\mathrm{s}} p_{\mathrm{c}}^{M_{\min}} p(0|\mathrm{c})(1-p_{\mathrm{c}}) q_{\mathrm{p}} \\
&\times [p(\neq 0|\mathrm{c}) + p(\neq 1|\mathrm{c})] \\
&= 2 p_{|0\rangle} q_{\mathrm{s}} p_{\mathrm{c}}^{M_{\min}} p(0|\mathrm{c})(1-p_{\mathrm{c}}) q_{\mathrm{p}} p(\neq 0|\mathrm{c}),
\end{aligned} \tag{162}
$$

if $M_{\min} > 2$, and where we have used again the fact that $p(\neq 0|\mathrm{c}) = p(\neq 1|\mathrm{c})$. In both scenarios, we have that with probability $r_{(0|0)} + r_{(2|0)}$, with $r_{(i|j)}$ given by Eq. (105) Bob observes at the time instance corresponding to the interference between the original signals $|\varphi_0\rangle$ and $|\varphi_1\rangle$ emitted by Alice, the interference between two coherent states, while with probability $r_{(1|0)}$ he observes at that time instance the interference between a coherent state and the vacuum state. This means that $p_{\mathrm{click}}(\mathrm{D}_{\mathrm{M}i}|01, \mathrm{b3}, 2, M_{\min}+2)$ is given by Eq. (106), *i.e.*,

$$
\begin{aligned}
p_{\mathrm{click}}(\mathrm{D}_{\mathrm{M1}}|01, \mathrm{b3}, 2, M_{\min}+2) &= \frac{q_{\mathrm{s}} + q_{\mathrm{f}}}{p_{\mathrm{c}}}\lambda + \frac{q_{\mathrm{f}}}{p_{\mathrm{c}}}\gamma = \frac{\Theta}{p_{\mathrm{c}}}, \\
p_{\mathrm{click}}(\mathrm{D}_{\mathrm{M2}}|01, \mathrm{b3}, 2, M_{\min}+2) &= \frac{q_{\mathrm{f}}}{p_{\mathrm{c}}}\gamma.
\end{aligned} \tag{163}
$$

By combining Eqs. (160)-(161)-(162)-(163) we obtain

$$
\begin{aligned}
p_{(\mathrm{b3},2,M_{\min}+2|01)} p_{\mathrm{click}}(\mathrm{D}_{\mathrm{M1}}|01, \mathrm{b3}, 2, M_{\min}+2) &= \begin{cases} q_{\mathrm{s}} p_{\mathrm{c}} \lambda \omega & \text{if } M_{\min} = 2, \\ p_{\mathrm{c}}^{M_{\min}-1} p(0|\mathrm{c}) \Theta \omega & \text{if } M_{\min} > 2, \end{cases} \\
p_{(\mathrm{b3},2,M_{\min}+2|01)} p_{\mathrm{click}}(\mathrm{D}_{\mathrm{M2}}|01, \mathrm{b3}, 2, M_{\min}+2) &= \begin{cases} 0 & \text{if } M_{\min} = 2, \\ q_{\mathrm{f}} p_{\mathrm{c}}^{M_{\min}-1} p(0|\mathrm{c}) \gamma \omega & \text{if } M_{\min} > 2, \end{cases}
\end{aligned} \tag{164}
$$

with the parameter $\omega$ given by

$$
\omega = 2 p_{|0\rangle} q_{\mathrm{s}} (1-p_{\mathrm{c}}) q_{\mathrm{p}} p(\neq 0|\mathrm{c}). \tag{165}
$$

Next we will consider the case $M_{\min}+2 < l < M_{\max}+1$ with $M_{\min} = 2$. There are different possibilities depending on the time instance that the signal $|\varphi_1\rangle$ occupies with respect to the block, which, in this case, can vary from $l' = 1$ till $l' = l-2$. This will become clear below. To be precise, we will rewrite $p_{(\mathrm{b3},2,l|01)} p_{\mathrm{click}}(\mathrm{D}_{\mathrm{M}i}|01, \mathrm{b3}, 2, l)$ as follows

$$
\begin{aligned}
p_{(\mathrm{b3},2,l|01)} p_{\mathrm{click}}(\mathrm{D}_{\mathrm{M}i}|01, \mathrm{b3}, 2, l) &= \sum_{l'=1}^{l-2} p_{(\mathrm{b3},2,l,l'|01)} \\
&\times p_{\mathrm{click}}(\mathrm{D}_{\mathrm{M}i}|01, \mathrm{b3}, 2, l, l'),
\end{aligned} \tag{166}
$$

where $p_{(\mathrm{b3},2,l,l'|01)}$ is the conditional probability that the signals $|\varphi_0\rangle \otimes |\varphi_1\rangle$ sent by Alice actually correspond to the time instance $l'$ of a block of the type "b3" of length $l$ and they occupy the position 2 after the processing performed by Eve, and the probability $p_{\mathrm{click}}(\mathrm{D}_{\mathrm{M}i}|01, \mathrm{b3}, 2, l, l')$ can be defined analogously.

In particular, let us consider first the situation where $|\varphi_1\rangle$ occupies the time instance $l' = 1$. This scenario is illustrated in Fig. 14(a). We find then that $p_{(\mathrm{b3},2,1|01)}$ means that: in the time instance "0" Eve sends Bob a vacuum state, next Eve correctly identifies the signal $|\varphi_1\rangle$ emitted by Alice, also Eve obtains a conclusive result when measuring the signal $|\varphi_0\rangle$, then Eve obtains $l-5$ further conclusive results when measuring the next $l-5$ signals, next Eve obtains the result $|\varphi_0\rangle$ in the following signal, also she obtains a conclusive result different from $|\varphi_0\rangle$ when she measures the signal located in position $l-1$, Eve obtains an inconclusive result in the following signal (located in the position $l$), and with probability $q_{\mathrm{p}}$ Eve decides to process the block. This corresponds to the first illustration in Fig. 14(a).

Alternatively (if $l \geq 6$), Eve can also send Bob a vacuum state in the time instance "0", next Eve correctly identifies the signal $|\varphi_1\rangle$, also Eve obtains a conclusive result when measuring the signal $|\varphi_0\rangle$, then Eve obtains $l-6$ further conclusive results when measuring the next $l-6$ signals, next Eve obtains the result $|\varphi_0\rangle$ in the following signal, also she obtains a conclusive result different from $|\varphi_0\rangle$ when she measures the signals located in positions $l-2$ and $l-1$, Eve obtains an inconclusive result in the following signal (located in the position $l$), and with probability $q_{\mathrm{p}}$ Eve decides to process the block. This corresponds to the second illustration in Fig. 14(a).

In total, we have $l-4$ cases similar to the two cases described above. In all these cases, the probabilities $p_{\mathrm{click}}(\mathrm{D}_{\mathrm{M}i}|01, \mathrm{b3}, 2, l, l')$ are given by Eq. (106), *i.e.*,

$$
\begin{aligned}
p_{\mathrm{click}}(\mathrm{D}_{\mathrm{M1}}|01, \mathrm{b3}, 2, l, 1) &= \frac{q_{\mathrm{s}} + q_{\mathrm{f}}}{p_{\mathrm{c}}}\lambda + \frac{q_{\mathrm{f}}}{p_{\mathrm{c}}}\gamma = \frac{\Theta}{p_{\mathrm{c}}}, \\
p_{\mathrm{click}}(\mathrm{D}_{\mathrm{M2}}|01, \mathrm{b3}, 2, l, 1) &= \frac{q_{\mathrm{f}}}{p_{\mathrm{c}}}\gamma.
\end{aligned} \tag{167}
$$

Finally, there is an additional case which corresponds to the last illustration shown in Fig. 14(a). That is, here Eve sends Bob a vacuum state in the time instance "0", next Eve correctly identifies both the signals $|\varphi_0\rangle$ and $|\varphi_1\rangle$, also Eve obtains $l-3$ conclusive result different from $|\varphi_0\rangle$ when she measures the following signals, Eve obtains an inconclusive result in the following signal (located in the position $l$), and with probability $q_{\mathrm{p}}$ Eve decides to process the block. In this latter case, we have that $p_{\mathrm{click}}(\mathrm{D}_{\mathrm{M1}}|01, \mathrm{b3}, 2, l, 1) = \lambda$ and $p_{\mathrm{click}}(\mathrm{D}_{\mathrm{M2}}|01, \mathrm{b3}, 2, l, 1) = 0$.

Putting the results above together, and taking into account that $p(\neq 0|\mathrm{c}) = 1 - p(0|\mathrm{c})$, we have that:

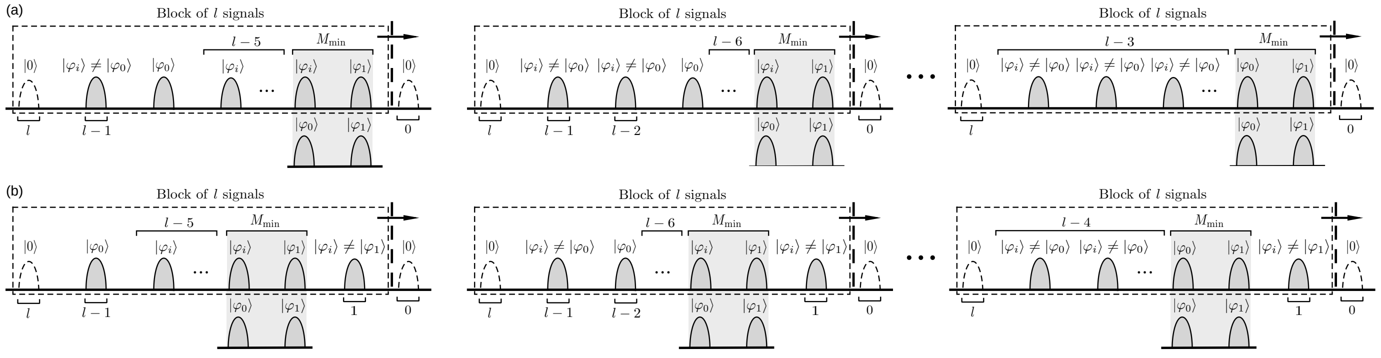


FIG. 15. (a) Illustration of the different possibilities for the original signals $|\varphi_0\rangle \otimes |\varphi_1\rangle$ (prepared by Alice) to correspond to the time instance $l' = 1$ of a block of signals of the type "b3" of length $l$, such that they occupy the position 2 after the processing performed by Eve. (b) The same like subfigure (a) but now referred to $l' = 2$.

$$
\begin{aligned}
p_{(\mathrm{b3},2,l,1|01)} p_{\mathrm{click}}(\mathrm{D_{M1}}|01,\mathrm{b3},2,l,1) &= p_{|0\rangle} q_{\mathrm{s}} p_{\mathrm{c}}^{3} p(0|\mathrm{c}) p(\neq 0|\mathrm{c})(1-p_{\mathrm{c}}) q_{\mathrm{p}} \sum_{k=0}^{l-5} \left[p_{\mathrm{c}} p(\neq 0|\mathrm{c})\right]^{k} p_{\mathrm{c}}^{l-5-k} \left[\frac{q_{\mathrm{s}}+q_{\mathrm{f}}}{p_{\mathrm{c}}}\lambda + \frac{q_{\mathrm{f}}}{p_{\mathrm{c}}}\gamma\right] \\
&\quad + p_{|0\rangle} q_{\mathrm{s}}^{2} p_{\mathrm{c}}^{l-3} p(\neq 0|\mathrm{c})^{l-3}(1-p_{\mathrm{c}}) q_{\mathrm{p}} \lambda \\
&= p_{|0\rangle} q_{\mathrm{s}} (1-p_{\mathrm{c}}) q_{\mathrm{p}} p_{\mathrm{c}}^{l-3} p(\neq 0|\mathrm{c}) \left\{ q_{\mathrm{s}} p(\neq 0|\mathrm{c})^{l-4}\lambda + [1-p(\neq 0|\mathrm{c})^{l-4}]\Theta \right\}, \\
p_{(\mathrm{b3},2,l,1|01)} p_{\mathrm{click}}(\mathrm{D_{M2}}|01,\mathrm{b3},2,l,1) &= p_{|0\rangle} q_{\mathrm{s}} p_{\mathrm{c}}^{3} p(0|\mathrm{c}) p(\neq 0|\mathrm{c})(1-p_{\mathrm{c}}) q_{\mathrm{p}} \sum_{k=0}^{l-5} \left[p_{\mathrm{c}} p(\neq 0|\mathrm{c})\right]^{k} p_{\mathrm{c}}^{l-5-k} \frac{q_{\mathrm{f}}}{p_{\mathrm{c}}}\gamma \\
&= p_{|0\rangle} q_{\mathrm{s}} (1-p_{\mathrm{c}}) q_{\mathrm{p}} p_{\mathrm{c}}^{l-3} p(\neq 0|\mathrm{c})[1-p(\neq 0|\mathrm{c})^{l-4}] q_{\mathrm{f}} \gamma. \qquad (168)
\end{aligned}
$$

Let us now focus in the situation where $|\varphi_1\rangle$ occupies the time instance $l' = 2$. This scenario is illustrated in Fig. 14(b). In this case, $p_{(\mathrm{b3},2,l,2|01)}$ implies that: in the time instance "0" Eve sends Bob a vacuum state, next Eve obtains a conclusive result different from $|\varphi_1\rangle$ when she measures the signal located in position 1, then Eve correctly identifies the signal $|\varphi_1\rangle$ emitted by Alice, also Eve obtains a conclusive result when measuring the signal $|\varphi_0\rangle$, then Eve obtains $l-5$ further conclusive results when measuring the next $l-5$ signals, next Eve obtains the result $|\varphi_0\rangle$ in the following signal (which is located in the position $l-1$), Eve obtains an inconclusive result in the following signal (located in the position $l$), and with probability $q_{\mathrm{p}}$ Eve decides to process the block. This corresponds to the first illustration shown in Fig. 14(b).

Alternatively (if $l \geq 6$), Eve can also send Bob a vacuum state in the time instance "0", next Eve obtains a conclusive result different from $|\varphi_1\rangle$ when she measures the signal located in position 1, then Eve correctly identifies the signal $|\varphi_1\rangle$ emitted by Alice, also Eve obtains a conclusive result when measuring the signal $|\varphi_0\rangle$, then Eve obtains $l-6$ further conclusive results when measuring the next $l-6$ signals, next Eve obtains the result $|\varphi_0\rangle$ in the following signal (which is located in the position $l-2$), next Eve obtains a conclusive result different from $|\varphi_0\rangle$ when she measures the signal located in position $l-1$, Eve obtains an inconclusive result in the following signal (located in the position $l$), and with probability $q_{\mathrm{p}}$ Eve decides to process the block. This corresponds to the second illustration shown in Fig. 14(b).

In total, we have $l-4$ cases similar to the two cases described above. Like above, in all these cases we have that the probabilities $p_{\mathrm{click}}(\mathrm{D}_{\mathrm{M}i}|01,\mathrm{b3},2,l,2)$ are given by Eq. (106). Also, there is the additional case which corresponds to the last illustration shown in Fig. 14(b). Here, Eve sends Bob a vacuum state in the time instance "0", next Eve obtains a conclusive result different from $|\varphi_1\rangle$ when she measures the signal located in position 1, then she correctly identifies both the signals $|\varphi_0\rangle$ and $|\varphi_1\rangle$, also Eve obtains $l-4$ conclusive result different from $|\varphi_0\rangle$ when she measures the following signals, Eve obtains an inconclusive result in the following signal (located in the position $l$), and with probability $q_{\mathrm{p}}$ Eve decides to process the block. In this latter case, we have that $p_{\mathrm{click}}(\mathrm{D_{M1}}|01,\mathrm{b3},2,l,2) = \lambda$ and $p_{\mathrm{click}}(\mathrm{D_{M2}}|01,\mathrm{b3},2,l,2) = 0$.

Putting all together we find that

$$p_{(\mathrm{b3},2,l,2|01)}p_{\mathrm{click}}(\mathrm{D_{M1}}|01,\mathrm{b3},2,l,2) = p_{|0\rangle}q_{\mathrm{s}}p_{\mathrm{c}}^3 p(0|\mathrm{c})p(\neq 1|\mathrm{c})(1-p_{\mathrm{c}})q_{\mathrm{p}}\sum_{k=0}^{l-5}[p_{\mathrm{c}}p(\neq 0|\mathrm{c})]^k p_{\mathrm{c}}^{l-5-k}\left[\frac{q_{\mathrm{s}}+q_{\mathrm{f}}}{p_{\mathrm{c}}}\lambda+\frac{q_{\mathrm{f}}}{p_{\mathrm{c}}}\gamma\right]$$
$$+ p_{|0\rangle}q_{\mathrm{s}}^2 p(\neq 1|\mathrm{c})p_{\mathrm{c}}^{l-3}p(\neq 0|\mathrm{c})^{l-4}(1-p_{\mathrm{c}})q_{\mathrm{p}}\lambda$$
$$= p_{|0\rangle}q_{\mathrm{s}}(1-p_{\mathrm{c}})q_{\mathrm{p}}p_{\mathrm{c}}^{l-3}p(\neq 1|\mathrm{c})\Big\{q_{\mathrm{s}}p(\neq 0|\mathrm{c})^{l-4}\lambda+[1-p(\neq 0|\mathrm{c})^{l-4}]\Theta\Big\},$$
$$p_{(\mathrm{b3},2,l,2|01)}p_{\mathrm{click}}(\mathrm{D_{M2}}|01,\mathrm{b3},2,l,2) = p_{|0\rangle}q_{\mathrm{s}}p_{\mathrm{c}}^3 p(0|\mathrm{c})p(\neq 1|\mathrm{c})(1-p_{\mathrm{c}})q_{\mathrm{p}}\sum_{k=0}^{l-5}[p_{\mathrm{c}}p(\neq 0|\mathrm{c})]^k p_{\mathrm{c}}^{l-5-k}\frac{q_{\mathrm{f}}}{p_{\mathrm{c}}}\gamma$$
$$= p_{|0\rangle}q_{\mathrm{s}}(1-p_{\mathrm{c}})q_{\mathrm{p}}p_{\mathrm{c}}^{l-3}p(\neq 1|\mathrm{c})[1-p(\neq 0|\mathrm{c})^{l-4}]q_{\mathrm{f}}\gamma. \quad (169)$$

In general, by following the same reasoning like above, it can be shown that for any $l' = 1,\dots,l-2$, we have that

$$p_{(\mathrm{b3},2,l,l'|01)}p_{\mathrm{click}}(\mathrm{D_{M1}}|01,\mathrm{b3},2,l,l') = p_{|0\rangle}q_{\mathrm{s}}(1-p_{\mathrm{c}})q_{\mathrm{p}}p_{\mathrm{c}}^{l-3}p(\neq 1|\mathrm{c})^{l'-1}\Big\{q_{\mathrm{s}}p(\neq 0|\mathrm{c})^{l-l'-2}\lambda+p(0|\mathrm{c})\Theta \times\sum_{k=\max\{0,2-l'\}}^{l-l'-3}p(\neq 0|\mathrm{c})^k\Big\},$$
$$p_{(\mathrm{b3},2,l,l'|01)}p_{\mathrm{click}}(\mathrm{D_{M2}}|01,\mathrm{b3},2,l,l') = p_{|0\rangle}q_{\mathrm{s}}(1-p_{\mathrm{c}})q_{\mathrm{p}}p_{\mathrm{c}}^{l-3}p(\neq 1|\mathrm{c})^{l'-1}p(0|\mathrm{c})\sum_{k=\max\{0,2-l'\}}^{l-l'-3}p(\neq 0|\mathrm{c})^k q_{\mathrm{f}}\gamma. \quad (170)$$

with $l' = 1,\dots,l-2$.

By using Eqs. (171)-(166), as well as the fact that $p(\neq 0|\mathrm{c}) = p(\neq 1|\mathrm{c})$, this means that

$$p_{(\mathrm{b3},2,l|01)}p_{\mathrm{click}}(\mathrm{D_{M1}}|01,\mathrm{b3},2,l) = p_{|0\rangle}q_{\mathrm{s}}(1-p_{\mathrm{c}})q_{\mathrm{p}}p_{\mathrm{c}}^{l-3}\Big\{q_{\mathrm{s}}\lambda\sum_{l'=1}^{l-2}p(\neq 1|\mathrm{c})^{l'-1}p(\neq 0|\mathrm{c})^{l-l'-2}+p(0|\mathrm{c})\Theta \times\sum_{l'=1}^{l-2}p(\neq 1|\mathrm{c})^{l'-1}\sum_{k=\max\{0,2-l'\}}^{l-l'-3}p(\neq 0|\mathrm{c})^k\Big\}$$
$$= p_{|0\rangle}q_{\mathrm{s}}(1-p_{\mathrm{c}})q_{\mathrm{p}}p_{\mathrm{c}}^{l-3}\Big\{q_{\mathrm{s}}\lambda(l-2)p(\neq 0|\mathrm{c})^{l-3}+\Theta\Big[p(\neq 0|\mathrm{c})-(l-3)p(\neq 0|\mathrm{c})^{l-3} + \frac{p(\neq 0|\mathrm{c})-p(\neq 0|\mathrm{c})^{l-3}}{1-p(\neq 0|\mathrm{c})}\Big]\Big\},$$
$$p_{(\mathrm{b3},2,l|01)}p_{\mathrm{click}}(\mathrm{D_{M2}}|01,\mathrm{b3},2,l) = p_{|0\rangle}q_{\mathrm{s}}(1-p_{\mathrm{c}})q_{\mathrm{p}}p_{\mathrm{c}}^{l-3}p(0|\mathrm{c})q_{\mathrm{f}}\gamma\sum_{l'=1}^{l-2}p(\neq 1|\mathrm{c})^{l'-1}\sum_{k=\max\{0,2-l'\}}^{l-l'-3}p(\neq 0|\mathrm{c})^k \quad (171)$$
$$= p_{|0\rangle}q_{\mathrm{s}}(1-p_{\mathrm{c}})q_{\mathrm{p}}p_{\mathrm{c}}^{l-3}q_{\mathrm{f}}\gamma\Big[p(\neq 0|\mathrm{c})-(l-3)p(\neq 0|\mathrm{c})^{l-3}+\frac{p(\neq 0|\mathrm{c})-p(\neq 0|\mathrm{c})^{l-3}}{1-p(\neq 0|\mathrm{c})}\Big],$$

when $M_{\min}+2 < l < M_{\max}+1$ and $M_{\min}=2$.

Following the same procedure, it is easy to show that when $M_{\min}+2 < l < M_{\max}+1$ and $M_{\min}>2$ we have that

$$
\begin{aligned}
p_{(\mathrm{b3},2,l|01)}p_{\mathrm{click}}(\mathrm{D_{M1}}|01,\mathrm{b3},2,l) &= p_{|0\rangle}q_{\mathrm{s}}(1-p_{\mathrm{c}})q_{\mathrm{p}}p_{\mathrm{c}}^{l-3}p(0|\mathrm{c})\Theta\sum_{l'=1}^{l-M_{\min}}p(\neq 1|\mathrm{c})^{l'-1}\sum_{k=\max\{0,2-l'\}}^{l-l'-M_{\min}}p(\neq 0|\mathrm{c})^{k} \\
&= p_{|0\rangle}q_{\mathrm{s}}(1-p_{\mathrm{c}})q_{\mathrm{p}}p_{\mathrm{c}}^{l-3}\Theta\Bigg\{p(\neq 0|\mathrm{c})-(l-M_{\min})p(\neq 0|\mathrm{c})^{l-M_{\min}} \\
&\quad+\frac{p(\neq 0|\mathrm{c})-p(\neq 0|\mathrm{c})^{l-M_{\min}}}{1-p(\neq 0|\mathrm{c})}\Bigg\}, \\
p_{(\mathrm{b3},2,l|01)}p_{\mathrm{click}}(\mathrm{D_{M2}}|01,\mathrm{b3},2,l) &= \frac{q_{\mathrm{f}}\gamma}{\Theta}p_{(\mathrm{b3},2,l|01)}p_{\mathrm{click}}(\mathrm{D_{M1}}|01,\mathrm{b3},2,l). \qquad (172)
\end{aligned}
$$

The result for the case $l = M_{\max} + 1$ can be obtained directly from that of the case $M_{\min} + 1 < l < M_{\max} + 1$. For this, one only needs to remove the term $1 - p_{\mathrm{c}}$ from the probability $p_{(\mathrm{b3},2,l|01)}$. This means that

$$
\begin{aligned}
p_{(\mathrm{b3},2,M_{\max}+1|01)}p_{\mathrm{click}}(\mathrm{D_{M1}}|01,\mathrm{b3},2,M_{\max}+1) &= p_{|0\rangle}q_{\mathrm{s}}q_{\mathrm{p}}p_{\mathrm{c}}^{M_{\max}-2}\Bigg\{q_{\mathrm{s}}\lambda(M_{\max}-1)p(\neq 0|\mathrm{c})^{M_{\max}-2}+\Theta\Bigg[p(\neq 0|\mathrm{c}) \\
&\quad-(M_{\max}-2)p(\neq 0|\mathrm{c})^{M_{\max}-2}+\frac{p(\neq 0|\mathrm{c})-p(\neq 0|\mathrm{c})^{M_{\max}-2}}{1-p(\neq 0|\mathrm{c})}\Bigg]\Bigg\}, \\
p_{(\mathrm{b3},2,M_{\max}+1|01)}p_{\mathrm{click}}(\mathrm{D_{M2}}|01,\mathrm{b3},2,M_{\max}+1) &= p_{|0\rangle}q_{\mathrm{s}}q_{\mathrm{p}}p_{\mathrm{c}}^{M_{\max}-2}q_{\mathrm{f}}\gamma\Bigg[p(\neq 0|\mathrm{c})-(M_{\max}-2)p(\neq 0|\mathrm{c})^{M_{\max}-2} \\
&\quad+\frac{p(\neq 0|\mathrm{c})-p(\neq 0|\mathrm{c})^{M_{\max}-2}}{1-p(\neq 0|\mathrm{c})}\Bigg], \qquad (173)
\end{aligned}
$$

when $M_{\min} = 2$, and

$$
\begin{aligned}
p_{(\mathrm{b3},2,M_{\max}+1|01)}p_{\mathrm{click}}(\mathrm{D_{M1}}|01,\mathrm{b3},2,M_{\max}+1) &= p_{|0\rangle}q_{\mathrm{s}}q_{\mathrm{p}}p_{\mathrm{c}}^{M_{\max}-2}\Theta\Bigg\{p(\neq 0|\mathrm{c}) \\
&\quad-(M_{\max}-M_{\min}+1)p(\neq 0|\mathrm{c})^{M_{\max}-M_{\min}+1} \\
&\quad+\frac{p(\neq 0|\mathrm{c})-p(\neq 0|\mathrm{c})^{M_{\max}-M_{\min}+1}}{1-p(\neq 0|\mathrm{c})}\Bigg\} \\
p_{(\mathrm{b3},2,M_{\max}+1|01)}p_{\mathrm{click}}(\mathrm{D_{M2}}|01,\mathrm{b3},2,M_{\max}+1) &= \frac{q_{\mathrm{f}}\gamma}{\Theta}p_{(\mathrm{b3},2,M_{\max}+1|01)}p_{\mathrm{click}}(\mathrm{D_{M1}}|01,\mathrm{b3},2,M_{\max}+1), \qquad (174)
\end{aligned}
$$

when $M_{\min} > 2$.

Finally, by using the fact that

$$
p_{(\mathrm{b3},2|01)}p_{\mathrm{click}}(\mathrm{D}_{\mathrm{M}i}|01,\mathrm{b3},2) = \sum_{l=M_{\min}+2}^{M_{\max}+1}p_{(\mathrm{b3},2,l|01)} \times p_{\mathrm{click}}(\mathrm{D_{M1}}|01,\mathrm{b3},2,l), \qquad (175)
$$

together with Eqs. (164)-(171)-(173), and by taking $M_{\max} \geq M_{\min} + 3$ (which is what we do in the simulations, as ideally $M_{\max} >> M_{\min}$), we find that when $M_{\min} = 2$ the probability $p_{(\mathrm{b3},2|01)}p_{\mathrm{click}}(\mathrm{D}_{\mathrm{M}i}|01,\mathrm{b3},2)$ is given by

$$p_{(\mathrm{b3},2|01)}p_{\mathrm{click}}(\mathrm{D_{M1}}|01,\mathrm{b3},2)=p_{|0\rangle}q_{\mathrm{s}}q_{\mathrm{p}}\Bigg\{2q_{\mathrm{s}}(1-p_{\mathrm{c}})p_{\mathrm{c}}\lambda p(\neq 0|\mathrm{c})+(1-p_{\mathrm{c}})\sum_{l=5}^{M_{\max}}p_{\mathrm{c}}^{l-3}\Bigg(\Theta\Big[p(\neq 0|\mathrm{c})-(l-3)p(\neq 0|\mathrm{c})^{l-3}$$
$$+\frac{p(\neq 0|\mathrm{c})-p(\neq 0|\mathrm{c})^{l-3}}{1-p(\neq 0|\mathrm{c})}\Big]+\lambda q_{\mathrm{s}}(l-2)p(\neq 0|\mathrm{c})^{l-3}\Bigg)+p_{\mathrm{c}}^{M_{\max}-2}\Bigg(\Theta\Big[p(\neq 0|\mathrm{c})-(M_{\max}-2)p(\neq 0|\mathrm{c})^{M_{\max}-2}$$
$$+\frac{p(\neq 0|\mathrm{c})-p(\neq 0|\mathrm{c})^{M_{\max}-2}}{1-p(\neq 0|\mathrm{c})}\Big]+(M_{\max}-1)p(\neq 0|\mathrm{c})^{M_{\max}-2}q_{\mathrm{s}}\lambda\Bigg)\Bigg\}=\frac{p_{|0\rangle}q_{\mathrm{p}}q_{\mathrm{s}}}{p(\neq 0|\mathrm{c})^2p_{\mathrm{c}}[1-p(\neq 0|\mathrm{c})p_{\mathrm{c}}]^2}$$
$$\times\Bigg\{2p(\neq 0|\mathrm{c})^3\lambda p_{\mathrm{c}}^2q_{\mathrm{s}}+p(\neq 0|\mathrm{c})^4p_{\mathrm{c}}^4\Bigg(\big[p(\neq 0|\mathrm{c})-1\big]\Theta+\lambda q_{\mathrm{s}}\Bigg)-p(\neq 0|\mathrm{c})^3p_{\mathrm{c}}^3\Bigg(2\big[p(\neq 0|\mathrm{c})-1\big]\Theta$$
$$+\big[2+p(\neq 0|\mathrm{c})\big]\lambda q_{\mathrm{s}}\Bigg)+[p(\neq 0|\mathrm{c})p_{\mathrm{c}}]^{1+M_{\max}}\Bigg(\big[1-p(\neq 0|\mathrm{c})\big]\Theta(M_{\max}-2)+\lambda q_{\mathrm{s}}\Big[2-p(\neq 0|\mathrm{c})$$
$$+\big[p(\neq 0|\mathrm{c})-1\big]M_{\max}\Big]\Bigg)+[p(\neq 0|\mathrm{c})p_{\mathrm{c}}]^{M_{\max}}\Bigg(\Theta-p(\neq 0|\mathrm{c})\Theta-\lambda q_{\mathrm{s}}+\big[p(\neq 0|\mathrm{c})-1\big]M_{\max}\big[\Theta-\lambda q_{\mathrm{s}}\big]\Bigg)\Bigg\},\tag{176}$$

and

$$p_{(\mathrm{b3},2|01)}p_{\mathrm{click}}(\mathrm{D_{M2}}|01,\mathrm{b3},2)=p_{|0\rangle}q_{\mathrm{s}}q_{\mathrm{f}}q_{\mathrm{p}}\gamma\Bigg\{(1-p_{\mathrm{c}})\sum_{l=5}^{M_{\max}}p_{\mathrm{c}}^{l-3}\Big[p(\neq 0|\mathrm{c})-(l-3)p(\neq 0|\mathrm{c})^{l-3}+\frac{p(\neq 0|\mathrm{c})-p(\neq 0|\mathrm{c})^{l-3}}{1-p(\neq 0|\mathrm{c})}\Big]$$
$$+p_{\mathrm{c}}^{M_{\max}-2}\Big[p(\neq 0|\mathrm{c})-(M_{\max}-2)p(\neq 0|\mathrm{c})^{M_{\max}-2}+\frac{p(\neq 0|\mathrm{c})-p(\neq 0|\mathrm{c})^{M_{\max}-2}}{1-p(\neq 0|\mathrm{c})}\Big]\Bigg\}=$$
$$\frac{p_{|0\rangle}q_{\mathrm{s}}q_{\mathrm{f}}q_{\mathrm{p}}\gamma\big[1-p(\neq 0|\mathrm{c})\big]\Big\{[p(\neq 0|\mathrm{c})p_{\mathrm{c}}]^{M_{\max}}\Big[p(\neq 0|\mathrm{c})p_{\mathrm{c}}\,(M_{\max}-2)-M_{\max}+1\Big]+p(\neq 0|\mathrm{c})^3p_{\mathrm{c}}^3\,[2-p(\neq 0|\mathrm{c})p_{\mathrm{c}}]\Big\}}{p(\neq 0|\mathrm{c})^2p_{\mathrm{c}}\big[1-p(\neq 0|\mathrm{c})p_{\mathrm{c}}\big]^2}.\tag{177}$$

Similarly, by using Eqs. (164)-(172)-(174)-(175), and by taking again $M_{\max}\geq M_{\min}+3$, we find that when $M_{\min}>2$ the probability $p_{(\mathrm{b3},2|01)}p_{\mathrm{click}}(\mathrm{D}_{\mathrm{M}i}|01,\mathrm{b3},2)$ is given by

$$p_{(\mathrm{b3},2|01)}p_{\mathrm{click}}(\mathrm{D_{M1}}|01,\mathrm{b3},2)=p_{|0\rangle}q_{\mathrm{s}}q_{\mathrm{p}}\Theta\Bigg\{2(1-p_{\mathrm{c}})p_{\mathrm{c}}^{M_{\min}-1}p(\neq 0|\mathrm{c})\big[1-p(\neq 0|\mathrm{c})\big]$$
$$+(1-p_{\mathrm{c}})\sum_{l=M_{\min}+3}^{M_{\max}}p_{\mathrm{c}}^{l-3}\Big[p(\neq 0|\mathrm{c})-(l-M_{\min})p(\neq 0|\mathrm{c})^{l-M_{\min}}+\frac{p(\neq 0|\mathrm{c})-p(\neq 0|\mathrm{c})^{l-M_{\min}}}{1-p(\neq 0|\mathrm{c})}\Big]$$
$$+p_{\mathrm{c}}^{M_{\max}-2}\Big[p(\neq 0|\mathrm{c})-(M_{\max}-M_{\min}+1)p(\neq 0|\mathrm{c})^{M_{\max}-M_{\min}+1}+\frac{p(\neq 0|\mathrm{c})-p(\neq 0|\mathrm{c})^{M_{\max}-M_{\min}+1}}{1-p(\neq 0|\mathrm{c})}\Big]\Bigg\}$$
$$=\frac{p_{|0\rangle}q_{\mathrm{s}}q_{\mathrm{p}}\Theta\big[1-p(\neq 0|\mathrm{c})\big]p(\neq 0|\mathrm{c})}{p_{\mathrm{c}}[1-p(\neq 0|\mathrm{c})p_{\mathrm{c}}]^2}$$
$$\times\Big(p_{\mathrm{c}}^{M_{\max}}p(\neq 0|\mathrm{c})^{M_{\max}-M_{\min}}\Big[p(\neq 0|\mathrm{c})p_{\mathrm{c}}\,(M_{\max}-M_{\min}+1)-M_{\max}+M_{\min}-2\Big]+\big[2-p(\neq 0|\mathrm{c})p_{\mathrm{c}}\big]p_{\mathrm{c}}^{M_{\min}}\Big),$$
$$p_{(\mathrm{b3},2|01)}p_{\mathrm{click}}(\mathrm{D_{M2}}|01,\mathrm{b3},2)=\frac{q_{\mathrm{f}}\gamma}{\Theta}p_{(\mathrm{b3},2|01)}p_{\mathrm{click}}(\mathrm{D_{M1}}|01,\mathrm{b3},2).\tag{178}$$

*Position 3:* We now consider the scenario where the signals $|\varphi_0\rangle\otimes|\varphi_1\rangle$ emitted by Alice are located in position 3 (see Fig. 12(c)). In a block of the type "b3", this is only possible if its length $l$ satisfies $l\geq 6$, as it is necessary that the number of non-vacuum signals within the block (after Eve's processing) is at least four. Otherwise, the

signals $|\varphi_0\rangle\otimes|\varphi_1\rangle$ cannot be located at position 3 in the processed block prepared by Eve.

We will distinguish between two possibilities, depending on whether the first signal of the block (before Eve's processing) is equal or different to $|\varphi_1\rangle$. To be precise, we will write $p_{(\text{b3},3|01)}p_{\text{click}}(\text{D}_{\text{M}i}|01,\text{b3},3)$ as

$$p_{(\text{b3},3|01)}p_{\text{click}}(\text{D}_{\text{M}i}|01,\text{b3},3)=\sum_{j\in\{|\varphi_1\rangle,\neq|\varphi_1\rangle\}}\sum_{l=\max\{M_{\min}+2,6\}}^{M_{\max}+1}p_{(\text{b3},3,l,j|01)}p_{\text{click}}(\text{D}_{\text{M}i}|01,\text{b3},3,l,j),\tag{179}$$

where $p_{(\text{b3},3,l,|\varphi_1\rangle|01)}$ ($p_{(\text{b3},3,l,\neq|\varphi_1\rangle|01)}$) refers to the conditional probability that the signals $|\varphi_0\rangle\otimes|\varphi_1\rangle$ emitted by Alice correspond to the position 3 of a block of length $l$ of the type "b3" whose first signal is (different from) $|\varphi_1\rangle$, and the probabilities $p_{\text{click}}(\text{D}_{\text{M}i}|01,\text{b3},3,l,j)$ are defined analogously.

We now take into account that when the signals $|\varphi_0\rangle\otimes|\varphi_1\rangle$ emitted by Alice are located in position 3 of a block of signals resent by Eve, there are in total nine possible combinations of signals that Eve can send to Bob (instead of the signals $|\varphi_0\rangle\otimes|\varphi_1\rangle$), each of them happening with probability $r_{(i|0)}r_{(j|1)}$, with $i,j\in\{0,1,2\}$. This means that the probabilities $p_{\text{click}}(\text{D}_{\text{M}i}|01,\text{b3},3,l,j)$ are given by Eq. (117) independently of the value of $l$ and $j$- That is, we have that

$$\begin{aligned}p_{\text{click}}(\text{D}_{\text{M1}}|01,\text{b3},3)&=\frac{(q_{\text{s}}+q_{\text{f}})^2}{p_{\text{c}}^2}\lambda+\frac{2q_{\text{f}}(q_{\text{s}}+q_{\text{f}})}{p_{\text{c}}^2}\gamma=\frac{\xi}{p_{\text{c}}^2},\\ p_{\text{click}}(\text{D}_{\text{M2}}|01,\text{b3},3)&=\frac{2q_{\text{f}}(q_{\text{s}}+q_{\text{f}})}{p_{\text{c}}^2}\gamma.\end{aligned}\tag{180}$$

From Eq. (179) this means that

$$p_{(\text{b3},3|01)}=\sum_{j\in\{|\varphi_1\rangle,\neq|\varphi_1\rangle\}}\sum_{l=\max\{M_{\min}+2,6\}}^{M_{\max}+1}p_{(\text{b3},3,l,j|01)},\tag{181}$$

Next we calculate the probabilities $p_{(\text{b3},3,l,j|01)}$.

We focus first on the probability $p_{(\text{b3},3,l,|\varphi_1\rangle|01)}$, and we start with the case $\max\{M_{\min}+2,6\}\leq l\leq M_{\max}$. Since the block is of the type "b3", this scenario implies that the last non-vacuum signal of the block (*i.e.*, that located at the position $l-1$) is different from $|\varphi_0\rangle$ (otherwise, the block would be of the type "b1"). This situation is illustrated in Fig. 16. There are different possibilities that contribute to $p_{(\text{b3},3,l,|\varphi_1\rangle|01)}$. For example, in the time instance "0" Eve sends Bob a vacuum state, then Eve obtains the result $|\varphi_1\rangle$ (which happens with probability $p_{\text{c}}p(1|\text{c})$), she obtains $l-4$ conclusive results when she measures the following $l-4$ signals including the signals $|\varphi_0\rangle\otimes|\varphi_1\rangle$ emitted by Alice (which happens with probability $p_{\text{c}}^{l-4}$), Eve's measurement result on the next signal is equal to $|\varphi_0\rangle$ (which happens with probability $p_{\text{c}}p(0|\text{c})$), her next measurement result is not equal to $|\varphi_0\rangle$ (which happens with probability $p_{\text{c}}p(\neq 0|\text{c})$), Eve obtains an inconclusive result in the following signal, and with probability $q_{\text{p}}$ Eve decides to process the block. Importantly, note that in this case there are $l-5$ possible positions where the original signals $|\varphi_0\rangle\otimes|\varphi_1\rangle$ can be located. This is illustrated in Fig. 16(a).

Alternatively (if $l\geq\max\{M_{\min}+3,7\}$), Eve can also send Bob a vacuum state in the time instance "0", then Eve obtains the result $|\varphi_1\rangle$, she obtains $l-5$ conclusive results when she measures the following $l-5$ signals including the signals $|\varphi_0\rangle\otimes|\varphi_1\rangle$ emitted by Alice (which happens with probability $p_{\text{c}}^{l-5}$), Eve's measurement result on the next signal is equal to $|\varphi_0\rangle$, her next two measurement results are not equal to $|\varphi_0\rangle$ (which happens with probability $[p_{\text{c}}p(\neq 0|\text{c})]^2$), Eve obtains an inconclusive result in the following signal, and with probability $q_{\text{p}}$ Eve decides to process the block. Importantly, note that in this case there are $l-6$ possible positions where the original signals $|\varphi_0\rangle\otimes|\varphi_1\rangle$ can be located. This is illustrated in Fig. 16(b).

For convenience, let us define the parameter $\kappa$ as

$$\kappa=\max\{M_{\min},4\}.\tag{182}$$

Then, it is easy to show that in total there are $l-\kappa-1$ alternatives like the two described above, being the last one of them that where Eve sends Bob a vacuum state in the time instance "0", then Eve obtains the result $|\varphi_1\rangle$, she obtains $\kappa-2$ conclusive results when she measures the following $\kappa-2$ signals including the signals $|\varphi_0\rangle\otimes|\varphi_1\rangle$ emitted by Alice (which happens with probability $p_{\text{c}}^{\kappa-2}$), Eve's measurement result on the next signal is equal to $|\varphi_0\rangle$, her next $l-\kappa-1$ measurement results are not equal to $|\varphi_0\rangle$ (which happens with probability $[p_{\text{c}}p(\neq 0|\text{c})]^{l-\kappa-1}$), Eve obtains an inconclusive result in the following signal, and with probability $q_{\text{p}}$ Eve decides to process the block. In this case there are $\kappa-3$ possible positions where the original signals $|\varphi_0\rangle\otimes|\varphi_1\rangle$ can be located. This is illustrated in Fig. 16(c).

Putting all together, we find that $p_{(\text{b3},3,l,|\varphi_1\rangle|01)}$, with $\max\{M_{\min}+2,6\}\leq l\leq M_{\max}$, is given by

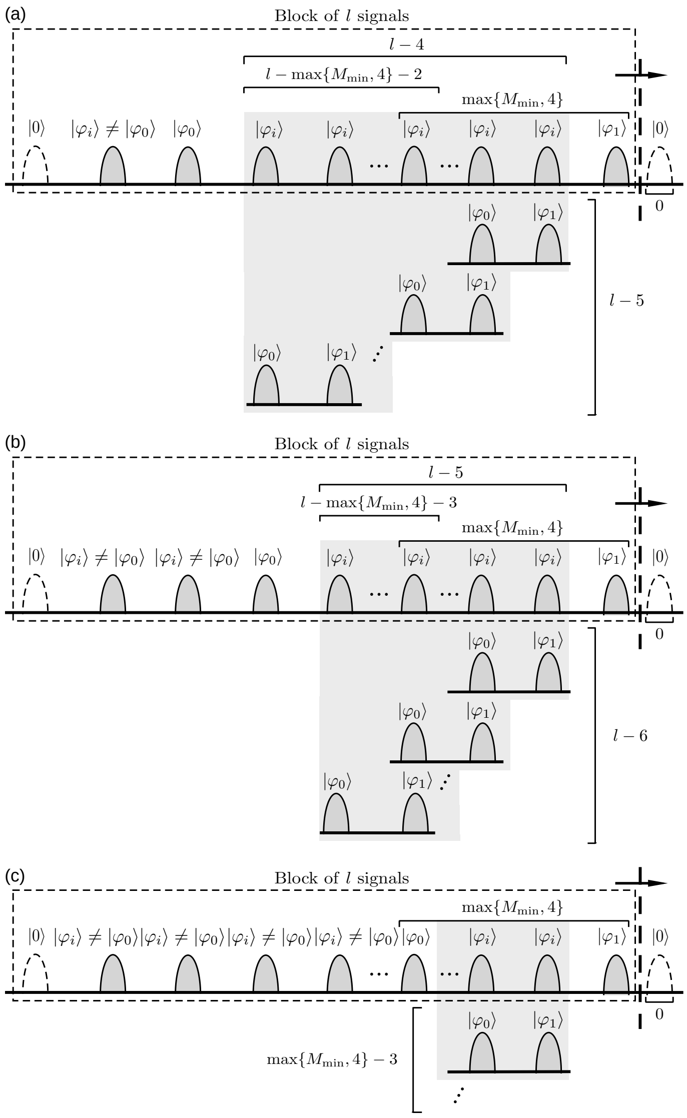


FIG. 16. Illustration of the possible scenarios where the original signals $|\varphi_0\rangle \otimes |\varphi_1\rangle$ emitted by Alice occupy the position 3 in a block of signals of the type "b3" with length $l$ and whose first signal is $|\varphi_1\rangle$. The shadow parts show the time instances where the signals $|\varphi_0\rangle \otimes |\varphi_1\rangle$ can be located with respect to the block.

$$
\begin{aligned}
p_{(\mathrm{b}3,3,l,|\varphi_1\rangle|01)} &= p_{|0\rangle} p(0|\mathrm{c}) p(1|\mathrm{c}) p(\neq 0|\mathrm{c})(1-p_\mathrm{c}) q_\mathrm{p} p_\mathrm{c}^{\kappa+1} \sum_{k=0}^{l-\kappa-2} (l-5-k)[p_\mathrm{c} p(\neq 0|\mathrm{c})]^k p_\mathrm{c}^{l-\kappa-2-k} \\
&= p_{|0\rangle} p(\neq 0|\mathrm{c})(1-p_\mathrm{c}) q_\mathrm{p} p_\mathrm{c}^{l-1} \Big\{ -5 + l[1-p(\neq 0|\mathrm{c})]\big[1-p(\neq 0|\mathrm{c})^{l-\kappa-1}\big] + p(\neq 0|\mathrm{c}) \Big[ 4 + p(\neq 0|\mathrm{c})^{l-\kappa-2} \\
&\times \Big( 4 + l - \kappa - (3+l-\kappa) p(\neq 0|\mathrm{c}) \Big) \Big] \Big\}. \qquad (183)
\end{aligned}
$$

From this result is straightforward to calculate the case with $l = M_{\max}+1$ by simply removing the multiplicative term $1-p_\mathrm{c}$ . We obtain

$$p_{(\mathrm{b3},3,M_{\max}+1,|\varphi_1\rangle|01)} = p_{|0\rangle}p(\neq 0|\mathrm{c})q_{\mathrm{p}}p_{\mathrm{c}}^{M_{\max}}\Big\{-5+(M_{\max}+1)[1-p(\neq 0|\mathrm{c})]\big[1-p(\neq 0|\mathrm{c})^{M_{\max}-\kappa}\big]+p(\neq 0|\mathrm{c})\Big[4 + p(\neq 0|\mathrm{c})^{M_{\max}-\kappa-1}\Big(5+M_{\max}-\kappa-(4+M_{\max}-\kappa)p(\neq 0|\mathrm{c})\Big)\Big]\Big\}. \quad (184)$$

Let us now consider the probability $p_{(\mathrm{b3},3,l,\neq|\varphi_1\rangle|01)}$ with $\max\{M_{\min}+2,6\}\leq l\leq M_{\max}$. The analysis is similar to that of the previous case, and there are also various possibilities that contribute to $p_{(\mathrm{b3},3,l,\neq|\varphi_1\rangle|01)}$. For instance, in the time instance "0" Eve sends Bob a vacuum state, then Eve obtains a conclusive result different from $|\varphi_1\rangle$ (which happens with probability $p_{\mathrm{c}}p(\neq 1|\mathrm{c})$), in the next signal she obtains the result $|\varphi_1\rangle$, she obtains $l-4$ conclusive results when she measures the following $l-4$ signals (including the signals $|\varphi_0\rangle\otimes|\varphi_1\rangle$ emitted by Alice), Eve's measurement result on the next signal (located at position $l-1$) is equal to $|\varphi_0\rangle$, Eve obtains an inconclusive result in the following signal, and with probability $q_{\mathrm{p}}$ Eve decides to process the block. Moreover, in this scenario there are $l-5$ possible positions where the original signals $|\varphi_0\rangle\otimes|\varphi_1\rangle$ can be located. This situation is illustrated in Fig. 17(a).

Similarly, another possibility is that Eve sends Bob a vacuum state in the time instance "0", then Eve obtains a conclusive result different from $|\varphi_1\rangle$, in the next signal she obtains the result $|\varphi_1\rangle$, she obtains $l-5$ conclusive results when she measures the following $l-5$ signals (including the signals $|\varphi_0\rangle\otimes|\varphi_1\rangle$ emitted by Alice), Eve's measurement result on the next signal (located at position $l-2$) is equal to $|\varphi_0\rangle$, Eve obtains a conclusive result different from $|\varphi_0\rangle$ when measuring the signal located at the position $l-1$ of the block, she obtains an inconclusive result in the following signal, and with probability $q_{\mathrm{p}}$ Eve decides to process the block. In this scenario there are $l-6$ possible positions where the original signals $|\varphi_0\rangle\otimes|\varphi_1\rangle$ can be located. They are illustrated in Fig. 17(b).

There are in total $l-\kappa-1$ alternatives like the two described above, being the last one that illustrated in Fig. 17(c). We omit its description here for simplicity and because it is obvious from the text above.

Moreover, we have to consider also those scenarios where Eve obtains several conclusive results different from $|\varphi_1\rangle$ at the beginning of the block (instead of only one as assumed in the cases discussed above) before she obtains the first result equal to $|\varphi_1\rangle$. The analysis is analogous to these above and we also omit it here. Putting all together, it can be shown that

$$\begin{aligned} p_{(\mathrm{b3},3,l,\neq|\varphi_1\rangle|01)} &= p_{|0\rangle}p(0|\mathrm{c})p(1|\mathrm{c})(1-p_{\mathrm{c}})q_{\mathrm{p}}p_{\mathrm{c}}^{l-1}\sum_{t=1}^{l-\kappa-1}p(\neq 1|\mathrm{c})^t\sum_{k=0}^{l-\kappa-1-t}(l-4-t-k)p(\neq 0|\mathrm{c})^k \\ &= \frac{p_{|0\rangle}(1-p_{\mathrm{c}})q_{\mathrm{p}}p_{\mathrm{c}}^{l-1}}{1-p(\neq 0|\mathrm{c})}\Big\{\Big[l(1-p(\neq 0|\mathrm{c}))+3p(\neq 0|\mathrm{c})-5\Big]p(\neq 0|\mathrm{c})-\Big[(l-\kappa)(\kappa-4)+\Big(2(\kappa-3)\kappa \\ &\quad +(7-2\kappa)l-5\Big)p(\neq 0|\mathrm{c})+(l-\kappa-1)(\kappa-3)p(\neq 0|\mathrm{c})^2\Big]p(\neq 0|\mathrm{c})^{l-\kappa}\Big\}, \end{aligned} \quad (185)$$

where in the second equality we have used the fact that $p(\neq 1|\mathrm{c})=p(\neq 0|\mathrm{c})$.

Like above, to calculate $p_{(\mathrm{b3},3,M_{\max}+1,\neq|\varphi_1\rangle|01)}$ we only need to remove from Eq. (185) the term $1-p_{\mathrm{c}}$. We obtain

$$\begin{aligned} p_{(\mathrm{b3},3,M_{\max}+1,\neq|\varphi_1\rangle|01)} &= \frac{p_{|0\rangle}q_{\mathrm{p}}p_{\mathrm{c}}^{M_{\max}}}{1-p(\neq 0|\mathrm{c})}\Big\{\Big[(M_{\max}+1)(1-p(\neq 0|\mathrm{c}))+3p(\neq 0|\mathrm{c})-5\Big]p(\neq 0|\mathrm{c})-\Big[(M_{\max}+1-\kappa) \\ &\quad \times(\kappa-4)+\Big(2(\kappa-3)\kappa+(7-2\kappa)(M_{\max}+1)-5\Big)p(\neq 0|\mathrm{c})+(M_{\max}-\kappa)(\kappa-3)p(\neq 0|\mathrm{c})^2\Big] \\ &\quad \times p(\neq 0|\mathrm{c})^{M_{\max}-\kappa+1}\Big\}. \end{aligned} \quad (186)$$

By combining Eqs. (181)-(183)-(184)-(185)-(186) we find that

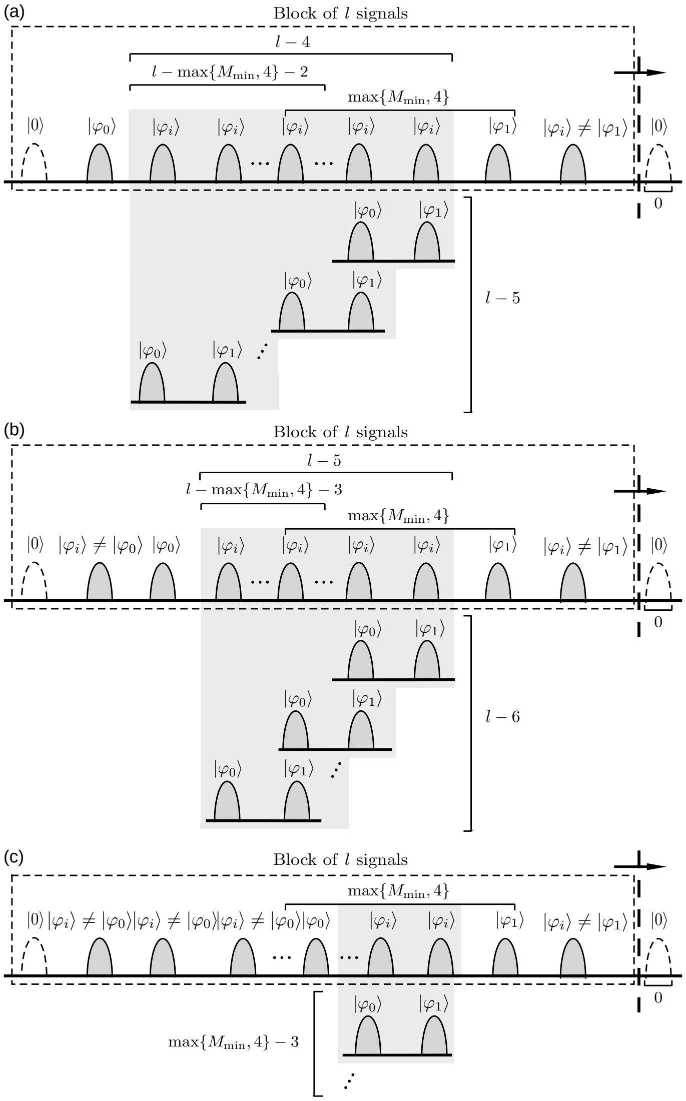


FIG. 17. Illustration of possible scenarios where the original signals $|\varphi_0\rangle\otimes|\varphi_1\rangle$ emitted by Alice occupy the position 3 in a block of signals of the type "b3" with length $l$ and whose first signal is different from $|\varphi_1\rangle$. The shadow parts show the time instances where the signals $|\varphi_0\rangle\otimes|\varphi_1\rangle$ can be located with respect to the block.

$$
\begin{aligned}
p_{(\mathrm{b3},3|01)} = {} & \frac{p_{|0\rangle} q_{\rm p} p_{\rm c}^{M_{\max}}}{1-p(\neq 0|\mathrm{c})}\Bigg\{M_{\max}[2-p(\neq 0|\mathrm{c})][1-p(\neq 0|\mathrm{c})]p(\neq 0|\mathrm{c}) - 8p(\neq 0|\mathrm{c}) + 3[3-p(\neq 0|\mathrm{c})]p(\neq 0|\mathrm{c})^2 + \Bigg[\Bigg(2\kappa \\
& \times (M_{\max}-\kappa+5) - 7M_{\max} - 9\Bigg)p(\neq 0|\mathrm{c}) - (\kappa-4)(M_{\max}-\kappa+2) - (\kappa-3)(M_{\max}-\kappa+1)p(\neq 0|\mathrm{c})^2\Bigg] \\
& \times p(\neq 0|\mathrm{c})^{M_{\max}-\kappa+1}\Bigg\} + \frac{p_{|0\rangle}(1-p_{\rm c})q_{\rm p}}{1-p(\neq 0|\mathrm{c})} \sum_{l=\max\{M_{\min}+2,6\}}^{M_{\max}} p_{\rm c}^{l-1}\Bigg\{\Bigg[l[2-p(\neq 0|\mathrm{c})][1-p(\neq 0|\mathrm{c})] + 4[3-p(\neq 0|\mathrm{c})] \\
& \times p(\neq 0|\mathrm{c}) - 10\Bigg]p(\neq 0|\mathrm{c}) + \Bigg[4 + 4l + \kappa^2[1-p(\neq 0|\mathrm{c})]^2 - 2p(\neq 0|\mathrm{c}) - l[7-3p(\neq 0|\mathrm{c})]p(\neq 0|\mathrm{c}) \\
& - \kappa[1-p(\neq 0|\mathrm{c})]\Bigg(5 + l[1-p(\neq 0|\mathrm{c})] - 3p(\neq 0|\mathrm{c})\Bigg)\Bigg]p(\neq 0|\mathrm{c})^{l-\kappa}\Bigg\}. \qquad (187)
\end{aligned}
$$

Finally, by taking into account Eq. (180) we obtain the probabilities $p_{(\mathrm{b3},3|01)}p_{\rm click}(\mathrm{D}_{\mathrm{M}i}|01,\mathrm{b3},3)$.

*Position 4:* To conclude this part, we now evaluate the situation where the signals $|\varphi_0\rangle\otimes|\varphi_1\rangle$ emitted by Alice are located in position 4.

We start with the case $l=M_{\rm min}+2$ with $M_{\rm min}=2$. This scenario is exactly the same that we have already taken into account when addressing position 2 (see Figs. 14(a) and (b)). So, to avoid counting the same events twice, we set

$$p_{({\rm b3},4,M_{\rm min}+2|01)}=0, \tag{188}$$

if $M_{\rm min}=2$. On the other hand, if $l=M_{\rm min}+2$ with $M_{\rm min}>2$ there are two possibilities. They are illustrated in Figs. 18(a) and (b), and are completely analogous to those of position 2. For simplicity, we omit here their description. By using the fact that $p(\neq 0|{\rm c})=p(\neq 1|{\rm c})$, we obtain that

$$p_{({\rm b3},4,M_{\rm min}+2|01)}=2p_{|0\rangle}q_{\rm s}p_{\rm c}^{M_{\rm min}}p(1|{\rm c})(1-p_{\rm c})q_{\rm p}p(\neq 0|{\rm c}), \tag{189}$$

if $M_{\rm min}>2$. Note that since $p(1|{\rm c})=p(0|{\rm c})$, we have that $p_{({\rm b3},4,M_{\rm min}+2|01)}=p_{({\rm b3},2,M_{\rm min}+2|01)}$.

Also, it is straightforward to show that $p_{\rm click}({\rm D}_{{\rm M}i}|01,{\rm b3},4,M_{\rm min}+2)$ is given by Eq. (106). Putting all together, this means that

$$\begin{aligned}
p_{({\rm b3},2,M_{\rm min}+2|01)}p_{\rm click}({\rm D_{M1}}|01,{\rm b3},2,M_{\rm min}+2)&=\begin{cases}0 & \text{if } M_{\rm min}=2,\\ p_{\rm c}^{M_{\rm min}-1}p(1|{\rm c})\Theta\omega & \text{if } M_{\rm min}>2,\end{cases}\\
p_{({\rm b3},2,M_{\rm min}+2|01)}p_{\rm click}({\rm D_{M2}}|01,{\rm b3},2,M_{\rm min}+2)&=\begin{cases}0 & \text{if } M_{\rm min}=2,\\ q_{\rm f}p_{\rm c}^{M_{\rm min}-1}p(1|{\rm c})\gamma\omega & \text{if } M_{\rm min}>2,\end{cases}
\end{aligned} \tag{190}$$

where the parameters $\Theta$ and $\omega$ are given, respectively, by Eqs. (109)-(165).

Next we evaluate the case $M_{\rm min}+2<l<M_{\rm max}+1$ with $M_{\rm min}=2$. Like in the scenario of position 2, we will consider the time instance that the signal $|\varphi_0\rangle$ (instead of $|\varphi_1\rangle$, used as reference in the case of position 2) occupies with respect to the block, which, in this case, can vary from $l'=l-1$ till $l'=2$.

In particular, let us consider first the situation where $|\varphi_0\rangle$ occupies the time instance $l'=l-1$. This case is completely equivalent to that illustrated in Fig. 14(a) for position 2. One only needs to change in that figure the signal $|\varphi_0\rangle$ with $|\varphi_1\rangle$ (and vice versa) and change the time instances $i$ with $l-i$ (*i.e.*, 0 now becomes $l$, 1 now becomes $l-1$, and so on). In addition, we do not need to consider the case where the first $l-3$ signals of the block provides Eve a conclusive result different from $|\varphi_1\rangle$, as this event has been already taken into account when evaluating the case of position 2. In short, we find that

$$\begin{aligned}
p_{({\rm b3},4,l,l-1|01)}p_{\rm click}({\rm D_{M1}}|01,{\rm b3},4,l,l-1)&=p_{|0\rangle}q_{\rm s}p_{\rm c}^3p(1|{\rm c})p(\neq 1|{\rm c})(1-p_{\rm c})q_{\rm p}\sum_{k=0}^{l-5}[p_{\rm c}p(\neq 1|{\rm c})]^k\,p_{\rm c}^{l-5-k}\left[\frac{q_{\rm s}+q_{\rm f}}{p_{\rm c}}\lambda+\frac{q_{\rm f}}{p_{\rm c}}\gamma\right]\\
&=p_{|0\rangle}q_{\rm s}(1-p_{\rm c})q_{\rm p}p_{\rm c}^{l-3}p(\neq 1|{\rm c})\Theta[1-p(\neq 1|{\rm c})^{l-4}],\\
p_{({\rm b3},4,l,l-1|01)}p_{\rm click}({\rm D_{M2}}|01,{\rm b3},4,l,l-1)&=p_{|0\rangle}q_{\rm s}p_{\rm c}^3p(1|{\rm c})p(\neq 1|{\rm c})(1-p_{\rm c})q_{\rm p}\sum_{k=0}^{l-5}[p_{\rm c}p(\neq 1|{\rm c})]^k\,p_{\rm c}^{l-5-k}\frac{q_{\rm f}}{p_{\rm c}}\gamma\\
&=p_{|0\rangle}q_{\rm s}(1-p_{\rm c})q_{\rm p}p_{\rm c}^{l-3}p(\neq 1|{\rm c})q_{\rm f}\gamma[1-p(\neq 1|{\rm c})^{l-4}].
\end{aligned} \tag{191}$$

If we now consider the case where $|\varphi_0\rangle$ occupies the time instance $l'=l-2$, this is totally equivalent to the case illustrated in Fig. 14(b) for position 2 after making the same changes described above, *i.e.*, change the signals $|\varphi_0\rangle$ with $|\varphi_1\rangle$ (and vice versa) as well as the time instances $i$ with $l-i$. Moreover, like above, we do not need to consider the case where the resulting block (after Eve's processing) contains only two non-vacuum signals, as this event has been already taken into account when evaluating the case of position 2. We find, therefore, that

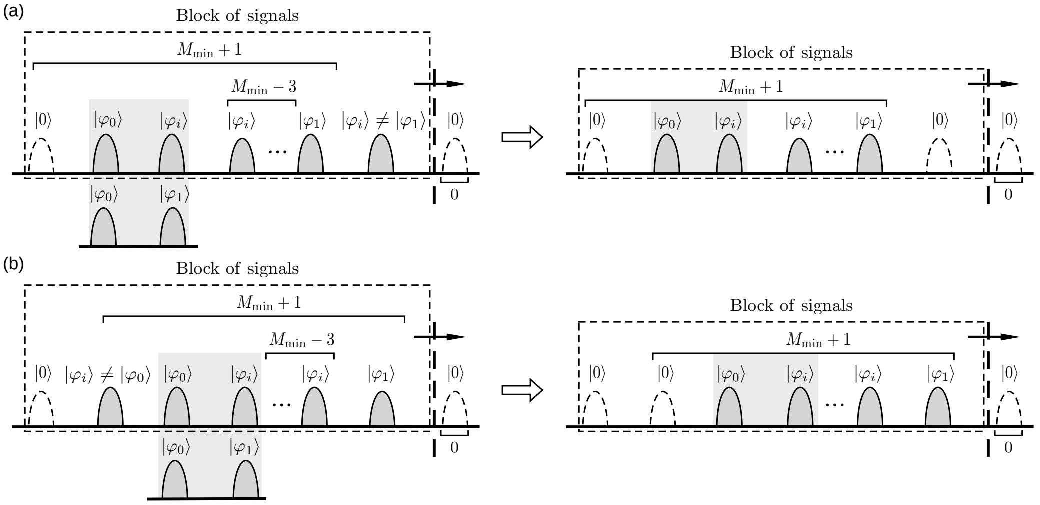


FIG. 18. Illustration of the possible scenarios where the original signals $|\varphi_0\rangle \otimes |\varphi_1\rangle$ emitted by Alice occupy the position 4 in a block of the type "b3" of length $l = M_{\min} + 2$ with $M_{\min} > 2$. On the left hand side of each subfigure we illustrate the measurement results obtained by Eve (including also the vacuum signal in the time instance "0" that precedes the block) together with the location of the original signals emitted by Alice (marked with a shadow area). On the right hand side of each subfigure we illustrate the block of signals that Eve finally sends to Bob.

$$
\begin{aligned}
p_{(\mathrm{b3},4,l,l-2|01)} p_{\mathrm{click}}(\mathrm{D_{M1}}|01,\mathrm{b3},4,l,l-2) &= p_{|0\rangle} q_{\mathrm{s}} p_{\mathrm{c}}^3 p(1|\mathrm{c}) p(\neq 0|\mathrm{c})(1-p_{\mathrm{c}}) q_{\mathrm{p}} \sum_{k=0}^{l-5} [p_{\mathrm{c}} p(\neq 1|\mathrm{c})]^k \, p_{\mathrm{c}}^{l-5-k} \left[\frac{q_{\mathrm{s}}+q_{\mathrm{f}}}{p_{\mathrm{c}}}\lambda + \frac{q_{\mathrm{f}}}{p_{\mathrm{c}}}\gamma\right] \\
&= p_{|0\rangle} q_{\mathrm{s}} (1-p_{\mathrm{c}}) q_{\mathrm{p}} p_{\mathrm{c}}^{l-3} p(\neq 0|\mathrm{c}) \Theta [1 - p(\neq 1|\mathrm{c})^{l-4}], \\
p_{(\mathrm{b3},4,l,l-2|01)} p_{\mathrm{click}}(\mathrm{D_{M2}}|01,\mathrm{b3},4,l,l-2) &= p_{|0\rangle} q_{\mathrm{s}} p_{\mathrm{c}}^3 p(1|\mathrm{c}) p(\neq 0|\mathrm{c})(1-p_{\mathrm{c}}) q_{\mathrm{p}} \sum_{k=0}^{l-5} [p_{\mathrm{c}} p(\neq 1|\mathrm{c})]^k \, p_{\mathrm{c}}^{l-5-k} \frac{q_{\mathrm{f}}}{p_{\mathrm{c}}}\gamma \\
&= p_{|0\rangle} q_{\mathrm{s}} (1-p_{\mathrm{c}}) q_{\mathrm{p}} p_{\mathrm{c}}^{l-3} p(\neq 0|\mathrm{c}) q_{\mathrm{f}} \gamma [1 - p(\neq 1|\mathrm{c})^{l-4}]. \qquad (192)
\end{aligned}
$$

In general, by following the same reasoning like above, it can be shown that for any $l' = 3, \ldots, l-1$, we have that

$$
\begin{aligned}
p_{(\mathrm{b3},4,l,l'|01)} p_{\mathrm{click}}(\mathrm{D_{M1}}|01,\mathrm{b3},4,l,l') &= p_{|0\rangle} q_{\mathrm{s}} (1-p_{\mathrm{c}}) q_{\mathrm{p}} p_{\mathrm{c}}^{l-3} p(\neq 0|\mathrm{c})^{l-l'-1} p(1|\mathrm{c}) \Theta \sum_{k=\max\{0,2-l+l'\}}^{l'-3} p(\neq 1|\mathrm{c})^k, \\
p_{(\mathrm{b3},4,l,l'|01)} p_{\mathrm{click}}(\mathrm{D_{M2}}|01,\mathrm{b3},4,l,l') &= p_{|0\rangle} q_{\mathrm{s}} (1-p_{\mathrm{c}}) q_{\mathrm{p}} p_{\mathrm{c}}^{l-3} p(\neq 0|\mathrm{c})^{l-l'-1} p(1|\mathrm{c}) q_{\mathrm{f}} \gamma \sum_{k=\max\{0,2-l+l'\}}^{l'-3} p(\neq 1|\mathrm{c})^k. \qquad (193)
\end{aligned}
$$

We note that the index $l'$ (which here indicates the position of $|\varphi_0\rangle$) is strictly greater than two because the case $l' = 2$ corresponds to the situation illustrated in the last subfigure of Fig. 14(a), and this case has been already taken into account when we analyzed position 2. Note, however, that in that figure $l'$ refers to the position of the signal $|\varphi_1\rangle$ (instead of the signal $|\varphi_0\rangle$).

We find, therefore, that

$$p_{(\mathrm{b3},4,l|01)}p_{\mathrm{click}}(\mathrm{D_{M1}}|01,\mathrm{b3},4,l) = p_{|0\rangle}q_{\mathrm{s}}(1-p_{\mathrm{c}})q_{\mathrm{p}}p_{\mathrm{c}}^{l-3}p(1|\mathrm{c})\Theta\sum_{l'=3}^{l-1}p(\neq 0|\mathrm{c})^{l-l'-1}\sum_{k=\max\{0,2-l+l'\}}^{l'-3}p(\neq 1|\mathrm{c})^{k}\Bigg\}$$
$$= p_{|0\rangle}q_{\mathrm{s}}(1-p_{\mathrm{c}})q_{\mathrm{p}}p_{\mathrm{c}}^{l-3}\Theta\Bigg[p(\neq 0|\mathrm{c})-(l-3)p(\neq 0|\mathrm{c})^{l-3}+\frac{p(\neq 0|\mathrm{c})-p(\neq 0|\mathrm{c})^{l-3}}{1-p(\neq 0|\mathrm{c})}\Bigg],$$
$$p_{(\mathrm{b3},4,l|01)}p_{\mathrm{click}}(\mathrm{D_{M2}}|01,\mathrm{b3},4,l) = \frac{q_{\mathrm{f}}\gamma}{\Theta}p_{(\mathrm{b3},4,l|01)}p_{\mathrm{click}}(\mathrm{D_{M1}}|01,\mathrm{b3},4,l), \tag{194}$$

when $M_{\min}+2 < l < M_{\max}+1$ and $M_{\min}=2$. Note that in Eq. (194) we have used the fact that $p(\neq 0|\mathrm{c}) = p(\neq 1|\mathrm{c})$. Also, note that, as expected, the probabilities $p_{(\mathrm{b3},4,l|01)}p_{\mathrm{click}}(\mathrm{D}_{\mathrm{M}i}|01,\mathrm{b3},4,l)$, with $i=1,2$, coincide with $p_{(\mathrm{b3},2,l|01)}p_{\mathrm{click}}(\mathrm{D}_{\mathrm{M}i}|01,\mathrm{b3},2,l)$ if we remove from these latter ones the term that multiplies the parameter $\lambda$. This is so because this term corresponds to blocks which (after Eve's processing) only contain two non-vacuum signals, $|\varphi_0\rangle\otimes|\varphi_1\rangle$. Therefore, these events can be interpreted as if Alice's original signals $|\varphi_0\rangle\otimes|\varphi_1\rangle$ are either in position 2 or in position 4 of the processed block, but we have already included them when evaluating position 2, so we do not need to include them again in position 4.

Following the same procedure, it is easy to show that when $M_{\min}+2 < l < M_{\max}+1$ and $M_{\min} > 2$ we have that

$$p_{(\mathrm{b3},4,l|01)}p_{\mathrm{click}}(\mathrm{D_{M1}}|01,\mathrm{b3},4,l) = p_{|0\rangle}q_{\mathrm{s}}(1-p_{\mathrm{c}})q_{\mathrm{p}}p_{\mathrm{c}}^{l-3}p(1|\mathrm{c})\Theta\sum_{l'=M_{\min}}^{l-1}p(\neq 0|\mathrm{c})^{l-l'-1}\sum_{k=\max\{0,2-l+l'\}}^{l'-M_{\min}}p(\neq 1|\mathrm{c})^{k}$$
$$= p_{|0\rangle}q_{\mathrm{s}}(1-p_{\mathrm{c}})q_{\mathrm{p}}p_{\mathrm{c}}^{l-3}\Theta\Bigg\{p(\neq 0|\mathrm{c})-(l-M_{\min})p(\neq 0|\mathrm{c})^{l-M_{\min}}$$
$$+\frac{p(\neq 0|\mathrm{c})-p(\neq 0|\mathrm{c})^{l-M_{\min}}}{1-p(\neq 0|\mathrm{c})}\Bigg\},$$
$$p_{(\mathrm{b3},4,l|01)}p_{\mathrm{click}}(\mathrm{D_{M2}}|01,\mathrm{b3},4,l) = \frac{q_{\mathrm{f}}\gamma}{\Theta}p_{(\mathrm{b3},2,l|01)}p_{\mathrm{click}}(\mathrm{D_{M1}}|01,\mathrm{b3},2,l), \tag{195}$$

where we have used the fact that $p(\neq 0|\mathrm{c}) = p(\neq 1|\mathrm{c})$.

The case $l = M_{\max}+1$ can be obtained directly from the case $M_{\min}+1 < l < M_{\max}+1$ by simply removing the term $1-p_{\mathrm{c}}$ from the probability $p_{(\mathrm{b3},4,l|01)}$. This means that

$$p_{(\mathrm{b3},4,M_{\max}+1|01)}p_{\mathrm{click}}(\mathrm{D_{M1}}|01,\mathrm{b3},4,M_{\max}+1) = p_{|0\rangle}q_{\mathrm{s}}q_{\mathrm{p}}p_{\mathrm{c}}^{M_{\max}-2}\Theta\Bigg[p(\neq 0|\mathrm{c})-(M_{\max}-2)p(\neq 0|\mathrm{c})^{M_{\max}-2}$$
$$+\frac{p(\neq 0|\mathrm{c})-p(\neq 0|\mathrm{c})^{M_{\max}-2}}{1-p(\neq 0|\mathrm{c})}\Bigg],$$
$$p_{(\mathrm{b3},4,M_{\max}+1|01)}p_{\mathrm{click}}(\mathrm{D_{M2}}|01,\mathrm{b3},4,M_{\max}+1) = \frac{q_{\mathrm{f}}\gamma}{\Theta}p_{(\mathrm{b3},4,M_{\max}+1|01)}p_{\mathrm{click}}(\mathrm{D_{M1}}|01,\mathrm{b3},4,M_{\max}+1), \tag{196}$$

when $M_{\min}=2$, and

$$p_{(\mathrm{b3},4,M_{\max}+1|01)}p_{\mathrm{click}}(\mathrm{D_{M1}}|01,\mathrm{b3},4,M_{\max}+1) = p_{|0\rangle}q_{\mathrm{s}}q_{\mathrm{p}}p_{\mathrm{c}}^{M_{\max}-2}\Theta\Bigg\{p(\neq 0|\mathrm{c})-(M_{\max}-M_{\min}+1)$$
$$\times\, p(\neq 0|\mathrm{c})^{M_{\max}-M_{\min}+1}+\frac{p(\neq 0|\mathrm{c})-p(\neq 0|\mathrm{c})^{M_{\max}-M_{\min}+1}}{1-p(\neq 0|\mathrm{c})}\Bigg\},$$
$$p_{(\mathrm{b3},4,M_{\max}+1|01)}p_{\mathrm{click}}(\mathrm{D_{M2}}|01,\mathrm{b3},4,M_{\max}+1) = \frac{q_{\mathrm{f}}\gamma}{\Theta}p_{(\mathrm{b3},4,M_{\max}+1|01)}p_{\mathrm{click}}(\mathrm{D_{M1}}|01,\mathrm{b3},4,M_{\max}+1), \tag{197}$$

when $M_{\min} > 2$.

Finally, by using the fact that

$$p_{(\mathrm{b3},4|01)}p_{\mathrm{click}}(\mathrm{D}_{\mathrm{M}i}|01,\mathrm{b3},4) = \sum_{l=M_{\min}+2}^{M_{\max}+1} p_{(\mathrm{b3},4,l|01)} \times p_{\mathrm{click}}(\mathrm{D}_{\mathrm{M}1}|01,\mathrm{b3},4,l), \quad (198)$$

we obtain that

$$p_{(\mathrm{b3},4|01)}p_{\mathrm{click}}(\mathrm{D}_{\mathrm{M}1}|01,\mathrm{b3},4) = p_{|0\rangle}q_{\mathrm{s}}q_{\mathrm{p}}\Theta\Bigg\{(1-p_{\mathrm{c}})\sum_{l=5}^{M_{\max}}\Bigg[p(\neq 0|\mathrm{c}) - (l-3)p(\neq 0|\mathrm{c})^{l-3} + \frac{p(\neq 0|\mathrm{c}) - p(\neq 0|\mathrm{c})^{l-3}}{1-p(\neq 0|\mathrm{c})}\Bigg]p_{\mathrm{c}}^{l-3} + p_{\mathrm{c}}^{M_{\max}-2}\Bigg[p(\neq 0|\mathrm{c}) - (M_{\max}-2)p(\neq 0|\mathrm{c})^{M_{\max}-2} + \frac{p(\neq 0|\mathrm{c}) - p(\neq 0|\mathrm{c})^{M_{\max}-2}}{1-p(\neq 0|\mathrm{c})}\Bigg]\Bigg\} = \frac{p_{|0\rangle}q_{\mathrm{s}}q_{\mathrm{p}}\Theta\big[1-p(\neq 0|\mathrm{c})\big]}{p(\neq 0|\mathrm{c})^2p_{\mathrm{c}}\big[1-p(\neq 0|\mathrm{c})p_{\mathrm{c}}\big]^2} \times\Bigg\{[p(\neq 0|\mathrm{c})p_{\mathrm{c}}]^{M_{\max}}\Big(p(\neq 0|\mathrm{c})p_{\mathrm{c}}\big[M_{\max}-2\big] - M_{\max}+1\Big) + p(\neq 0|\mathrm{c})^3p_{\mathrm{c}}^3\big[2-p(\neq 0|\mathrm{c})p_{\mathrm{c}}\big]\Bigg\},$$

$$p_{(\mathrm{b3},4|01)}p_{\mathrm{click}}(\mathrm{D}_{\mathrm{M}2}|01,\mathrm{b3},4) = \frac{q_{\mathrm{f}}\gamma}{\Theta}p_{(\mathrm{b3},4|01)}p_{\mathrm{click}}(\mathrm{D}_{\mathrm{M}1}|01,\mathrm{b3},4), \quad (199)$$

if $M_{\min} = 2$ and

$$p_{(\mathrm{b3},4|01)}p_{\mathrm{click}}(\mathrm{D}_{\mathrm{M}1}|01,\mathrm{b3},4) = p_{(\mathrm{b3},2|01)}p_{\mathrm{click}}(\mathrm{D}_{\mathrm{M}1}|01,\mathrm{b3},2),$$
$$p_{(\mathrm{b3},4|01)}p_{\mathrm{click}}(\mathrm{D}_{\mathrm{M}2}|01,\mathrm{b3},4) = \frac{q_{\mathrm{f}}\gamma}{\Theta}p_{(\mathrm{b3},4|01)}p_{\mathrm{click}}(\mathrm{D}_{\mathrm{M}1}|01,\mathrm{b3},4), \quad (200)$$

when $M_{\min} > 2$, where $p_{(\mathrm{b3},2|01)}p_{\mathrm{click}}(\mathrm{D}_{\mathrm{M}1}|01,\mathrm{b3},2)$ is given by Eq. (178).

The visibility $V_{01}$ is given by Eq. (91) with $s = 01$ and the quantities therein are defined by Eq. (98). The summands $p_{(j,k|01)}p_{\mathrm{click}}(\mathrm{D}_{\mathrm{M}i}|01,j,k)$ in Eq. (98), where $i = 1,2$ corresponds to the two different detectors in the monitoring line, $j \in \Omega = \{\mathrm{b1},\mathrm{b2},\mathrm{b3}\}$ refers to the type of block considered and $k = 1,2,3,4,5$ is the position of the sent signals $|\varphi_0\rangle \otimes |\varphi_1\rangle$ in a block of type $j \in \Omega$, are given by Eqs. (99), (100), (113), (123), (133), (143), (151), (153), (155), (157), (159), (176), (177), (178), (187) with (180), (199), (200).

### C. Visibilities $V_{0d}$, $V_{d1}$ and $V_{dd}$

In the remainder of this Section we give the formulas necessary for calculating the visibilities $V_{0d}$, $V_{d1}$ and $V_{dd}$. Since the derivation is very similar to that of $V_{01}$ we only include the final formulas for the quantities $p_{(j,k|s')}p_{\mathrm{click}}(\mathrm{D}_{\mathrm{M}i}|s',j,k)$ with $s' \in \{\text{“}0d\text{”}, \text{“}d1\text{”}, \text{“}dd\text{”}\}$. To obtain the visibilities $V_{0d}$, $V_{d1}$ and $V_{dd}$, one has to combine the $p_{(j,k|s')}p_{\mathrm{click}}(\mathrm{D}_{\mathrm{M}i}|s',j,k)$ quantities in a similar way as it has been done for $V_{01}$ (as in Eq. (98)).

It is easy to see that the quantities $p_{(j,k|s')}p_{\mathrm{click}}(\mathrm{D}_{\mathrm{M}i}|s',j,k)$ for the Positions $k = 1,3,5$ and for all $s' \in \{\text{“}0d\text{”}, \text{“}d1\text{”}, \text{“}dd\text{”}\}$ coincide with the corresponding results for the 01 case, that is, $p_{(\mathrm{b1},1|s')}p_{\mathrm{click}}(\mathrm{D}_{\mathrm{M}i}|s',\mathrm{b1},1)$ is given by Eq. (99), $p_{(\mathrm{b1},5|s')}p_{\mathrm{click}}(\mathrm{D}_{\mathrm{M}i}|s',\mathrm{b1},5)$ is given by Eq. (100), $p_{(\mathrm{b1},3|s')}p_{\mathrm{click}}(\mathrm{D}_{\mathrm{M}i}|s',\mathrm{b1},3)$ is given by Eq. (123), $p_{(\mathrm{b2},1|s')}p_{\mathrm{click}}(\mathrm{D}_{\mathrm{M}i}|s',\mathrm{b2},1)$ is given by Eq. (143), $p_{(\mathrm{b2},3|s')}p_{\mathrm{click}}(\mathrm{D}_{\mathrm{M}i}|s',\mathrm{b2},3)$ is given by Eq. (153), $p_{(\mathrm{b2},5|s')}p_{\mathrm{click}}(\mathrm{D}_{\mathrm{M}i}|s',\mathrm{b2},5)$ is given by Eq. (157), $p_{(\mathrm{b3},1|s')}p_{\mathrm{click}}(\mathrm{D}_{\mathrm{M}i}|s',\mathrm{b3},1)$ is given by Eq. (159), $p_{(\mathrm{b3},5|s')}p_{\mathrm{click}}(\mathrm{D}_{\mathrm{M}i}|s',\mathrm{b3},5)$ is given by Eq. (159) and $p_{(\mathrm{b3},3|s')}p_{\mathrm{click}}(\mathrm{D}_{\mathrm{M}i}|s',\mathrm{b3},3)$ is given by Eq. (187) with Eq. (180) with $i = 1,2$. The remaining quantities can be obtained easily by reusing the corresponding

formulas for the "01" case, one only needs to change the appropriate $q_\mathrm{s}$ quantities to $q_\mathrm{f}$ or vice versa depending on the value of $s'$.

### 1. $V_{0d}$

Thus we obtain the following results for the "$0d$" case:

$$
\begin{aligned}
p_{(\mathrm{b1},2|0d)}p_\mathrm{click}(\mathrm{D_{M1}}|0d,\mathrm{b1},2) &= \begin{cases} p_{|0\rangle}q_\mathrm{f}\Big\{q_\mathrm{s}(1-p_\mathrm{c})q\lambda + p(0|\mathrm{c})p_\mathrm{c}\Theta\Big\} & \text{if } M_\mathrm{min}=2,\\ p_{|0\rangle}q_\mathrm{f}p(0|\mathrm{c})p_\mathrm{c}^{M_\mathrm{min}-2}\big[p_\mathrm{c}+(1-p_\mathrm{c})q\big]\Theta & \text{if } M_\mathrm{min}>2,\end{cases}\\
p_{(\mathrm{b1},2|0d)}p_\mathrm{click}(\mathrm{D_{M2}}|0d,\mathrm{b1},2) &= \begin{cases} p_{|0\rangle}q_\mathrm{f}^2p(0|\mathrm{c})\gamma p_\mathrm{c} & \text{if } M_\mathrm{min}=2,\\ p_{|0\rangle}q_\mathrm{f}^2p(0|\mathrm{c})\gamma p_\mathrm{c}^{M_\mathrm{min}-2}\big[p_\mathrm{c}+(1-p_\mathrm{c})q\big] & \text{if } M_\mathrm{min}>2,\end{cases}
\end{aligned}
\tag{201}
$$

$$
\begin{aligned}
p_{(\mathrm{b1},4|0d)}p_\mathrm{click}(\mathrm{D_{M1}}|0d,\mathrm{b1},4) &= \begin{cases} p_{|0\rangle}q_\mathrm{s}p(1|\mathrm{c})p_\mathrm{c}\Theta & \text{if } M_\mathrm{min}=2,\\ p_{|0\rangle}q_\mathrm{s}p(1|\mathrm{c})p_\mathrm{c}^{M_\mathrm{min}-2}\big[p_\mathrm{c}+(1-p_\mathrm{c})q\big]\Theta & \text{if } M_\mathrm{min}>2,\end{cases}\\
p_{(\mathrm{b1},4|0d)}p_\mathrm{click}(\mathrm{D_{M2}}|0d,\mathrm{b1},4) &= \begin{cases} p_{|0\rangle}q_\mathrm{s}q_\mathrm{f}p(1|\mathrm{c})\gamma p_\mathrm{c} & \text{if } M_\mathrm{min}=2,\\ p_{|0\rangle}q_\mathrm{s}q_\mathrm{f}p(1|\mathrm{c})\gamma p_\mathrm{c}^{M_\mathrm{min}-2}\big[p_\mathrm{c}+(1-p_\mathrm{c})q\big] & \text{if } M_\mathrm{min}>2,\end{cases}
\end{aligned}
\tag{202}
$$

$$
\begin{aligned}
p_{(\mathrm{b2},2|0d)}p_\mathrm{click}(\mathrm{D_{M1}}|0d,\mathrm{b2},2) &= \begin{cases} p_{|0\rangle}(1-q_\mathrm{p})\Big[p_\mathrm{c}\Big(q_\mathrm{f}(q_\mathrm{f}+q_\mathrm{s})\gamma + \big(q_\mathrm{s}+\big[p(1|\mathrm{c})+p(2|\mathrm{c})\big]q_\mathrm{f}\big)\Theta\Big)+ & \\ +(1-p_\mathrm{c})q\Big(2q_\mathrm{f}(q_\mathrm{f}+q_\mathrm{s})\gamma+(q_\mathrm{f}^2+q_\mathrm{f}q_\mathrm{s}+q_\mathrm{s}^2)\lambda\Big)\Big] & \text{if } M_\mathrm{min}=2,\\ p_{|0\rangle}(1-q_\mathrm{p})p_\mathrm{c}^{M_\mathrm{min}-2}\Big[p_\mathrm{c}+(1-p_\mathrm{c})q\Big]\Big[q_\mathrm{f}(q_\mathrm{f}+q_\mathrm{s})\gamma+ & \\ +\Big(q_\mathrm{s}+\big[p(1|\mathrm{c})+p(2|\mathrm{c})\big]q_\mathrm{f}\Big)\Theta\Big] & \text{if } M_\mathrm{min}>2,\end{cases}\\
p_{(\mathrm{b2},2|0d)}p_\mathrm{click}(\mathrm{D_{M2}}|0d,\mathrm{b2},2) &= \begin{cases} p_{|0\rangle}(1-q_\mathrm{p})q_\mathrm{f}\gamma\Big[2p_\mathrm{c}(1-q)q_\mathrm{s}+p_\mathrm{c}\Big(1+p(1|\mathrm{c})+p(2|\mathrm{c})-2q\Big)q_\mathrm{f}+ & \\ +2q(q_\mathrm{f}+q_\mathrm{s})\Big] & \text{if } M_\mathrm{min}=2,\\ p_{|0\rangle}(1-q_\mathrm{p})p_\mathrm{c}^{M_\mathrm{min}-2}q_\mathrm{f}\gamma\Big[p_\mathrm{c}+(1-p_\mathrm{c})q\Big]\Big[2q_\mathrm{s}+ & \\ +\big[1+p(1|\mathrm{c})+p(2|\mathrm{c})\big]q_\mathrm{f}\Big] & \text{if } M_\mathrm{min}>2,\end{cases}
\end{aligned}
\tag{203}
$$

and

$$
\begin{aligned}
p_{(\mathrm{b2},4|0d)}p_\mathrm{click}(\mathrm{D_{M1}}|0d,\mathrm{b2},4) &= \begin{cases} p_{|0\rangle}(1-q_\mathrm{p})p_\mathrm{c}\Big[q_\mathrm{f}(q_\mathrm{f}+q_\mathrm{s})\gamma+\Big(q_\mathrm{f}+\big[1-p(1|\mathrm{c})\big]q_\mathrm{s}\Big)\Theta\Big] & \text{if } M_\mathrm{min}=2,\\ p_{|0\rangle}(1-q_\mathrm{p})p_\mathrm{c}^{M_\mathrm{min}-2}\Big[p_\mathrm{c}+(1-p_\mathrm{c})q\Big]\Big[q_\mathrm{f}(q_\mathrm{f}+q_\mathrm{s})\gamma+ & \\ +\Big(q_\mathrm{f}+\big[1-p(1|\mathrm{c})\big]q_\mathrm{s}\Big)\Theta\Big] & \text{if } M_\mathrm{min}>2,\end{cases}\\
p_{(\mathrm{b2},4|0d)}p_\mathrm{click}(\mathrm{D_{M2}}|0d,\mathrm{b2},4) &= \begin{cases} p_{|0\rangle}(1-q_\mathrm{p})q_\mathrm{f}p_\mathrm{c}\gamma\Big[2q_\mathrm{f}+\Big(2-p(1|\mathrm{c})\Big)q_\mathrm{s}\Big] & \text{if } M_\mathrm{min}=2,\\ p_{|0\rangle}(1-q_\mathrm{p})p_\mathrm{c}^{M_\mathrm{min}-2}q_\mathrm{f}\gamma\Big[p_\mathrm{c}+(1-p_\mathrm{c})q\Big]\Big[2q_\mathrm{f}+\Big(2-p(1|\mathrm{c})\Big)q_\mathrm{s}\Big] & \text{if } M_\mathrm{min}>2.\end{cases}
\end{aligned}
\tag{204}
$$

For type "b3" and Position 2 we have, that

$$p_{(\mathrm{b3},2|0d)}p_{\mathrm{click}}(\mathrm{D_{M1}}|0d,\mathrm{b3},2) = \frac{p_{|0\rangle}q_{\mathrm{p}}q_{\mathrm{f}}}{p(\neq 0|\mathrm{c})^2 p_{\mathrm{c}}[1-p(\neq 0|\mathrm{c})p_{\mathrm{c}}]^2}$$
$$\times\Bigg\{2p(\neq 0|\mathrm{c})^3\lambda p_{\mathrm{c}}^2 q_{\mathrm{s}} + p(\neq 0|\mathrm{c})^4 p_{\mathrm{c}}^4\Big(\big[p(\neq 0|\mathrm{c})-1\big]\Theta+\lambda q_{\mathrm{s}}\Big) - p(\neq 0|\mathrm{c})^3 p_{\mathrm{c}}^3\Big(2\big[p(\neq 0|\mathrm{c})-1\big]\Theta$$
$$+\big[2+p(\neq 0|\mathrm{c})\big]\lambda q_{\mathrm{s}}\Big) + [p(\neq 0|\mathrm{c})p_{\mathrm{c}}]^{1+M_{\max}}\Big(\big[1-p(\neq 0|\mathrm{c})\big]\Theta(M_{\max}-2)+\lambda q_{\mathrm{s}}\Big[2-p(\neq 0|\mathrm{c})$$
$$+\big[p(\neq 0|\mathrm{c})-1\big]M_{\max}\Big]\Big) + [p(\neq 0|\mathrm{c})p_{\mathrm{c}}]^{M_{\max}}\Big(\Theta - p(\neq 0|\mathrm{c})\Theta - \lambda q_{\mathrm{s}} + \big[p(\neq 0|\mathrm{c})-1\big]M_{\max}\big[\Theta-\lambda q_{\mathrm{s}}\big]\Big)\Bigg\}, \tag{205}$$

and

$$p_{(\mathrm{b3},2|0d)}p_{\mathrm{click}}(\mathrm{D_{M2}}|0d,\mathrm{b3},2) =$$
$$\frac{p_{|0\rangle}q_{\mathrm{f}}^2 q_{\mathrm{p}}\gamma\big[1-p(\neq 0|\mathrm{c})\big]\Big\{[p(\neq 0|\mathrm{c})p_{\mathrm{c}}]^{M_{\max}}\Big[p(\neq 0|\mathrm{c})p_{\mathrm{c}}\,(M_{\max}-2)-M_{\max}+1\Big]+p(\neq 0|\mathrm{c})^3 p_{\mathrm{c}}^3\,[2-p(\neq 0|\mathrm{c})p_{\mathrm{c}}]\Big\}}{p(\neq 0|\mathrm{c})^2 p_{\mathrm{c}}\big[1-p(\neq 0|\mathrm{c})p_{\mathrm{c}}\big]^2}, \tag{206}$$

if $M_{\min}=2$ and $M_{\max}\geq 5$. And similarly for the case $M_{\min}>2$ and $M_{\max}\geq M_{\min}+3$:

$$p_{(\mathrm{b3},2|0d)}p_{\mathrm{click}}(\mathrm{D_{M1}}|0d,\mathrm{b3},2) = \frac{p_{|0\rangle}q_{\mathrm{f}}q_{\mathrm{p}}\Theta\big[1-p(\neq 0|\mathrm{c})\big]p(\neq 0|\mathrm{c})}{p_{\mathrm{c}}[1-p(\neq 0|\mathrm{c})p_{\mathrm{c}}]^2}$$
$$\times\Big(p_{\mathrm{c}}^{M_{\max}}p(\neq 0|\mathrm{c})^{M_{\max}-M_{\min}}\Big[p(\neq 0|\mathrm{c})p_{\mathrm{c}}\,(M_{\max}-M_{\min}+1)-M_{\max}+M_{\min}-2\Big]+\big[2-p(\neq 0|\mathrm{c})p_{\mathrm{c}}\big]p_{\mathrm{c}}^{M_{\min}}\Big),$$
$$p_{(\mathrm{b3},2|0d)}p_{\mathrm{click}}(\mathrm{D_{M2}}|0d,\mathrm{b3},2) = \frac{q_{\mathrm{f}}\gamma}{\Theta}p_{(\mathrm{b3},2|0d)}p_{\mathrm{click}}(\mathrm{D_{M1}}|0d,\mathrm{b3},2). \tag{207}$$

And the final case for "0$d$" is type "b3" and Position 4, for which we obtain

$$p_{(\mathrm{b3},4|0d)}p_{\mathrm{click}}(\mathrm{D_{M1}}|0d,\mathrm{b3},4) = \frac{p_{|0\rangle}q_{\mathrm{s}}q_{\mathrm{p}}\Theta\big[1-p(\neq 0|\mathrm{c})\big]}{p(\neq 0|\mathrm{c})^2 p_{\mathrm{c}}\big[1-p(\neq 0|\mathrm{c})p_{\mathrm{c}}\big]^2}$$
$$\times\Bigg\{[p(\neq 0|\mathrm{c})p_{\mathrm{c}}]^{M_{\max}}\Big(p(\neq 0|\mathrm{c})p_{\mathrm{c}}\big[M_{\max}-2\big]-M_{\max}+1\Big)$$
$$+\,p(\neq 0|\mathrm{c})^3 p_{\mathrm{c}}^3\big[2-p(\neq 0|\mathrm{c})p_{\mathrm{c}}\big]\Bigg\},$$
$$p_{(\mathrm{b3},4|0d)}p_{\mathrm{click}}(\mathrm{D_{M2}}|0d,\mathrm{b3},4) = \frac{q_{\mathrm{f}}\gamma}{\Theta}p_{(\mathrm{b3},4|0d)}p_{\mathrm{click}}(\mathrm{D_{M1}}|0d,\mathrm{b3},4), \tag{208}$$

if $M_{\min}=2$ and $M_{\max}\geq 5$, and

$$p_{(\mathrm{b3},4|0d)}p_{\mathrm{click}}(\mathrm{D_{M1}}|0d,\mathrm{b3},4)=p_{(\mathrm{b3},2|01)}p_{\mathrm{click}}(\mathrm{D_{M1}}|01,\mathrm{b3},2),$$
$$p_{(\mathrm{b3},4|0d)}p_{\mathrm{click}}(\mathrm{D_{M2}}|0d,\mathrm{b3},4)=\frac{q_{\mathrm{f}}\gamma}{\Theta}p_{(\mathrm{b3},4|0d)}p_{\mathrm{click}}(\mathrm{D_{M1}}|0d,\mathrm{b3},4), \tag{209}$$

when $M_{\min}>2$ and $M_{\max}\geq M_{\min}+3$, where $p_{(\mathrm{b3},2|01)}p_{\mathrm{click}}(\mathrm{D_{M1}}|01,\mathrm{b3},2)$ is given by Eq. (178).

### 2. $V_{d1}$

The formulas for the "$d1$" case are the following:

$$p_{(\mathrm{b1},2|d1)}p_{\mathrm{click}}(\mathrm{D_{M1}}|d1,\mathrm{b1},2)=\begin{cases}p_{|0\rangle}q_{\mathrm{s}}\Big\{q_{\mathrm{f}}(1-p_{\mathrm{c}})q\lambda+p(0|\mathrm{c})p_{\mathrm{c}}\Theta\Big\} & \text{if } M_{\min}=2,\\ p_{|0\rangle}q_{\mathrm{s}}p(0|\mathrm{c})p_{\mathrm{c}}^{M_{\min}-2}\big[p_{\mathrm{c}}+(1-p_{\mathrm{c}})q\big]\Theta & \text{if } M_{\min}>2,\end{cases}$$
$$p_{(\mathrm{b1},2|d1)}p_{\mathrm{click}}(\mathrm{D_{M2}}|d1,\mathrm{b1},2)=\begin{cases}p_{|0\rangle}q_{\mathrm{s}}q_{\mathrm{f}}p(0|\mathrm{c})\gamma p_{\mathrm{c}} & \text{if } M_{\min}=2,\\ p_{|0\rangle}q_{\mathrm{s}}q_{\mathrm{f}}p(0|\mathrm{c})\gamma p_{\mathrm{c}}^{M_{\min}-2}\big[p_{\mathrm{c}}+(1-p_{\mathrm{c}})q\big] & \text{if } M_{\min}>2,\end{cases} \tag{210}$$

$$p_{(\mathrm{b1},4|d1)}p_{\mathrm{click}}(\mathrm{D_{M1}}|d1,\mathrm{b1},4)=\begin{cases}p_{|0\rangle}q_{\mathrm{f}}p(1|\mathrm{c})p_{\mathrm{c}}\Theta & \text{if } M_{\min}=2,\\ p_{|0\rangle}q_{\mathrm{f}}p(1|\mathrm{c})p_{\mathrm{c}}^{M_{\min}-2}\big[p_{\mathrm{c}}+(1-p_{\mathrm{c}})q\big]\Theta & \text{if } M_{\min}>2,\end{cases}$$
$$p_{(\mathrm{b1},4|d1)}p_{\mathrm{click}}(\mathrm{D_{M2}}|d1,\mathrm{b1},4)=\begin{cases}p_{|0\rangle}q_{\mathrm{f}}^2p(1|\mathrm{c})\gamma p_{\mathrm{c}} & \text{if } M_{\min}=2,\\ p_{|0\rangle}q_{\mathrm{f}}^2p(1|\mathrm{c})\gamma p_{\mathrm{c}}^{M_{\min}-2}\big[p_{\mathrm{c}}+(1-p_{\mathrm{c}})q\big] & \text{if } M_{\min}>2,\end{cases} \tag{211}$$

$$p_{(\mathrm{b2},2|d1)}p_{\mathrm{click}}(\mathrm{D_{M1}}|d1,\mathrm{b2},2)=\begin{cases}p_{|0\rangle}(1-q_{\mathrm{p}})\Big[p_{\mathrm{c}}\Big(q_{\mathrm{f}}(q_{\mathrm{f}}+q_{\mathrm{s}})\gamma+\big(q_{\mathrm{f}}+\big[p(1|\mathrm{c})+p(2|\mathrm{c})\big]q_{\mathrm{s}}\big)\Theta\Big)+ & \\ +(1-p_{\mathrm{c}})q\Big(2q_{\mathrm{f}}(q_{\mathrm{f}}+q_{\mathrm{s}})\gamma+(q_{\mathrm{f}}^2+q_{\mathrm{f}}q_{\mathrm{s}}+q_{\mathrm{s}}^2)\lambda\Big)\Big] & \text{if } M_{\min}=2,\\ p_{|0\rangle}(1-q_{\mathrm{p}})p_{\mathrm{c}}^{M_{\min}-2}\Big[p_{\mathrm{c}}+(1-p_{\mathrm{c}})q\Big]\Big[q_{\mathrm{f}}(q_{\mathrm{f}}+q_{\mathrm{s}})\gamma+ & \\ +\Big(q_{\mathrm{f}}+\big[p(1|\mathrm{c})+p(2|\mathrm{c})\big]q_{\mathrm{s}}\Big)\Theta\Big] & \text{if } M_{\min}>2,\end{cases}$$
$$p_{(\mathrm{b2},2|d1)}p_{\mathrm{click}}(\mathrm{D_{M2}}|d1,\mathrm{b2},2)=\begin{cases}p_{|0\rangle}(1-q_{\mathrm{p}})q_{\mathrm{f}}\gamma\Big[2p_{\mathrm{c}}(1-q)q_{\mathrm{f}}+p_{\mathrm{c}}\Big(1+p(1|\mathrm{c})+p(2|\mathrm{c})-2q\Big)q_{\mathrm{s}}+ & \\ +2q(q_{\mathrm{f}}+q_{\mathrm{s}})\Big] & \text{if } M_{\min}=2,\\ p_{|0\rangle}(1-q_{\mathrm{p}})p_{\mathrm{c}}^{M_{\min}-2}q_{\mathrm{f}}\gamma\Big[p_{\mathrm{c}}+(1-p_{\mathrm{c}})q\Big]\Big[2q_{\mathrm{f}}+ & \\ +\big[1+p(1|\mathrm{c})+p(2|\mathrm{c})\big]q_{\mathrm{s}}\Big] & \text{if } M_{\min}>2,\end{cases} \tag{212}$$

and

$$p_{(\mathrm{b2},4|d1)}p_{\mathrm{click}}(\mathrm{D_{M1}}|d1,\mathrm{b2},4)=\begin{cases}p_{|0\rangle}(1-q_{\mathrm{p}})p_{\mathrm{c}}\Big[q_{\mathrm{f}}(q_{\mathrm{f}}+q_{\mathrm{s}})\gamma+\Big(q_{\mathrm{s}}+\big[1-p(1|\mathrm{c})\big]q_{\mathrm{f}}\Big)\Theta\Big] & \text{if } M_{\min}=2,\\ p_{|0\rangle}(1-q_{\mathrm{p}})p_{\mathrm{c}}^{M_{\min}-2}\Big[p_{\mathrm{c}}+(1-p_{\mathrm{c}})q\Big]\Big[q_{\mathrm{f}}(q_{\mathrm{f}}+q_{\mathrm{s}})\gamma+ & \\ +\Big(q_{\mathrm{s}}+\big[1-p(1|\mathrm{c})\big]q_{\mathrm{f}}\Big)\Theta\Big] & \text{if } M_{\min}>2,\end{cases}$$

$$p_{(\mathrm{b2},4|d1)}p_{\mathrm{click}}(\mathrm{D_{M2}}|d1,\mathrm{b2},4)=\begin{cases}p_{|0\rangle}(1-q_{\mathrm{p}})q_{\mathrm{f}}p_{\mathrm{c}}\gamma\Big[2q_{\mathrm{s}}+\Big(2-p(1|\mathrm{c})\Big)q_{\mathrm{f}}\Big] & \text{if } M_{\min}=2,\\ p_{|0\rangle}(1-q_{\mathrm{p}})p_{\mathrm{c}}^{M_{\min}-2}q_{\mathrm{f}}\gamma\Big[p_{\mathrm{c}}+(1-p_{\mathrm{c}})q\Big]\Big[2q_{\mathrm{s}}+\Big(2-p(1|\mathrm{c})\Big)q_{\mathrm{f}}\Big] & \text{if } M_{\min}>2.\end{cases} \tag{213}$$

For type "b3" and Position 2 we have, that

$$\begin{aligned}p_{(\mathrm{b3},2|d1)}p_{\mathrm{click}}(\mathrm{D_{M1}}|d1,\mathrm{b3},2)=&\frac{p_{|0\rangle}q_{\mathrm{p}}q_{\mathrm{s}}}{p(\neq 0|\mathrm{c})^2p_{\mathrm{c}}[1-p(\neq 0|\mathrm{c})p_{\mathrm{c}}]^2}\\ \times\Bigg\{&2p(\neq 0|\mathrm{c})^3\lambda p_{\mathrm{c}}^2q_{\mathrm{f}}+p(\neq 0|\mathrm{c})^4p_{\mathrm{c}}^4\Bigg(\big[p(\neq 0|\mathrm{c})-1\big]\Theta+\lambda q_{\mathrm{f}}\Bigg)-p(\neq 0|\mathrm{c})^3p_{\mathrm{c}}^3\Bigg(2\big[p(\neq 0|\mathrm{c})-1\big]\Theta\\ &+\big[2+p(\neq 0|\mathrm{c})\big]\lambda q_{\mathrm{f}}\Bigg)+[p(\neq 0|\mathrm{c})p_{\mathrm{c}}]^{1+M_{\max}}\Bigg(\big[1-p(\neq 0|\mathrm{c})\big]\Theta(M_{\max}-2)+\lambda q_{\mathrm{f}}\Big[2-p(\neq 0|\mathrm{c})\\ &+\big[p(\neq 0|\mathrm{c})-1\big]M_{\max}\Big]\Bigg)+[p(\neq 0|\mathrm{c})p_{\mathrm{c}}]^{M_{\max}}\Bigg(\Theta-p(\neq 0|\mathrm{c})\Theta-\lambda q_{\mathrm{f}}+\big[p(\neq 0|\mathrm{c})-1\big]M_{\max}\big[\Theta-\lambda q_{\mathrm{f}}\big]\Bigg)\Bigg\},\end{aligned} \tag{214}$$

and

$$p_{(\mathrm{b3},2|d1)}p_{\mathrm{click}}(\mathrm{D_{M2}}|d1,\mathrm{b3},2)=\frac{p_{|0\rangle}q_{\mathrm{f}}q_{\mathrm{s}}q_{\mathrm{p}}\gamma\big[1-p(\neq 0|\mathrm{c})\big]\Big\{[p(\neq 0|\mathrm{c})p_{\mathrm{c}}]^{M_{\max}}\Big[p(\neq 0|\mathrm{c})p_{\mathrm{c}}\left(M_{\max}-2\right)-M_{\max}+1\Big]+p(\neq 0|\mathrm{c})^3p_{\mathrm{c}}^3\left[2-p(\neq 0|\mathrm{c})p_{\mathrm{c}}\right]\Big\}}{p(\neq 0|\mathrm{c})^2p_{\mathrm{c}}\big[1-p(\neq 0|\mathrm{c})p_{\mathrm{c}}\big]^2}, \tag{215}$$

if $M_{\min}=2$ and $M_{\max}\geq 5$. And similarly for the case $M_{\min}>2$ and $M_{\max}\geq M_{\min}+3$:

$$\begin{aligned}p_{(\mathrm{b3},2|d1)}p_{\mathrm{click}}(\mathrm{D_{M1}}|d1,\mathrm{b3},2)=&\frac{p_{|0\rangle}q_{\mathrm{s}}q_{\mathrm{p}}\Theta\big[1-p(\neq 0|\mathrm{c})\big]p(\neq 0|\mathrm{c})}{p_{\mathrm{c}}[1-p(\neq 0|\mathrm{c})p_{\mathrm{c}}]^2}\\ \times\Big(&p_{\mathrm{c}}^{M_{\max}}p(\neq 0|\mathrm{c})^{M_{\max}-M_{\min}}\Big[p(\neq 0|\mathrm{c})p_{\mathrm{c}}\left(M_{\max}-M_{\min}+1\right)-M_{\max}+M_{\min}-2\Big]+\big[2-p(\neq 0|\mathrm{c})p_{\mathrm{c}}\big]p_{\mathrm{c}}^{M_{\min}}\Big),\\ p_{(\mathrm{b3},2|d1)}p_{\mathrm{click}}(\mathrm{D_{M2}}|d1,\mathrm{b3},2)=&\frac{q_{\mathrm{f}}\gamma}{\Theta}p_{(\mathrm{b3},2|d1)}p_{\mathrm{click}}(\mathrm{D_{M1}}|d1,\mathrm{b3},2).\end{aligned} \tag{216}$$

And the final case for "$d1$" is type "b3" and Position 4, for which we obtain

$$p_{(\mathrm{b3},4|d1)}p_{\mathrm{click}}(\mathrm{D_{M1}}|d1,\mathrm{b3},4)=\frac{p_{|0\rangle}q_{\mathrm{f}}q_{\mathrm{p}}\Theta\big[1-p(\neq 0|\mathrm{c})\big]}{p(\neq 0|\mathrm{c})^2p_{\mathrm{c}}\big[1-p(\neq 0|\mathrm{c})p_{\mathrm{c}}\big]^2}\times\Bigg\{[p(\neq 0|\mathrm{c})p_{\mathrm{c}}]^{M_{\max}}\Big(p(\neq 0|\mathrm{c})p_{\mathrm{c}}\big[M_{\max}-2\big]-M_{\max}+1\Big)+p(\neq 0|\mathrm{c})^3p_{\mathrm{c}}^3\big[2-p(\neq 0|\mathrm{c})p_{\mathrm{c}}\big]\Bigg\},$$
$$p_{(\mathrm{b3},4|d1)}p_{\mathrm{click}}(\mathrm{D_{M2}}|d1,\mathrm{b3},4)=\frac{q_{\mathrm{f}}\gamma}{\Theta}p_{(\mathrm{b3},4|d1)}p_{\mathrm{click}}(\mathrm{D_{M1}}|d1,\mathrm{b3},4),\tag{217}$$

if $M_{\min}=2$ and $M_{\max}\geq 5$ and

$$p_{(\mathrm{b3},4|d1)}p_{\mathrm{click}}(\mathrm{D_{M1}}|d1,\mathrm{b3},4)=\frac{p_{|0\rangle}q_{\mathrm{f}}q_{\mathrm{p}}\Theta\big[1-p(\neq 0|\mathrm{c})\big]p(\neq 0|\mathrm{c})}{p_{\mathrm{c}}[1-p(\neq 0|\mathrm{c})p_{\mathrm{c}}]^2}\times\Big(p_{\mathrm{c}}^{M_{\max}}p(\neq 0|\mathrm{c})^{M_{\max}-M_{\min}}\Big[p(\neq 0|\mathrm{c})p_{\mathrm{c}}\left(M_{\max}-M_{\min}+1\right)-M_{\max}+M_{\min}-2\Big]+\big[2-p(\neq 0|\mathrm{c})p_{\mathrm{c}}\big]p_{\mathrm{c}}^{M_{\min}}\Big),$$
$$p_{(\mathrm{b3},4|d1)}p_{\mathrm{click}}(\mathrm{D_{M2}}|d1,\mathrm{b3},4)=\frac{q_{\mathrm{f}}\gamma}{\Theta}p_{(\mathrm{b3},4|d1)}p_{\mathrm{click}}(\mathrm{D_{M1}}|d1,\mathrm{b3},4),\tag{218}$$

when $M_{\min}>2$ and $M_{\max}\geq M_{\min}+3$.

### 3. $V_{dd}$

The results for the "*dd*" case are as follows:

$$p_{(\mathrm{b1},2|dd)}p_{\mathrm{click}}(\mathrm{D_{M1}}|dd,\mathrm{b1},2)=\begin{cases}p_{|0\rangle}q_{\mathrm{f}}\Big\{q_{\mathrm{f}}(1-p_{\mathrm{c}})q\lambda+p(0|\mathrm{c})p_{\mathrm{c}}\Theta\Big\} & \text{if } M_{\min}=2,\\ p_{|0\rangle}q_{\mathrm{f}}p(0|\mathrm{c})p_{\mathrm{c}}^{M_{\min}-2}\big[p_{\mathrm{c}}+(1-p_{\mathrm{c}})q\big]\Theta & \text{if } M_{\min}>2,\end{cases}$$
$$p_{(\mathrm{b1},2|dd)}p_{\mathrm{click}}(\mathrm{D_{M2}}|dd,\mathrm{b1},2)=\begin{cases}p_{|0\rangle}q_{\mathrm{f}}^2p(0|\mathrm{c})\gamma p_{\mathrm{c}} & \text{if } M_{\min}=2,\\ p_{|0\rangle}q_{\mathrm{f}}^2p(0|\mathrm{c})\gamma p_{\mathrm{c}}^{M_{\min}-2}\big[p_{\mathrm{c}}+(1-p_{\mathrm{c}})q\big] & \text{if } M_{\min}>2.\end{cases}\tag{219}$$

$$p_{(\mathrm{b1},4|dd)}p_{\mathrm{click}}(\mathrm{D_{M1}}|dd,\mathrm{b1},4)=\begin{cases}p_{|0\rangle}q_{\mathrm{f}}p(1|\mathrm{c})p_{\mathrm{c}}\Theta & \text{if } M_{\min}=2,\\ p_{|0\rangle}q_{\mathrm{f}}p(1|\mathrm{c})p_{\mathrm{c}}^{M_{\min}-2}\big[p_{\mathrm{c}}+(1-p_{\mathrm{c}})q\big]\Theta & \text{if } M_{\min}>2,\end{cases}$$
$$p_{(\mathrm{b1},4|dd)}p_{\mathrm{click}}(\mathrm{D_{M2}}|dd,\mathrm{b1},4)=\begin{cases}p_{|0\rangle}q_{\mathrm{f}}^2p(1|\mathrm{c})\gamma p_{\mathrm{c}} & \text{if } M_{\min}=2,\\ p_{|0\rangle}q_{\mathrm{f}}^2p(1|\mathrm{c})\gamma p_{\mathrm{c}}^{M_{\min}-2}\big[p_{\mathrm{c}}+(1-p_{\mathrm{c}})q\big] & \text{if } M_{\min}>2,\end{cases}\tag{220}$$

$$p_{(\mathrm{b2},2|dd)}p_{\mathrm{click}}(\mathrm{D_{M1}}|dd,\mathrm{b2},2)=\begin{cases} p_{|0\rangle}(1-q_{\mathrm{p}})\Big[p_{\mathrm{c}}\Big(q_{\mathrm{f}}(q_{\mathrm{f}}+q_{\mathrm{s}})\gamma+\big(q_{\mathrm{s}}+\big[p(1|\mathrm{c})+p(2|\mathrm{c})\big]q_{\mathrm{f}}\big)\Theta\Big)+ \\ +(1-p_{\mathrm{c}})q\Big(2q_{\mathrm{f}}(q_{\mathrm{f}}+q_{\mathrm{s}})\gamma+p_{\mathrm{c}}q_{\mathrm{s}}\lambda\Big)\Big] & \text{if } M_{\min}=2, \\ p_{|0\rangle}(1-q_{\mathrm{p}})p_{\mathrm{c}}^{M_{\min}-2}\Big[p_{\mathrm{c}}+(1-p_{\mathrm{c}})q\Big]\Big[q_{\mathrm{f}}(q_{\mathrm{f}}+q_{\mathrm{s}})\gamma+ \\ +\Big(q_{\mathrm{s}}+\big[p(1|\mathrm{c})+p(2|\mathrm{c})\big]q_{\mathrm{f}}\Big)\Theta\Big] & \text{if } M_{\min}>2, \end{cases}$$

$$p_{(\mathrm{b2},2|dd)}p_{\mathrm{click}}(\mathrm{D_{M2}}|dd,\mathrm{b2},2)=\begin{cases} p_{|0\rangle}(1-q_{\mathrm{p}})q_{\mathrm{f}}\gamma\Big[2p_{\mathrm{c}}(1-q)q_{\mathrm{s}}+p_{\mathrm{c}}\Big(1+p(1|\mathrm{c})+p(2|\mathrm{c})-2q\Big)q_{\mathrm{f}}+ \\ +2q(q_{\mathrm{f}}+q_{\mathrm{s}})\Big] & \text{if } M_{\min}=2, \\ p_{|0\rangle}(1-q_{\mathrm{p}})p_{\mathrm{c}}^{M_{\min}-2}q_{\mathrm{f}}\gamma\Big[p_{\mathrm{c}}+(1-p_{\mathrm{c}})q\Big]\Big[2q_{\mathrm{s}}+ \\ +\big[1+p(1|\mathrm{c})+p(2|\mathrm{c})\big]q_{\mathrm{f}}\Big] & \text{if } M_{\min}>2, \end{cases} \tag{221}$$

and for Position 4 one obtains:

$$p_{(\mathrm{b2},4|dd)}p_{\mathrm{click}}(\mathrm{D_{M1}}|dd,\mathrm{b2},4)=\begin{cases} p_{|0\rangle}(1-q_{\mathrm{p}})p_{\mathrm{c}}\Big[q_{\mathrm{f}}(q_{\mathrm{f}}+q_{\mathrm{s}})\gamma+\Big(q_{\mathrm{s}}+\big[1-p(1|\mathrm{c})\big]q_{\mathrm{f}}\Big)\Theta\Big] & \text{if } M_{\min}=2, \\ p_{|0\rangle}(1-q_{\mathrm{p}})p_{\mathrm{c}}^{M_{\min}-2}\Big[p_{\mathrm{c}}+(1-p_{\mathrm{c}})q\Big]\Big[q_{\mathrm{f}}(q_{\mathrm{f}}+q_{\mathrm{s}})\gamma+ \\ +\Big(q_{\mathrm{s}}+\big[1-p(1|\mathrm{c})\big]q_{\mathrm{f}}\Big)\Theta\Big] & \text{if } M_{\min}>2, \end{cases}$$

$$p_{(\mathrm{b2},4|dd)}p_{\mathrm{click}}(\mathrm{D_{M2}}|dd,\mathrm{b2},4)=\begin{cases} p_{|0\rangle}(1-q_{\mathrm{p}})q_{\mathrm{f}}p_{\mathrm{c}}\gamma\Big[2q_{\mathrm{s}}+\Big(2-p(1|\mathrm{c})\Big)q_{\mathrm{f}}\Big] & \text{if } M_{\min}=2, \\ p_{|0\rangle}(1-q_{\mathrm{p}})p_{\mathrm{c}}^{M_{\min}-2}q_{\mathrm{f}}\gamma\Big[p_{\mathrm{c}}+(1-p_{\mathrm{c}})q\Big]\Big[2q_{\mathrm{s}}+\Big(2-p(1|\mathrm{c})\Big)q_{\mathrm{f}}\Big] & \text{if } M_{\min}>2. \end{cases} \tag{222}$$

For type "b3" and Position 2 we have, that

$$\begin{aligned} p_{(\mathrm{b3},2|dd)}p_{\mathrm{click}}(\mathrm{D_{M1}}|dd,\mathrm{b3},2) &= \frac{p_{|0\rangle}q_{\mathrm{p}}q_{\mathrm{f}}}{p(\neq 0|\mathrm{c})^2p_{\mathrm{c}}[1-p(\neq 0|\mathrm{c})p_{\mathrm{c}}]^2} \\ &\times\Bigg\{2p(\neq 0|\mathrm{c})^3\lambda p_{\mathrm{c}}^2q_{\mathrm{f}}+p(\neq 0|\mathrm{c})^4p_{\mathrm{c}}^4\Bigg(\big[p(\neq 0|\mathrm{c})-1\big]\Theta+\lambda q_{\mathrm{f}}\Bigg)-p(\neq 0|\mathrm{c})^3p_{\mathrm{c}}^3\Bigg(2\big[p(\neq 0|\mathrm{c})-1\big]\Theta \\ &+\big[2+p(\neq 0|\mathrm{c})\big]\lambda q_{\mathrm{f}}\Bigg)+[p(\neq 0|\mathrm{c})p_{\mathrm{c}}]^{1+M_{\max}}\Bigg(\big[1-p(\neq 0|\mathrm{c})\big]\Theta(M_{\max}-2)+\lambda q_{\mathrm{f}}\Big[2-p(\neq 0|\mathrm{c}) \\ &+\big[p(\neq 0|\mathrm{c})-1\big]M_{\max}\Big]\Bigg)+[p(\neq 0|\mathrm{c})p_{\mathrm{c}}]^{M_{\max}}\Bigg(\Theta-p(\neq 0|\mathrm{c})\Theta-\lambda q_{\mathrm{f}}+\big[p(\neq 0|\mathrm{c})-1\big]M_{\max}\big[\Theta-\lambda q_{\mathrm{f}}\big]\Bigg)\Bigg\}, \end{aligned} \tag{223}$$

and

$$\begin{aligned} &p_{(\mathrm{b3},2|dd)}p_{\mathrm{click}}(\mathrm{D_{M2}}|dd,\mathrm{b3},2)= \\ &\frac{p_{|0\rangle}q_{\mathrm{f}}^2q_{\mathrm{p}}\gamma\big[1-p(\neq 0|\mathrm{c})\big]\Big\{[p(\neq 0|\mathrm{c})p_{\mathrm{c}}]^{M_{\max}}\Big[p(\neq 0|\mathrm{c})p_{\mathrm{c}}\,(M_{\max}-2)-M_{\max}+1\Big]+p(\neq 0|\mathrm{c})^3p_{\mathrm{c}}^3\,[2-p(\neq 0|\mathrm{c})p_{\mathrm{c}}]\Big\}}{p(\neq 0|\mathrm{c})^2p_{\mathrm{c}}\big[1-p(\neq 0|\mathrm{c})p_{\mathrm{c}}\big]^2}, \end{aligned} \tag{224}$$

if $M_{\min}=2$ and $M_{\max}\geq 5$. And similarly for the case $M_{\min}>2$ and $M_{\max}\geq M_{\min}+3$:

$$
\begin{aligned}
p_{(\mathrm{b3},2|dd)}p_{\mathrm{click}}(\mathrm{D_{M1}}|dd,\mathrm{b3},2) &= \frac{p_{|0\rangle}q_{\mathrm{f}}q_{\mathrm{p}}\Theta\big[1-p(\neq 0|\mathrm{c})\big]p(\neq 0|\mathrm{c})}{p_{\mathrm{c}}[1-p(\neq 0|\mathrm{c})p_{\mathrm{c}}]^2} \\
&\times\Big(p_{\mathrm{c}}^{M_{\max}}p(\neq 0|\mathrm{c})^{M_{\max}-M_{\min}}\Big[p(\neq 0|\mathrm{c})p_{\mathrm{c}}\,(M_{\max}-M_{\min}+1)-M_{\max}+M_{\min}-2\Big]+\big[2-p(\neq 0|\mathrm{c})p_{\mathrm{c}}\big]p_{\mathrm{c}}^{M_{\min}}\Big), \\
p_{(\mathrm{b3},2|dd)}p_{\mathrm{click}}(\mathrm{D_{M2}}|dd,\mathrm{b3},2) &= \frac{q_{\mathrm{f}}\gamma}{\Theta}p_{(\mathrm{b3},2|dd)}p_{\mathrm{click}}(\mathrm{D_{M1}}|dd,\mathrm{b3},2). \qquad (225)
\end{aligned}
$$

And the final case for "$dd$" is type "b3" and Position 4, for which we obtain

$$
\begin{aligned}
p_{(\mathrm{b3},4|dd)}p_{\mathrm{click}}(\mathrm{D_{M1}}|dd,\mathrm{b3},4) &= \frac{p_{|0\rangle}q_{\mathrm{f}}q_{\mathrm{p}}\Theta\big[1-p(\neq 0|\mathrm{c})\big]}{p(\neq 0|\mathrm{c})^2p_{\mathrm{c}}\big[1-p(\neq 0|\mathrm{c})p_{\mathrm{c}}\big]^2} \\
&\times\Bigg\{[p(\neq 0|\mathrm{c})p_{\mathrm{c}}]^{M_{\max}}\Big(p(\neq 0|\mathrm{c})p_{\mathrm{c}}\big[M_{\max}-2\big]-M_{\max}+1\Big) \\
&+p(\neq 0|\mathrm{c})^3p_{\mathrm{c}}^3\big[2-p(\neq 0|\mathrm{c})p_{\mathrm{c}}\big]\Bigg\}, \\
p_{(\mathrm{b3},4|dd)}p_{\mathrm{click}}(\mathrm{D_{M2}}|dd,\mathrm{b3},4) &= \frac{q_{\mathrm{f}}\gamma}{\Theta}p_{(\mathrm{b3},4|dd)}p_{\mathrm{click}}(\mathrm{D_{M1}}|dd,\mathrm{b3},4), \qquad (226)
\end{aligned}
$$

if $M_{\min}=2$ and $M_{\max}\geq 5$, and

$$
\begin{aligned}
p_{(\mathrm{b3},4|dd)}p_{\mathrm{click}}(\mathrm{D_{M1}}|dd,\mathrm{b3},4) &= \frac{p_{|0\rangle}q_{\mathrm{f}}q_{\mathrm{p}}\Theta\big[1-p(\neq 0|\mathrm{c})\big]p(\neq 0|\mathrm{c})}{p_{\mathrm{c}}[1-p(\neq 0|\mathrm{c})p_{\mathrm{c}}]^2} \\
&\times\Big(p_{\mathrm{c}}^{M_{\max}}p(\neq 0|\mathrm{c})^{M_{\max}-M_{\min}}\Big[p(\neq 0|\mathrm{c})p_{\mathrm{c}}\,(M_{\max}-M_{\min}+1)-M_{\max}+M_{\min}-2\Big]+\big[2-p(\neq 0|\mathrm{c})p_{\mathrm{c}}\big]p_{\mathrm{c}}^{M_{\min}}\Big), \\
p_{(\mathrm{b3},4|dd)}p_{\mathrm{click}}(\mathrm{D_{M2}}|dd,\mathrm{b3},4) &= \frac{q_{\mathrm{f}}\gamma}{\Theta}p_{(\mathrm{b3},4|dd)}p_{\mathrm{click}}(\mathrm{D_{M1}}|dd,\mathrm{b3},4), \qquad (227)
\end{aligned}
$$

when $M_{\min}>2$ and $M_{\max}\geq M_{\min}+3$.

## VI. COMPARISON WITH THE EXPERIMENTS

In this Section, we provide the experimental parameters of the long-distance implementations of the COW protocol reported in [21, 22], as well as those presented in [23, 24]. Also, we discuss in more detail how the achievable visibilities of Eve's attack have been optimized in the high gain region when comparing with the experimental implementations.

Since we plot the visibilities and the QBER as a function of the gain at Bob's side (*i.e.,* the probability to have a click in the data line per signal state sent by Alice), and in [21–24] this value is not given explicitly, we provide the formula used to calculate the gain from the experimental parameters. In particular, we have that

$$
\mathrm{Gain}=1-(1-p_{\mathrm{d}})\big[(1-f)e^{-\mu t_{\mathrm{B}}\eta_{\mathrm{D}}\eta_{\mathrm{ch}}}+fe^{-2\mu t_{\mathrm{B}}\eta_{\mathrm{D}}\eta_{\mathrm{ch}}}\big], \qquad (228)
$$

where $p_{\mathrm{d}}$ is the dark count rate per signal of the detector $\mathrm{D_d}$ in the data line, $f$ is the probability that Alice sends a decoy state, $\mu=|\alpha|^2$ is the mean photon number of Alice's pulses, $t_{\mathrm{B}}$ is the transmittance of Bob's beamsplitter, $\eta_{\mathrm{D}}$ is the detection efficiency of $D_{\mathrm{d}}$ and $\eta_{\mathrm{ch}}$ is the channel transmittance, which can be written as $10^{-\alpha_{\mathrm{att}}L/10}$, where $\alpha_{\mathrm{att}}$ is the attenuation of the optical fiber in dB/km and $L$ is the length of the fiber in km. Eq. (228) can be interpreted as calculating the probability of not having a click at all in the data line and subtracting this from probability 1. The quantity $e^{-\mu t_{\mathrm{B}}\eta_{\mathrm{D}}\eta_{\mathrm{ch}}}$ is the probability that a coherent pulse of intensity $\mu t_{\mathrm{B}}\eta_{\mathrm{D}}\eta_{\mathrm{ch}}$ does not produce a click in a perfect detector. Note that in Eq. (228) we have taken into account that double clicks in the detector $D_{\mathrm{d}}$ are not discarded by Bob but he assigns a random bit value in this case.

### A. Achievable QBER and Visibilities by the attack

To compare Eve's attack to the experiments, first, we have to calculate the QBER and the visibilities which are achievable by the attack. To do this, we take a set of $q_{\rm inc}$ (the probability of having an inconclusive result) values and use the SDP defined in Section II to obtain the probabilities of having a correct (incorrect), $q_{\rm s}$ ($q_{\rm f}$) conclusive outcome for each $q_{\rm inc}$ value. Note that this only depends on the mean photon number of Alice's pulses $\mu$. An example can be seen in Fig. 19 for two different $\mu$ values.

Then, given the formulas of the gain, the QBER and the visibilities presented in Sections III, IV and V, and the parameters of Eve's attack, we obtain the QBER and the different visibilities as a function of the gain produced by the attack. We note that the higher $q_{\rm inc}$ is, the lower the gain is in the attack, however, certain values of the parameters of the attack can further decrease the gain.

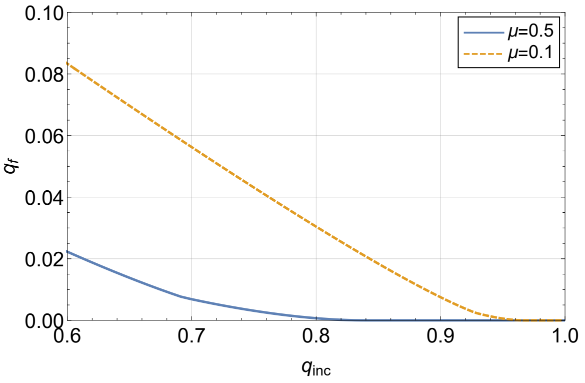


FIG. 19. The probability $q_{\rm f}$ of having an incorrect conclusive result as a function of the probability $q_{\rm inc}$ of having an inconclusive result for two different values of the mean photon number of Alice's pulses.

Note that in Fig. 19, one can observe, as we have already pointed out in the main text, that higher $\mu$ puts Eve into a better situation as USD can be performed until a lower value of $q_{\rm inc}$ (*i.e.,* higher gain). Moreover, one can confirm, as it has been observed in Fig. 3 of the main text, that allowing the QBER (visibilities $V_s$ with $s \in \mathcal{S}$) to be below (above) a certain threshold value $Q^{\rm th}$ ($V^{\rm th}$) does not help much in increasing the gain value from which the protocol is secure when $\mu$ is too low. This is so because for smaller $\mu$ the transition from the USD regime is much sharper, therefore there is a steeper decrease in the visibilities $V_s$ when leaving the perfect USD regime.

### B. Comparison with the experiments in [21]

These experiments perform key exchanges in the laboratory over fiber lengths ranging from 100 to 250 km with secret bit rates from 6 kbits/s to 15 bits/s, respectively. The QBER values range from 0.85% to 1.9%, respectively. We have taken the precise values of the QBER from a graphic in [21], which means that the precision is around 0.1%. They are given in Table II. The maximum and the minimum visibilities range from 0.92 to 0.95. Other experimental parameters are listed in Table III.

| Distance[km] | 100 | 150 | 200 | 250 |
|---|---|---|---|---|
| $\log_{10}$(Gain) | -3.54 | -4.36 | -5.18 | -6.15 |
| QBER[%] | 0.85 | 1.5 | 2 | 1.9 |

TABLE II. A summary of the distances (with the corresponding gain values) and the achieved QBERs in the experiments in [21]. The visibility values fall in the interval $[0.92, 0.95]$.

For the 250 km link, the total channel loss is 42.6 dB, while for the 100, 150 and 200 km links the average fiber attenuation is $\alpha_{\rm att} = 0.164\,{\rm dB/km}$. These are the values that we used to calculate the gain by means of Eq. (228). The calculated gain values, used in Fig. 2(a) of the main text, are also given in Table II. The exact values of the visibilities have not been included in [21], therefore in Fig. 2(a) of the main text we used an error bar representation because they lie in the interval $[0.92, 0.95]$.

| $\mu$ | $f$ | $t_{\rm B}$ | $p_{\rm d}$ | $\eta_{\rm D}$ | $\eta_{\rm M}$ |
|---|---|---|---|---|---|
| 0.5 | 0.0625 | 0.9 | $4\times10^{-9}$ | 0.0265 | 0.0144 |

TABLE III. Experimental parameters in [21]. Here, $\mu$ is the mean photon number of Alice's pulses, $f$ is the probability that Alice sends a decoy state, $t_{\rm B}$ is the transmittance of Bob's beamsplitter, $p_{\rm d}$ is the dark count rate per signal of Bob's detector in the data line and $\eta_{\rm D}$ ($\eta_{\rm M}$) is the detection efficiency of the detector in the data (monitoring) line.

#### 1. *Optimal parameters of the attack*

Since the experimental implementations in [21] monitor the QBER and all the visibilities $V_s$ with $s \in \mathcal{S}$, our task is to maximize the minimum of all the visibilities produced by Eve's attack while minimizing the QBER for each value of the gain, which we do numerically.

Below we present the parameters $M_{\rm min}$, $M_{\rm max}$, $q$, $q_{\rm p}$ and $\beta$ of the attack (see Section I for a detailed description of these parameters) that we use to obtain the results shown in Fig. 2(a) of the main text. We note that the observations below remain valid also for the experiments in [22], though, there Eve maximizes the average visibility $V_{\rm ave}$.

In particular, we fix $M_{\rm min} = 2$ and $M_{\rm max} = 10$ throughout the simulations. Eve has to set $M_{\rm min}$ as low as possible otherwise she would discard a lot of possibly correctly identified blocks of length smaller than $M_{\rm min}$. Ideally, Eve should set $M_{\rm max}$ as high as possible, however, in the gain regime that we are interested in, it is very unlikely that Eve obtains 10 or more consecutive

conclusive outcomes. So, to reduce the running time of the simulations, we fix $M_{\mathrm{max}}$ to that value.

In the perfect USD regime the optimum is obviously QBER $= 0$ and $V_s = 1$ for all $s \in \mathcal{S}$. To achieve this, $q = 1$ is required so that Eve does not discard the blocks of length $M_{\mathrm{min}}$ without trying to process them. Moreover, as here Eve does not have incorrect results it is worth having the mean photon number $|\beta|^2$ of her pulses as high as possible to make sure that the non-vacuum signals that she sends Bob actually produce a click. Setting $\beta = 2000$ is enough for this purpose as higher values of $\beta$ provide basically indistinguishable results.

Outside the perfect USD regime it is impossible to have QBER $= 0$ and $V_s = 1$ for all $s \in \mathcal{S}$, as sometimes Eve obtains an incorrect outcome. In this regime, it turns out that one has to decrease $\beta$ as this gives a chance for the incorrect signals to not reach the detectors in the monitoring line, but we cannot decrease $\beta$ too much as that would make the gain too small. The visibility $V_d$ is not affected by the border effects (*i.e.*, it does not depend on the position of the decoy signal within the block resent by Eve) as the coherence is checked inside the signal, therefore the best strategy for maximizing $V_d$ is to have $q_{\mathrm{p}} = 0$, as this gives the highest possible gain. Note that even if all the errors are resent (in this regime with $\mu = 0.5$ errors happen relatively rarely compared to having a correct outcome), $V_d$ would still be higher than in the case of $q_{\mathrm{p}} = 1$ since the errors (*i.e.*, identifying a decoy signal as a bit 0 or bit 1 signal) would have a higher probability of being resent (due to the distinguished role of the bit 0 and bit 1 in the $q_{\mathrm{p}} = 1$ case) than a correctly identified decoy signal, therefore Eve would have proportionally more errors among her non-vacuum signals besides having the gain much lower.

On the other hand, for the two-signals visibilities ($V_{01}$, $V_{0d}$, $V_{d1}$ and $V_{dd}$) there are errors coming from the borders of the blocks (which is not a problem for $V_d$) therefore it is much more advantageous to have $q_{\mathrm{p}} = 1$ as that protects against the border errors. Indeed, having $q_{\mathrm{p}} = 0$ would make $V_{01}$, $V_{0d}$, $V_{d1}$ and $V_{dd}$ much smaller than if we take $q_{\mathrm{p}} = 1$ for $V_d$ (worst case for $V_d$). This is so since outside the perfect USD regime the probability of obtaining an inconclusive result is much higher than the probability of having an incorrect outcome, therefore there are lots of errors associated with having inconclusive results due to the border effects for the two-signal visibilities. To see this, consider the following simple example: Alice sends "01" (*i.e.*, a bit 1 signal followed by a bit 0 signal) and Eve obtains "inc,1" or "0,inc", where "inc" represents obtaining an inconclusive outcome. When $q_{\mathrm{p}} = 0$ these instances are not processed so Bob's detector $D_{\mathrm{M2}}$ could click whereas it should not click at all as the sequence "01" has been sent. On the other hand, as already mentioned, for the case of $V_d$ there is no error associated with having an inconclusive result irrespective of the value of $q_{\mathrm{p}}$. This means that the optimal value of $q_{\mathrm{p}}$ is closer to 1 in this regime. Moreover, the quantity $q$ should be kept close to 1 as outside the perfect USD regime Eve often gets blocks of length of 2 signals and she cannot discard these blocks without trying to process them as that would highly decrease the gain.

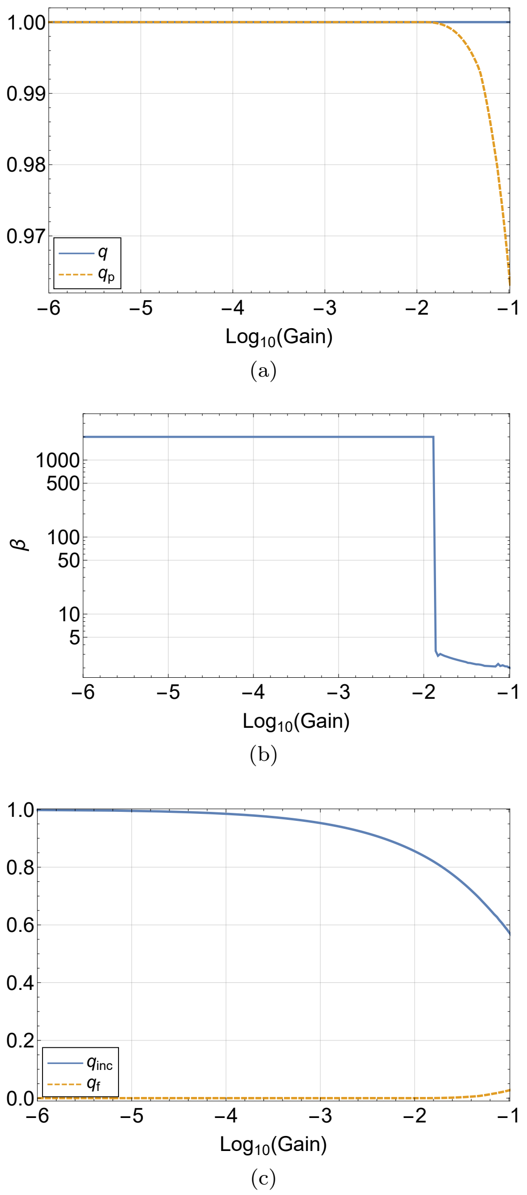


FIG. 20. The parameters of Eve's attack to obtain Fig. 2(a) in the main text. Subfigure (a) shows the parameters $q$ and $q_{\mathrm{p}}$ as a function of the gain. Subfigure (b) contains the values of the parameter $\beta$ as a function of the gain. In subfigure (c) the probabilities of having an inconclusive result ($q_{\mathrm{inc}}$) and the probability to have an incorrect outcome ($q_{\mathrm{f}}$) are shown as a function of the gain. In all cases we fix $M_{\mathrm{min}} = 2$ and $M_{\mathrm{max}} = 10$.

The values of $q$, $q_{\mathrm{p}}$ and $\beta$ obtained with the numerical optimization are shown in Fig. 20. To support the arguments above, we also include the values of $q_{\mathrm{f}}$ and $q_{\mathrm{inc}}$ as a function of the gain.

### C. Comparison with the experiments in [22]

Here the experimental implementations only monitor the QBER and $V_{\rm ave}$, whose values (together with other experimental parameters) are given in Table IV. To plot Fig. 2(b) in the main text, we consider the two experiments with the highest and the lowest $\mu$ (1st and 3rd line of Table IV) to apply the attack. For the other $\mu$ values, the $V_{\rm ave}$ and QBER curves lie between the two curves corresponding to $\mu = 0.06$ and $\mu = 0.1$ with our attack.

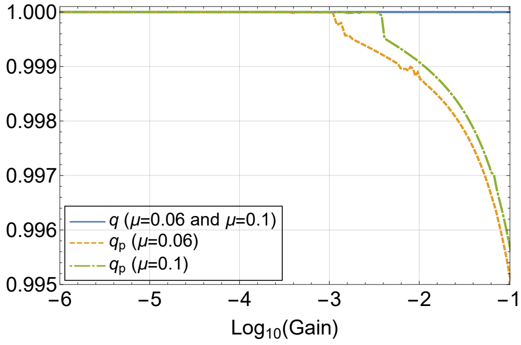


(a)

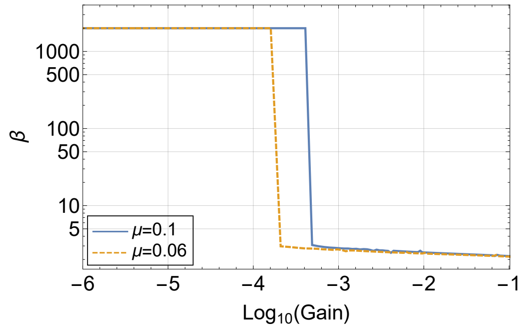


(b)

FIG. 21. The parameters of Eve's attack to obtain Fig. 2(b) in the main text. Subfigure (a) shows the parameters $q$ and $q_{\rm p}$ as a function of the gain. Subfigure (b) contains the values of the parameter $\beta$ as a function of the gain. In all cases we fix $M_{\rm min} = 2$ and $M_{\rm max} = 10$.

#### 1. *Optimal parameters of the attack*

Here Eve has to maximize the average visibility $V_{\rm ave}$ (see definition in the main text). The weights in $V_{\rm ave}$ corresponding to the different visibility components can be calculated directly from the value $f = 0.155$. In particular, we have that the weights of $s =$"01", "0$d$", "$d$1", "$dd$" and "$d$" are 0.178506, 0.0654875, 0.0654875, 0.024025 and 0.155, respectively. We can see that the four two-signal visibilities ($V_{01}$, $V_{0d}$, $V_{d1}$ and $V_{dd}$) altogether have twice as large weight as $V_d$ so it is more important for $V_{01}$, $V_{0d}$, $V_{d1}$ and $V_{dd}$ to be higher and one can allow for a smaller $V_d$. According to the observations in the previous Section we find that we should select $q_{\rm p}$ even closer to 1, which will make the visibilities $V_{01}$, $V_{0d}$, $V_{d1}$ and $V_{dd}$ larger and $V_d$ smaller, but since $V_d$ has the smallest weight in $V_{\rm ave}$ it is the most advantageous choice. The values of $q$, $q_{\rm p}$ and $\beta$ obtained with the numerical optimization are shown in Fig. 21.

### D. Comparison with the experiments in [23, 24]

Ref. [23] corresponds to the first proof-of-principle experimental demonstration of the COW protocol. For simplicity, in this implementation Alice always sends Bob the same sequence of four signal states "$|\varphi_2\rangle\,|\varphi_0\rangle\,|\varphi_1\rangle\,|\varphi_0\rangle$". Since this is a proof-of-principle experiment, we shall disregard the obvious security implications that arise from the fact that Alice repeatedly sends Bob the same states. However, we note that this particular sequence of signals only allows Alice and Bob to measure a restricted set of visibilities: $V_d$, $V_{0d}$, $V_{d1}$ and $V_{01}$. When we evaluate Eve's attack, we will then consider this restricted set of visibilities for which there is experimental data.

The experimental parameters of the implementation in [23] can be found in Table V. This work only provides the minimum value of the measured visibilities, which is 0.92. Moreover, since here we are considering the untrusted device scenario, we cannot deduce from this value the effect of the dark counts and afterpulses of the detectors at Bob's side, as it is done in [23]. The QBER and visibilities that are achievable by Eve's sequential attack are showed in Fig. 22. As already mentioned in the previous paragraph, in this figure we only consider those visibilities which are actually measured in the experiment. Like in Fig. 2 in the main text, here we optimize numerically the analytical expressions that describe Eve's attack over all parameters that she controls. We find that her attack results in $V_d \approx V_{0d} = V_{d1}$. The values of $q$, $q_{\rm p}$ and $\beta$ obtained with the numerical optimization are shown in Fig. 23. Most importantly, Fig. 22 shows that Eve can achieve a QBER value (visibilities) that is (are) below (above) those reported in [23], which implies that this proof-of-principle implementation would be insecure against the sequential attack introduced in this paper.

Similarly, in Fig. 24 we illustrate the QBER and visibilities that Eve could achieve with her sequential attack against the laboratory implementations of the COW scheme reported in [24]. The experimental parameters of these implementations are given in Table VI. Using the same reasoning as above, from Fig. 24 we find that all these experiments are also insecure against a sequential attack because Eve can always achieve a QBER and visibility values that outperform those measured in the experiments. We note that [24] also reports on some field trials of the COW scheme. Using the same techniques like above, it can be shown, however, that all such field trials are also insecure, and we omit the details here for simplicity. Indeed, it is easy to demonstrate that all such field trials lie in the perfect USD regime of Eve's sequential attack, where she can achieve perfect visibilities and

| Distance[km] | Attenuation[dB] | $\mu$ | $p_{\rm d}$ | $\eta_{\rm D}$ | $\eta_{\rm M}$ | $f$ | $t_{\rm B}$ | $\log_{10}$(Gain) | $V_{\rm ave}$[%] | QBER[%] |
|---|---|---|---|---|---|---|---|---|---|---|
| 104 | 16.9 | 0.06 | $4.38 \times 10^{-7}$ | 0.22 | 0.2 | 0.155 | 0.9 | -3.55 | 98.3 | 2.4 |
| 153 | 25.7 | 0.09 | $9.36 \times 10^{-8}$ | 0.27 | 0.25 | 0.155 | 0.9 | -4.17 | 98.0 | 1.5 |
| 203 | 34.1 | 0.1 | $1.3 \times 10^{-8}$ | 0.27 | 0.25 | 0.155 | 0.9 | -4.96 | 98.1 | 1.5 |
| 256 | 42.6 | 0.095 | $2.61 \times 10^{-9}$ | 0.27 | 0.25 | 0.155 | 0.9 | -5.83 | 98.2 | 2.0 |
| 307 | 51.9 | 0.75 | $1.06 \times 10^{-9}$ | 0.22 | 0.2 | 0.155 | 0.9 | -6.95 | 96.5 | 3.5 |

TABLE IV. Experimental parameters and results for the QBER and $V_{\rm ave}$ in [22]. See the caption of Table III for the meaning of the different quantities. The attenuation only includes the channel loss. The gain has been calculated using Eq. (228).

| Attenuation[dB] | $\mu$ | $p_{\rm d}$ | $\eta_{\rm D}$ | $\eta_{\rm M}$ | $f$ | $t_{\rm B}$ | $\log_{10}$(Gain) | $V$ | QBER[%] |
|---|---|---|---|---|---|---|---|---|---|
| 5 | 0.5 | $5.4 \times 10^{-6}$ | 0.1 | 0.1 | 0.25 | $\lesssim 1$ | -1.71 | 0.92 | 5.2 |

TABLE V. Experimental parameters and results for the QBER and visibilities in [23]. See the caption of Table III for the meaning of the different quantities. The parameter $V$ denotes the minimum value of the restricted set of visibilities measured in this experiment, which are $V_d$, $V_{0d}$, $V_{d1}$ and $V_{01}$. No other visibility value is provided in [23]. The attenuation only includes the channel loss. The gain is calculated via Eq. (228).

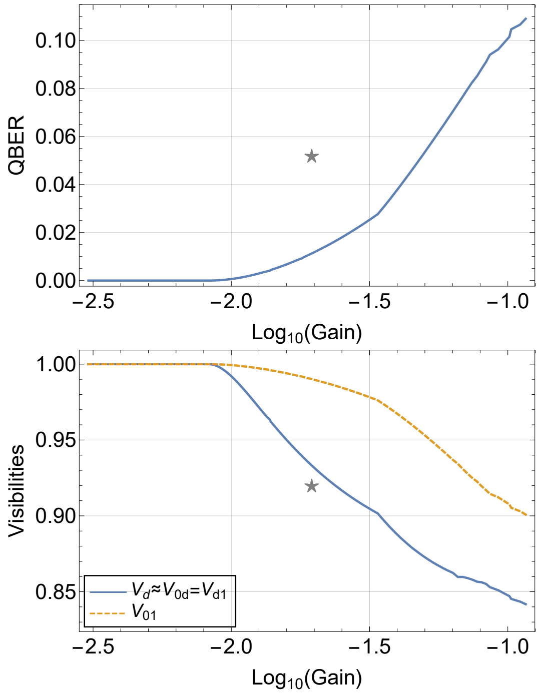


FIG. 22. QBER and visibilities versus gain at Bob's side which are achievable by the sequential attack. The stars represent experimental data from [23]. In the case of the visibilities, the star represents the only experimental value reported in [23], which is the minimum value of the four visibilities (*i.e.*, $V_d$, $V_{0d}$, $V_{d1}$ and $V_{01}$) measured in that experiment.

zero QBER.

### E. Distance limitation of experimental implementations

In the previous subsections we have seen that *all* experimental implementations of the COW protocol reported so far in the scientific literature are actually insecure. This is due to two main reasons. First, since it was believed that the COW scheme could deliver a secret key rate that scales linearly with the system's transmittance, many implementations use a mean intensity value $\mu$ for Alice's signals relatively high, say *e.g.* around 0.5, which is similar to that used in decoy-state QKD for key generation. This fact strongly limits the maximum achievable distance that is possible with the COW protocol according to the sequential attack. Second, in most experiments Bob's single-photon detectors have relatively low detection efficiency. In the untrusted device scenario considered in this paper, this latter fact further limits the transmission distance.

To illustrate these two points, in Table VII we consider the maximum achievable distance that would be possible at most by assuming that Bob uses state-of-the-art detectors with detection efficiencies 0.44 [25] and 0.93 [26], respectively. In this table we consider two possible values for the intensity $\mu$, say 0.1 and 0.5, and we evaluate two possible scenarios, depending on the values of $Q^{\rm th}$ and $V^{\rm th}$. As we can see in the table, when $\mu = 0.1$ the maximum transmission distance is limited to about 100 km, and this limit decreases further to about only 60 km when $\mu = 0.5$. As already discussed in the main text, by decreases $\mu$ one can enlarge the achievable distance, but the price to pay is a significant reduction on the key rate.

## VII. COMPARISON WITH AN UPPER BOUND AGAINST COLLECTIVE ATTACKS

In [1], the ideal scenario is assumed where all the visibilities are exactly the same, *i.e.*, $V_d = V_{01} = V_{0d} = V_{d1} = V_{dd} = V$. In such scenario, an upper bound on the key rate against collective two-pulse attacks in the limit of $\mu\eta_{\rm ch} \ll 1$, where $\eta_{\rm ch}$ represents the channel loss, is given by the formula [1]

$$K(Q,V) = \frac{1}{2}\mu\eta_{\rm ch}\eta_{\rm D}t_{\rm B}\big[1 - h(Q) - \chi(Q,V)\big], \quad (229)$$

| Attenuation[dB] | $\log_{10}$(Gain) | QBER[%] |
|---|---|---|
| 6 | -1.92 | 2.6 |
| 11 | -2.42 | 1.6 |
| 16 | -2.92 | 1.6 |
| 21 | -3.42 | 2.3 |
| 26 | -3.91 | 3.2 |
| 28 | -4.11 | 3.9 |
| 29 | -4.21 | 4.3 |
| 31 | -4.40 | 5.4 |

TABLE VI. A summary of the channel attenuations (with the corresponding gain values) and the achieved QBERs in the laboratory experiments in [24]. Other experimental parameters are common for all experiments, and are $\mu = 0.5$, $p_{\rm d} = 1.67 \times 10^{-6}$, $\eta_{\rm D} = 0.1$, $\eta_{\rm M} = 0.1$, $f = 0.0625$, and $t_{\rm B} = 0.9$. The measured visibilities satisfy $V \geq 0.95$ in all experiments. The gain is calculated via Eq. (228).

| | $\mu = 0.1$ | $\mu = 0.5$ |
|---|---|---|
| $Q^{\rm th} = 0$, $V^{\rm th} = 1$, $\eta_{\rm det} = 0.93$ | 110,4 km | 75,4 km |
| $Q^{\rm th} = 0$, $V^{\rm th} = 1$, $\eta_{\rm det} = 0.44$ | 94,2 km | 59,2 km |
| $Q^{\rm th} = 0.05$, $V^{\rm th} = 0.95$, $\eta_{\rm det} = 0.93$ | 105,9 km | 61,9 km |
| $Q^{\rm th} = 0.05$, $V^{\rm th} = 0.95$, $\eta_{\rm det} = 0.44$ | 89,7 km | 45,7 km |

TABLE VII. Illustration of the maximum achievable distance of the COW protocol as a function of the intensity $\mu$ of Alice's signals and the detection efficiency $\eta_{\rm det}$ of Bob's detectors. Particularly, we consider two state-of-the-art detectors, with detection efficiencies 0.44 [25] and 0.93 [26], respectively. The loss coefficient of the quantum channel is 0.2 dB/km. Moreover, like in the main text, we evaluate two possible sets of threshold values, $Q^{\rm th}$ and $V^{\rm th}$, for the QBER and visibilities, respectively. That is, we impose that Eve's attack simultaneously satisfies QBER$\leq Q^{\rm th}$ and $V_s \geq V^{\rm th}$ for all $s \in \mathcal{S} = \{$"$d$", "01", "0$d$", "$d$1", "$dd$"$\}$.

where $Q$ denotes the QBER, $\eta_{\rm D}$ is the detection efficiency of the detector in the data line, $t_{\rm B}$ is the transmittance of Bob's beamsplitter, the function $h$ denotes the binary entropy and $\chi(Q,V) = Q + (1-Q)h\Big([1+\xi(\mu,V)]/2\Big)$ with $\xi(\mu,V) = (2V-1)e^{-\mu} - 2\sqrt{V(1-V)(1-e^{-2\mu})}$. Eq. (229) is valid if $f \approx 0$ [1], thus for the comparison we set $f = 0.00001$. As $\mu\eta_{\rm ch} \ll 1$, $f \approx 0$ and moreover, we assume for simplicity that $p_{\rm d} = 0$, the gain given by Eq. (228) can be written as $\mu\eta_{\rm ch}t_{\rm B}\eta_{\rm D}$. To compare the sequential attack introduced in this work with the analysis in [1], we pick some typical experimental values from Table IV, for example the 1st (3rd) line corresponding to $\mu = 0.06$ ($\mu = 0.1$), where $V = 98.3\%$, $Q = 2.4\%$ and $\eta_{\rm D} = 0.22$ ($V = 98.1\%$, $Q = 1.5\%$ and $\eta_{\rm D} = 0.27$). We note, however, that the gain values included in Table IV are not valid here as a different value of $f$ is used. For the convenience of the comparison, we assume that the values $V = 98.3\%$ and $Q = 2.4\%$ ($V = 98.1\%$ and $Q = 1.5\%$) hold for all the gain values for $\mu = 0.06$ ($\mu = 0.1$). So the task is to find the maximum gain where Eve can keep all the visibilities no less than 98.3% and the QBER no higher than 2.4% (no less than 98.1% and the QBER no higher than 1.5%) since under that gain value the protocol becomes insecure against the sequential attack, as Eve can get higher $V$ and lower $Q$ than achieved in the experiment. The results can be seen in Fig. 25. This figure also includes the upper bound on the secret key rate given by Eq. (229), as a function of the gain ($\mu\eta_{\rm ch}t_{\rm B}\eta_{\rm D}$). From the results in Fig. 25, we find that the upper bound introduced in [1] can significantly overestimate the resulting secret key rate. In particular, it allows a secret key rate above $10^{-8}$ bits per pulse for gain values smaller than $10^{-7.2}$ (which corresponds to about 260 km and 280 km for $\mu = 0.06$ and $\mu = 0.1$, respectively, assuming an average channel attenuation 0.2 dB/km), while the sequential attack delivers no key rate for gain values smaller than $10^{-3.2}$ and $10^{-3.7}$ for $\mu = 0.1$ and $\mu = 0.06$, respectively (which correspond to distances around 80 km and 90 km, respectively).

## VIII. COMPARISON WITH AN UPPER BOUND DERIVED USING QUANTUM FILTERING OPERATIONS

Very recently, an attack that provides tighter upper security bounds for the COW protocol than those presented in [27] has been introduced in [2]. This attack resembles a sequential attack in the sense that Eve first performs quantum soft filtering operations [28] on each of the signals sent by Alice. In each of these operations, a signal from Alice interacts with an ancilla state which is in Eve's hands. The goal of this procedure is to probabilistically make Alice's signals more distinguishable. Then, Eve measures individually her ancilla systems and decides jointly the actual states that are resent to Bob based on her measurement results. Moreover, by combining various quantum soft filtering operations with different parameters, it is possible to preserve the detection statistics of the decoy states (*i.e.*, their percentage among the non-vacuum signals). We refer the reader to [2] for further details.

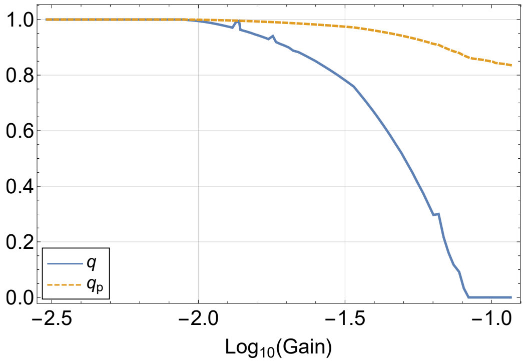


(a)

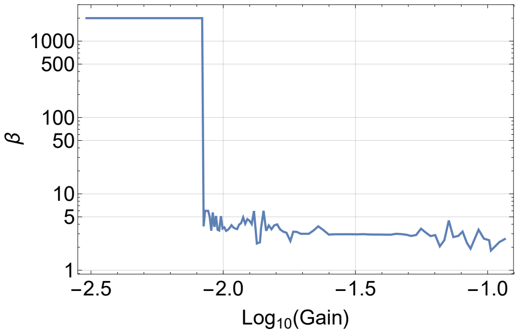


(b)

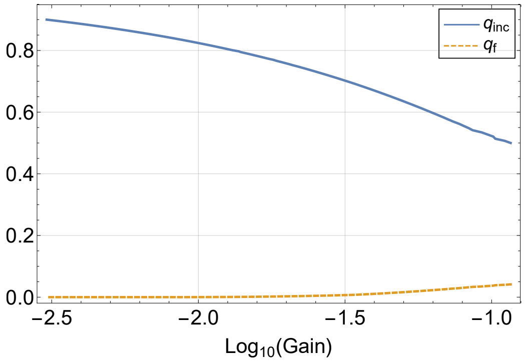


(c)

FIG. 23. The parameters of Eve's attack to obtain Fig. 22. Subfigure (a) shows the parameters $q$ and $q_{\mathrm{p}}$ as a function of the gain. Subfigure (b) contains the values of the parameter $\beta$ as a function of the gain. In subfigure (c) the probabilities of having an inconclusive result ($q_{\mathrm{inc}}$) and the probability to have an incorrect outcome ($q_{\mathrm{f}}$) are shown as a function of the gain. In all cases we fix $M_{\min} = 2$ and $M_{\max} = 10$.

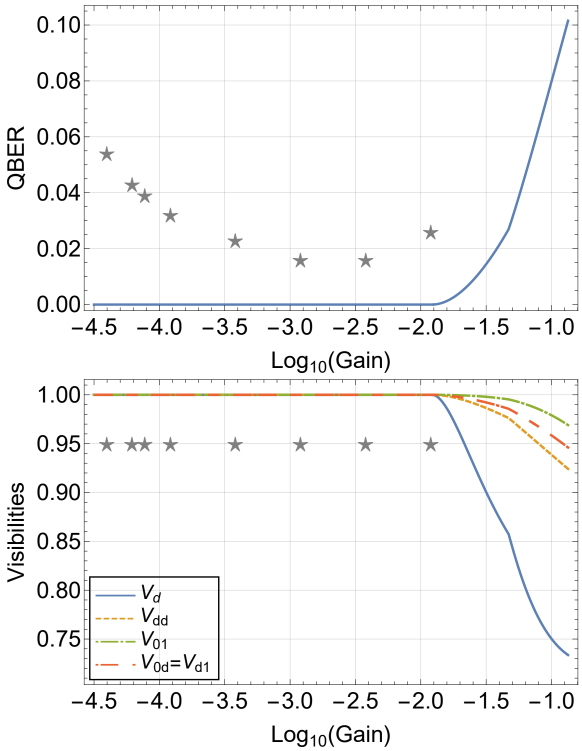


FIG. 24. QBER and visibilities versus gain at Bob's side achievable by the sequential attack. The stars represent experimental data from [24].

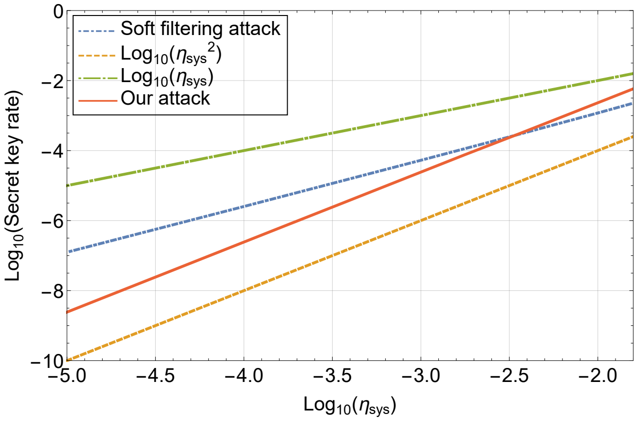


FIG. 26. Upper bounds on the secret key rate of the COW protocol as a function of the system's transmittance $\eta_{\mathrm{sys}}$ when $f = 0.1$. The dash-dotted blue line corresponds to the upper bound derived in [2], while the solid red line corresponds to the upper bound derived in this paper. For comparison, the figure includes as well the lines equal to $\eta_{\mathrm{sys}}$ (dash-dotted green line) and $\eta_{\mathrm{sys}}^2$ (dotted yellow line).

In Fig. 26 we illustrate the upper bound on the secret key rate of the COW protocol derived in [2] as a function of the system's transmittance $\eta_{\mathrm{sys}}$. For this, we use the same parameters considered in that paper, that is, we assume that the detection efficiency of the data line detector is $\eta_{\mathrm{D}} = 0.1$ and that the probability of emitting

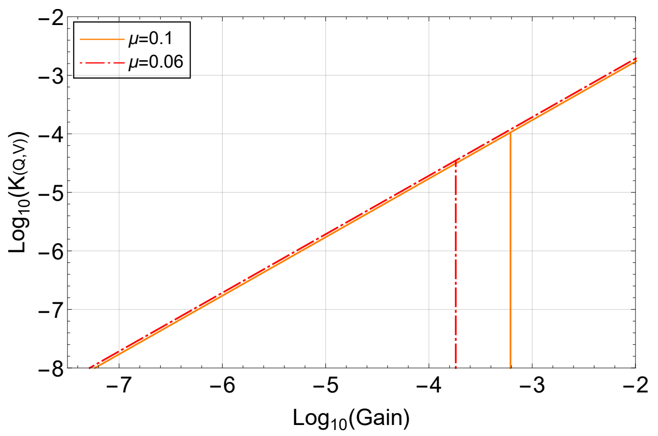


FIG. 25. Upper bound on the secret key rate introduced in [1] considering collective two-pulse attacks, as a function of the gain $\mu\eta_{\rm ch}t_{\rm B}\eta_{\rm D}$. The vertical lines represent the gain values where the protocol becomes insecure for the two different mean photon number settings according to the sequential attack introduced in this work. For the simulation of the attack we use $f = 0.00001$ and $t_{\rm B} = 0.9$.

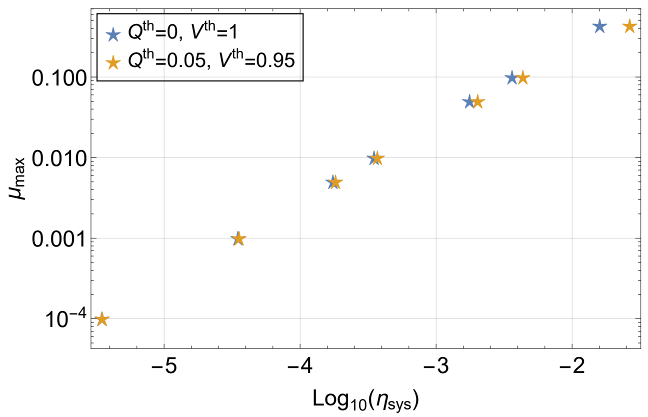


FIG. 27. The maximum intensity $|\alpha_{\rm max}(f)|^2 \equiv \mu_{\rm max}$ Alice can use such that Eve's attack cannot simultaneously satisfy QBER $\leq Q^{\rm th}$ and $V_s \geq V^{\rm th}$ for all $s \in \mathcal{S}$, as a function of the system's transmittance $\eta_{\rm sys} = \eta_{\rm ch}\eta_{\rm D}$, for the case $f = 0.155$ [22].

a decoy state is $f = 0.1$. For comparison, this figure includes as well the upper bound introduced in this paper based on sequential attacks, together with the lines $\eta_{\rm sys}$ and $\eta_{\rm sys}^2$. As shown in the figure, the upper bound in [2] has a scaling that is only slightly better than the linear scaling, while the upper bound derived in this work scales quadratically with the system's transmittance.

## IX. THE UPPER BOUND IN FIG. 3

For the simulations in Fig. 3 in the main text we assume that $t_{\rm B} = 1 - 10^{-6}$, so that Alice can obtain almost the highest secret key rate possible, as a very small fraction of the signals go to the monitoring line. The maximum values of $\mu$ that Alice can use for the threshold values $Q^{\rm th} = 0$, $V^{\rm th} = 1$ and $Q^{\rm th} = 0.05$, $V^{\rm th} = 0.95$ are shown in Fig. 27 when $f = 0.155$ [22].

As we already discussed in the context of Fig. 19, having the threshold values $Q^{\rm th} = 0.05$ and $V^{\rm th} = 0.95$ makes a difference for larger $\mu$ values only, where the $q_{\rm f}$ (as a function of $q_{\rm inc}$) curve does not leave the USD regime very sharply, in which case, allowing for the nonperfect threshold values puts Eve in a more advantageous situation as she can reach the threshold values until a higher value of the gain. Importantly, Fig. 27 demonstrates that the maximum value of $\mu$ decreases linearly with the system's transmittance $\eta_{\rm sys}$ when $f = 0.155$ [22].

Similarly, it can be shown that the slope of $\mu_{\rm max}$ as a function of $\eta_{\rm sys}$ is equal to that shown in Fig. 27 for any $f \in (0, 1)$. This implies that the secret key rate scales at best quadratically with $\eta_{\rm sys}$ for any $f \in (0, 1)$. As discussed in Sec VI, experimental implementations of the COW protocol typically use relatively small values of $f$ (say $f \lesssim 0.25$) in order to reduce the number of decoy signals sent and, thus, maximise the secret key rate. In this regime, it turns out that the upper bounds on the secret key rate almost overlap those illustrated in Fig. 3 in the main text. For instance, if we consider $f = 0.0625$ [21], the only difference with respect to Fig. 27 is that now the values of $\mu_{\rm max}$ are slightly lower than those corresponding to $f = 0.155$, and this results in upper bounds on the secret key rate that are marginally lower than those illustrated in Fig. 3 in the main text.

## X. DIFFERENTIAL-PHASE-SHIFT QUANTUM KEY DISTRIBUTION

Sequential attacks against differential-phase-shift (DPS) QKD [29–34] have been studied in the scientific literature in recent years [35–39]. Like the COW protocol, the DPS scheme is another example of distributed-phase-reference (DPR) QKD, where the receiver realizes joint coherence measurements on subsequent signals.

Precisely, in DPS QKD Alice sends Bob a train of weak coherent pulses whose phases are randomly modulated by 0 or $\pi$. That is, she sends him a random sequence of signals $|\alpha\rangle$ or $|-\alpha\rangle$. On the receiving side, Bob uses a Mach-Zehnder interferometer to measure the relative phase between every two consecutive incoming pulses. His measurement device is designed such that only one detector, say detector $D_0$ ($D_1$) may "click" when the relative phase between two pulses is 0 ($\pm\pi$). Once the quantum communication phase of the protocol concludes, Bob informs Alice about the time slots where he obtained a detection "click", but he does not announce the particular detector which actually fired. Also, he assigns a bit value "0" ("1") to the detection "clicks" in $D_0$ ($D_1$). In doing so, and assuming for the moment an ideal noiseless scenario, both Alice and Bob can obtain an identical string of bits which represents the sifted key.

The security of DPS QKD has been analysed in various works. For instance, Refs. [1, 35] showed that its secret key rate can scale linearly with the system's transmittance, $\eta_{\rm sys}$, if one assumes particular types of individual and collective attacks, respectively. More recently, its security against general attacks have been proven in [40, 41]. These latter works assume, however, block-wise phase randomization, and demonstrate a lower bound on the secret key rate that scales either quadratically with $\eta_{\rm sys}$, or, if the QBER is sufficiently small, with order $O(\eta_{\rm sys}^{3/2})$. Also, security bounds for a variant of the DPS scheme recently introduced in [44] have been obtained in [42, 43]. These results show an almost linear scaling of the secret key rate with $\eta_{\rm sys}$.

An essential difference between DPS and COW is that the former does not contain vacuum signals that break the coherence between adjacent pulses. This means that any sequential attack against DPS QKD necessarily introduces errors and decreases the resulting visibility. Note that, if a vacuum pulse precedes or follows a weak coherent pulse, this can always produce an error at Bob's side when both pulses interfere. This strongly contrasts with the case of the COW protocol where, as we have already seen in the main text, thanks to the presence of vacuum signals, Eve can achieve zero QBER and perfect visibilities with her sequential attack even when the overall system loss is relatively small. This is the principal reason why sequential attacks are much more effective against COW than against DPS.

In Fig. 28 we show an upper bound on the achievable secret key rate of the DPS scheme, which we have derived using a simplified version of the sequential attack introduced in the main text (against the COW protocol) more suitable for DPS QKD. In particular, to obtain this upper bound we assume that Eve first measures all the signals sent by Alice with an optimal USD measurement that discriminates the states $|\alpha\rangle$ and $|-\alpha\rangle$. Next, she groups her results in blocks of length $M$. If the number $S$ of consecutive successful measurement results within a block satisfies $S \geq M_{\rm min}$, with $\lfloor M/2+1 \rfloor \leq M_{\rm min} < M$ (to guarantee that each block of length $M$ has at most one subblock containing $M_{\rm min}$, or more, consecutive successful results), she sends Bob a train of signals. Otherwise, she sends Bob $M$ vacuum states. Precisely, if $S = M_{\rm min}$ then with probability $1-q$ she sends Bob $M$ vacuum signals, and with probability $q$ she sends him a subblock of $S$ strong coherent states (that correspond to those signals successfully identified by her measurement) together with $M-S$ vacuum signals (that correspond to those signals where Eve obtained an inconclusive measurement result). On the other hand, if $S > M_{\rm min}$, Eve directly sends Bob a subblock with $S$ strong coherent states, corresponding to those signals successfully identified by her measurement, together with $M-S$ vacuum states (for the inconclusive results). Indeed, this attack resembles that introduced in [36].

As we can see in Fig. 28, the scaling of the upper bound on the secret key rate depends on the maximum tolerable QBER, $Q^{\rm th}$, that Eve is allowed to produce with her sequential attack. In this sense, this effect is similar to what has been observed in [40, 41] when deriving lower bounds on the key rate of DPS, where the resulting scaling depends on the observed QBER. For illustration purposes, in this figure we consider two cases, $Q^{\rm th} = 0.02$ and $Q^{\rm th} = 0.1$. The higher the value of $Q^{\rm th}$ is, the more the key rate deviates from order $O(\eta_{\rm sys})$.

We note as well that the sequential attack against DPS described above can be improved further as follows. First, instead of grouping Eve's results in blocks of length $M$, Eve could directly send Bob non-vacuum signals whenever she obtains $S \geq M_{\rm min}$ consecutive successful results. And, second, the intensity of the coherent states that Eve sends to Bob does not need to be equal for all the signals but might depend on their position within the block. Indeed, by reducing the intensity of the non-vacuum pulses located at the edges of the blocks, Eve could reduce the QBER introduced by her sequential attack [37, 38]. These latter strategies could probably result in tighter upper bounds on the secret key rate of DPS QKD than those shown in Fig. 28. While this is definitively a very interesting question, it is beyond the scope of this paper, and we might address such analysis in future studies.

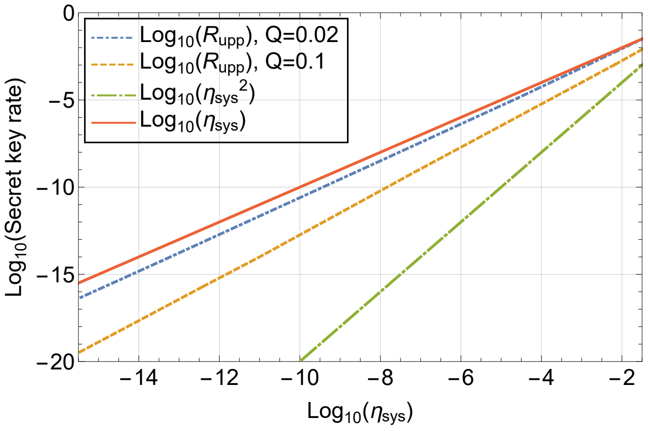


FIG. 28. Upper bound $R_{\rm upp}$ on the secret key rate of the DPS protocol [29–34] as a function of the system's transmittance $\eta_{\rm sys}$. We consider two scenarios, depending on the value of the threshold QBER, $Q^{\rm th}$. This threshold QBER represents the maximum QBER that Eve's sequential attack is allowed to cause. The case $Q^{\rm th} = 0.02$ ($Q^{\rm th} = 0.1$) is illustrated by a dash-dotted blue (dashed yellow) line. For comparison, the figure includes as well the lines equal to $\eta_{\rm sys}$ (solid red line) and $\eta_{\rm sys}^2$ (dash-dotted green line).

[1] C. Branciard, N. Gisin, and V. Scarani, New J. Phys. **10**, 013031 (2008).
[2] D. A. Kronberg, A. S. Nikolaeva, Y. V. Kurochkin, and A. K. Fedorov, Phys. Rev. A **101**, 032334 (2020).

[3] E. Waks, H. Takesue, and Y. Yamamoto, Phys. Rev. A **73**, 012344 (2006).

[4] M. Curty, L. L. Zhang, H.-K. Lo, and N. Lütkenhaus, Quant. Inf. Comp. **7**, 665 (2007).

[5] T. Tsurumaru, Phys. Rev. A **75**, 062319 (2007).

[6] M. Curty, K. Tamaki, and T. Moroder, Phys. Rev. A **77**, 052321 (2008).

[7] H. Gomez-Sousa, and M. Curty, Quant. Inf. Comp. **9**, 62 (2009).

[8] L. Vandenberghe, and S. Boyd, SIAM Rev. **38**, 49 (1996).

[9] S. Boyd, and L. Vandenberghe, *Convex Optimization* (Cambridge University Press, Cambridge, England, 2004).

[10] A. Chefles and S. M. Barnett, J. Mod. Opt. **45**, 1295 (1998).

[11] J. Fiurášek and M. Ježek, Phys. Rev. A **67**, 012321 (2003).

[12] C. W. Helstrom, *Quantum Detection and Estimation theory* (Academic Press, New York, 1976).

[13] A. Chefles, Contemporary Phys. **41**, 401-424 (2000).

[14] A. Chefles, Phys. Lett. A **239**, 339-347 (1998).

[15] A. Chefles, and S. M. Barnett, Phys. Lett. A **250**, 223-229 (1998).

[16] Y. C. Eldar, IEEE Trans. Inform. Theory **49**, 446-456 (2003).

[17] K. C. Toh, R. H. Tutuncu, and M. J. Todd, Optimization Methods and Software **11**, 545 (1999), available from http://www.math.nus.edu.sg/∼mattohkc/sdpt3.html.

[18] Jos F. Sturm, Using Sedumi 1.02, a MATLAB toolbox for optimization over symmetric cones, Optimi. Methods and Softw. **11**, 625 1999.

[19] J. Löfberg, in *Proceedings of the CACSD Conference* (Taipei, Taiwan, 2004), pp. 284-289, available from https://yalmip.github.io.

[20] Note that given $N$ linear matrix inequality (LMI) constraints $F^0(\mathbf{x}) \geq 0, \ldots, F^{N-1}(\mathbf{x}) \geq 0$, one can always combine them to form a single new LMI constraint as

$$F(\mathbf{x}) = \begin{pmatrix} F^0(\mathbf{x}) & 0 & 0 \\ 0 & \ddots & 0 \\ 0 & 0 & F^{N-1}(\mathbf{x}) \end{pmatrix} \equiv F^0(\mathbf{x}) \oplus \cdots \oplus F^{N-1}(\mathbf{x}) \geq 0, \qquad (230)$$

where the symbol $\oplus$ denotes direct sum.

[21] D. Stucki, N. Walenta, F. Vannel, R. T. Thew, N. Gisin, H. Zbinden, S. Gray, C. R. Towery, and S. Ten, New J. Phys. **11**, 075003 (2009).

[22] B. Korzh, C. C. W. Lim, R. Houlmann, N. Gisin, M. J. Li, D. Nolan, B. Sanguinetti, R. Thew, and H. Zbinden, Nat. Photonics **9**, 163 (2015).

[23] D. Stucki, N. Brunner, N. Gisin, V. Scarani, and H. Zbinden, Appl. Phys. Lett. **87**, 194108 (2005).

[24] D. Stucki, C. Barreiro, S. Fasel, J.-D. Gautier, O. Gay, N. Gisin, R. Thew, Y. Thoma, P. Trinkler, F. Vannel, and H. Zbinden, Opt. Express **17**, 13326-13334 (2009).

[25] M. Minder, M. Pittaluga, G. Roberts, M. Lucamarini, J. Dynes, Z. Yuan, and A. Shields, Nat. Photonics **13**, 334 (2019).

[26] F. Marsili *et al.*, Nat. Photonics **7**, 210 (2013).

[27] C. Branciard, N. Gisin, N. Lütkenhaus, and V. Scarani, Quant. Inf. Comput. **7**, 639 (2007).

[28] M. Curty, and N. Lütkenhaus, Phys. Rev. A **71**, 062301 (2005).

[29] K. Inoue, E. Waks, and Y. Yamamoto, *Phys. Rev. Lett.* **89**, 037902 (2002).

[30] K. Inoue, E. Waks, and Y. Yamamoto, *Phys. Rev. A* **68**, 022317 (2003).

[31] E. Waks, H. Takesue, and Y. Yamamoto, *Phys. Rev. A* **73**, 012344 (2006).

[32] H. Takesue, E. Diamanti, T. Honjo, C. Langrock, M. M. Fejer, K. Inoue, and Y. Yamamoto, *New J. Phys.* **7**, 232 (2005).

[33] E. Diamanti, H. Takesue, C. Langrock, M. M. Fejer, and Y. Yamamoto, *Opt. Express* **14**, 13073 (2006).

[34] H. Takesue, S. W. Nam, Q. Zhang, R. H. Hadfield, T. Honjo, K. Tamaki, and Y. Yamamoto, *Nat. Photonics* **1**, 343 (2007).

[35] E. Waks, H. Takesue, and Y. Yamamoto, *Phys. Rev. A* **73**, 012344 (2006).

[36] M. Curty, L. L. Zhang, H-K Lo, and N. Lütkenhaus, *Quant. Inf. Comp.* **7**, 665 (2007).

[37] T. Tsurumaru, *Phys. Rev. A* **75**, 062319 (2007).

[38] M. Curty, K. Tamaki, and T. Moroder, *Phys. Rev. A* **77**, 052321 (2008).

[39] H. Gómez-Sousa, and M. Curty, *Quant. Inf. Comp.* **9**, 62 (2007).

[40] K. Tamaki, M. Koashi, and G. Kato, preprint arXiv:1208.1995 (2012).

[41] A. Mizutani, T. Sasaki, G. Kato, Y. Takeuchi, and K. Tamaki, *Quantum Science and Technology* **3**, 014003 (2017).

[42] Y. Hatakeyama, A. Mizutani, G. Kato, N. Imoto, and K. Tamaki, *Phys. Rev. A* **95**, 042301 (2017).

[43] Z. Zhang, X. Yuan, Z. Cao, and X. Ma, *New J. Phys.* **19**, 033013 (2017).

[44] T. Sasaki, Y. Yamamoto, and M. Koashi, *Nature* **509**, 475 (2014).
